# Supplementary material for: ViDaExpert: user-friendly tool for nonlinear visualization and analysis of multidimensional vectorial data
Source: arXiv:1406.5550 ancillary file (2014-06-27)
Supplement: Supplementary file 1 [file VidaExpertPresentSh.pdf]

# VidaExpert (Visualization of DAta).

Software for multidimensional  
vectorial data visualization

# Downloads

- 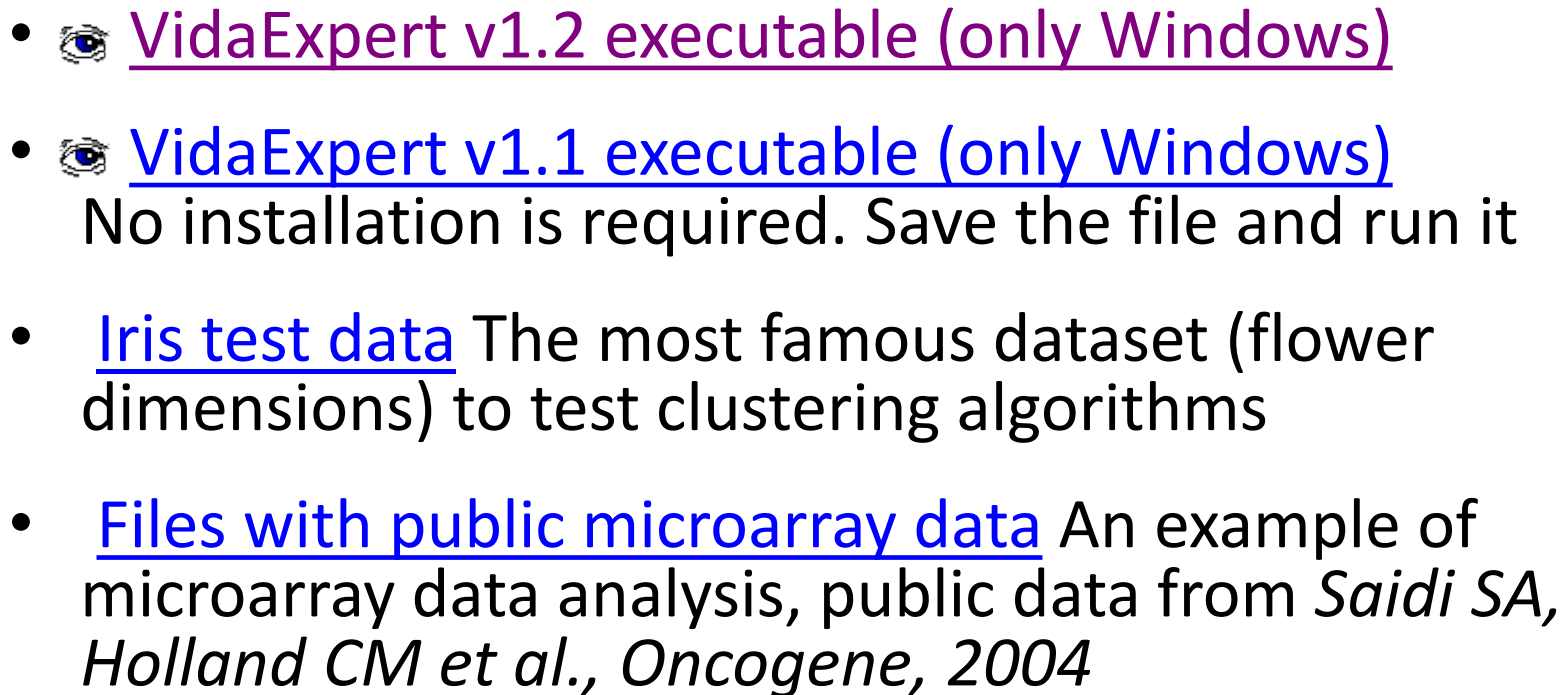 [VidaExpert v1.2 executable \(only Windows\)](#)
- 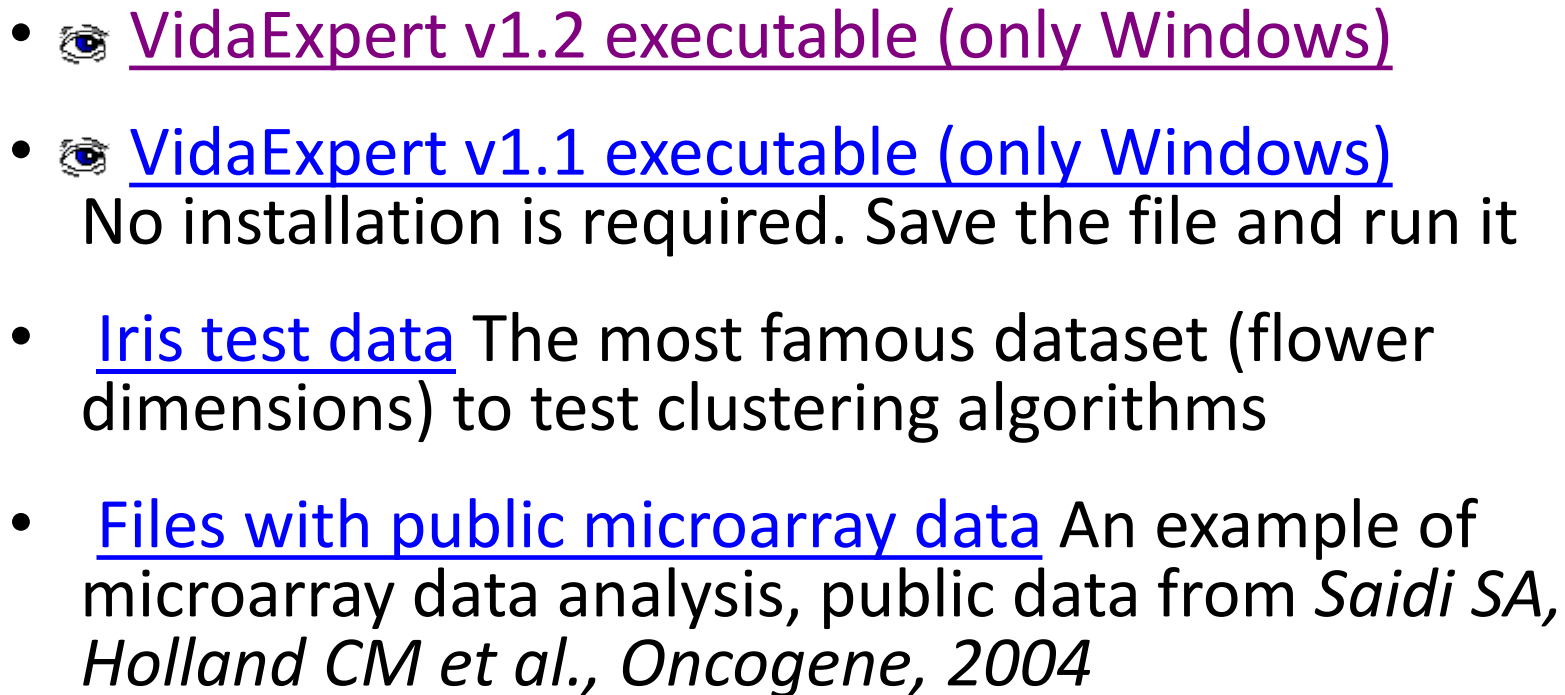 [VidaExpert v1.1 executable \(only Windows\)](#)  
No installation is required. Save the file and run it
- [Iris test data](#) The most famous dataset (flower dimensions) to test clustering algorithms
- [Files with public microarray data](#) An example of microarray data analysis, public data from *Saidi SA, Holland CM et al., Oncogene, 2004*

# Several published examples of use

- A. N. Gorban, A. Zinovyev, [Principal manifolds and graphs in practice: from molecular biology to dynamical systems](#), [International Journal of Neural Systems](#), Vol. 20, No. 3 (2010) 219–232, [arXiv:1001.1122](#) [cs.NE]
- M. Resta, [Portfolio optimization through elastic maps: Some evidence from the Italian stock exchange](#), Knowledge-Based Intelligent Information and Engineering Systems, B. Apolloni, R.J. Howlett and L. Jain (eds.), Lecture Notes in Computer Science, Vol. 4693, Springer: Berlin – Heidelberg, 2010, 635-641.
- H. Shaban, S. Tavoularis, [Identification of flow regime in vertical upward air–water pipe flow using differential pressure signals and elastic maps](#), [International Journal of Multiphase Flow](#) 61 (2014) 62-72.
- H. Failmezger, B. Jaegle, A. Schrader, M. Hülkamp, A. Tresch., [Semi-automated 3D leaf reconstruction and analysis of trichome patterning from light microscopic images](#), [PLoS Computational Biology](#), 2013, 9(4):e1003029.
- [A. Zinovyev](#), [A.N. Gorban](#), Nonlinear quality of life index, [arXiv:1008.4063](#) [cs.NE]

# VIDAEXPERT OVERVIEW

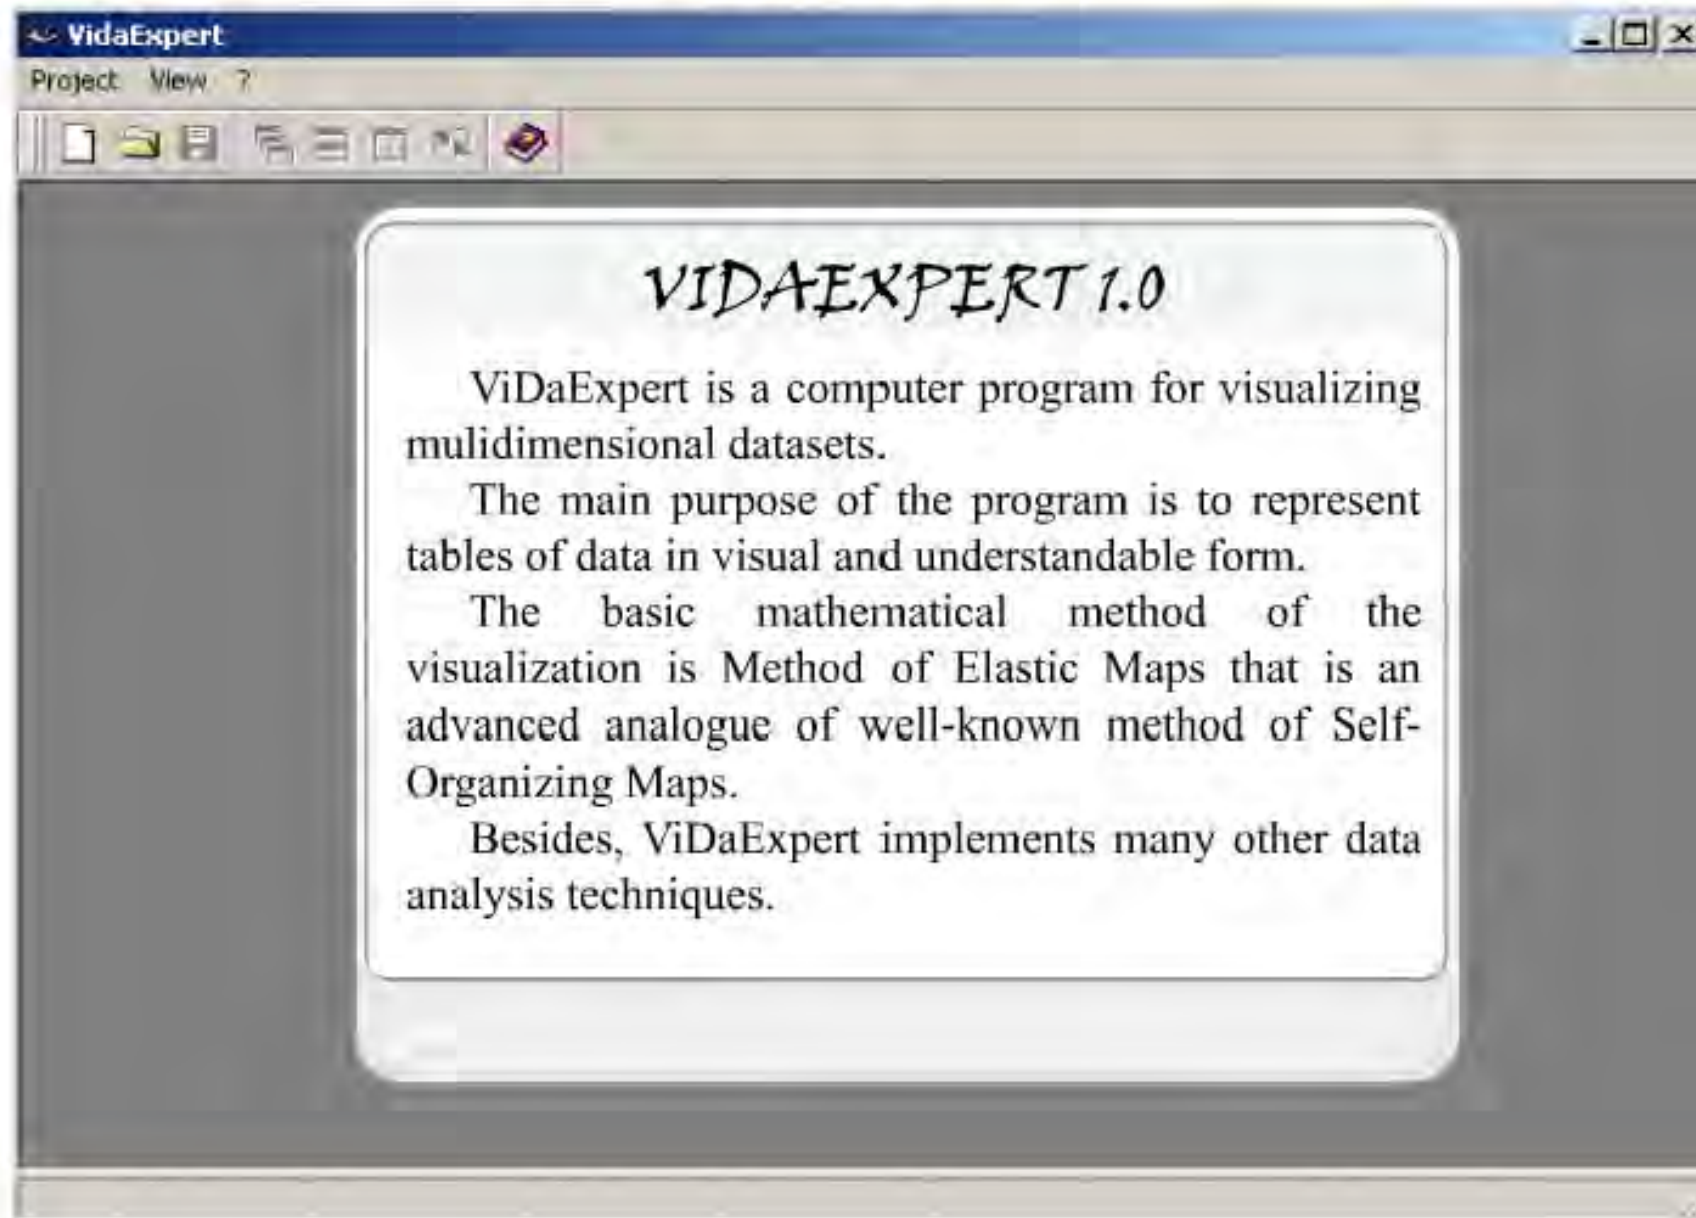

## VIDAEXPERT OVERVIEW

The screenshot displays the ViDaExpert application window. On the left, a table titled 'iris.ved' is shown with columns N2, N3, N4, and IRIS-SETOS. The table contains 8 rows of data. A dialog box titled 'Points and classes selection' is open on the right, showing options for conditional selection, random selection, and selection by color. The 'Conditional' option is selected, and the 'AND' operator is chosen. The 'Random' option is also visible, with a percentage of 100% and a checkbox for 'Including selected'. The 'Selection by color' option is also present. The 'Colors and shapes' section shows a red square for shape and fill color, and a black square for border. The 'Select' and 'Deselect' buttons are visible at the bottom of the dialog box.

|    | N2  | N3  | N4  | IRIS-SETOS  |
|----|-----|-----|-----|-------------|
| 39 | 3.4 | 1.5 | 0.2 | Iris-setosa |
| 40 | 3.5 | 1.3 | 0.3 | Iris-setosa |
| 41 | 2.3 | 1.3 | 0.3 | Iris-setosa |
| 42 | 3.2 | 1.3 | 0.2 | Iris-setosa |
| 43 | 3.5 | 1.6 | 0.6 | Iris-setosa |
| 44 | 3.8 | 1.9 | 0.4 | Iris-setosa |
| 45 | 3   | 1.4 | 0.3 | Iris-setosa |
| 46 | 3.8 | 1.6 | 0.2 | Iris-setosa |

ViDaExpert allows to work with datatables stored in popular database formats.

ViDaExpert provides many possibilities to work with a datatable: selecting records, marking records, sorting records etc. Finally every record of table is represented as a point with definite color, size and shape.



## VIDAEXPERT OVERVIEW

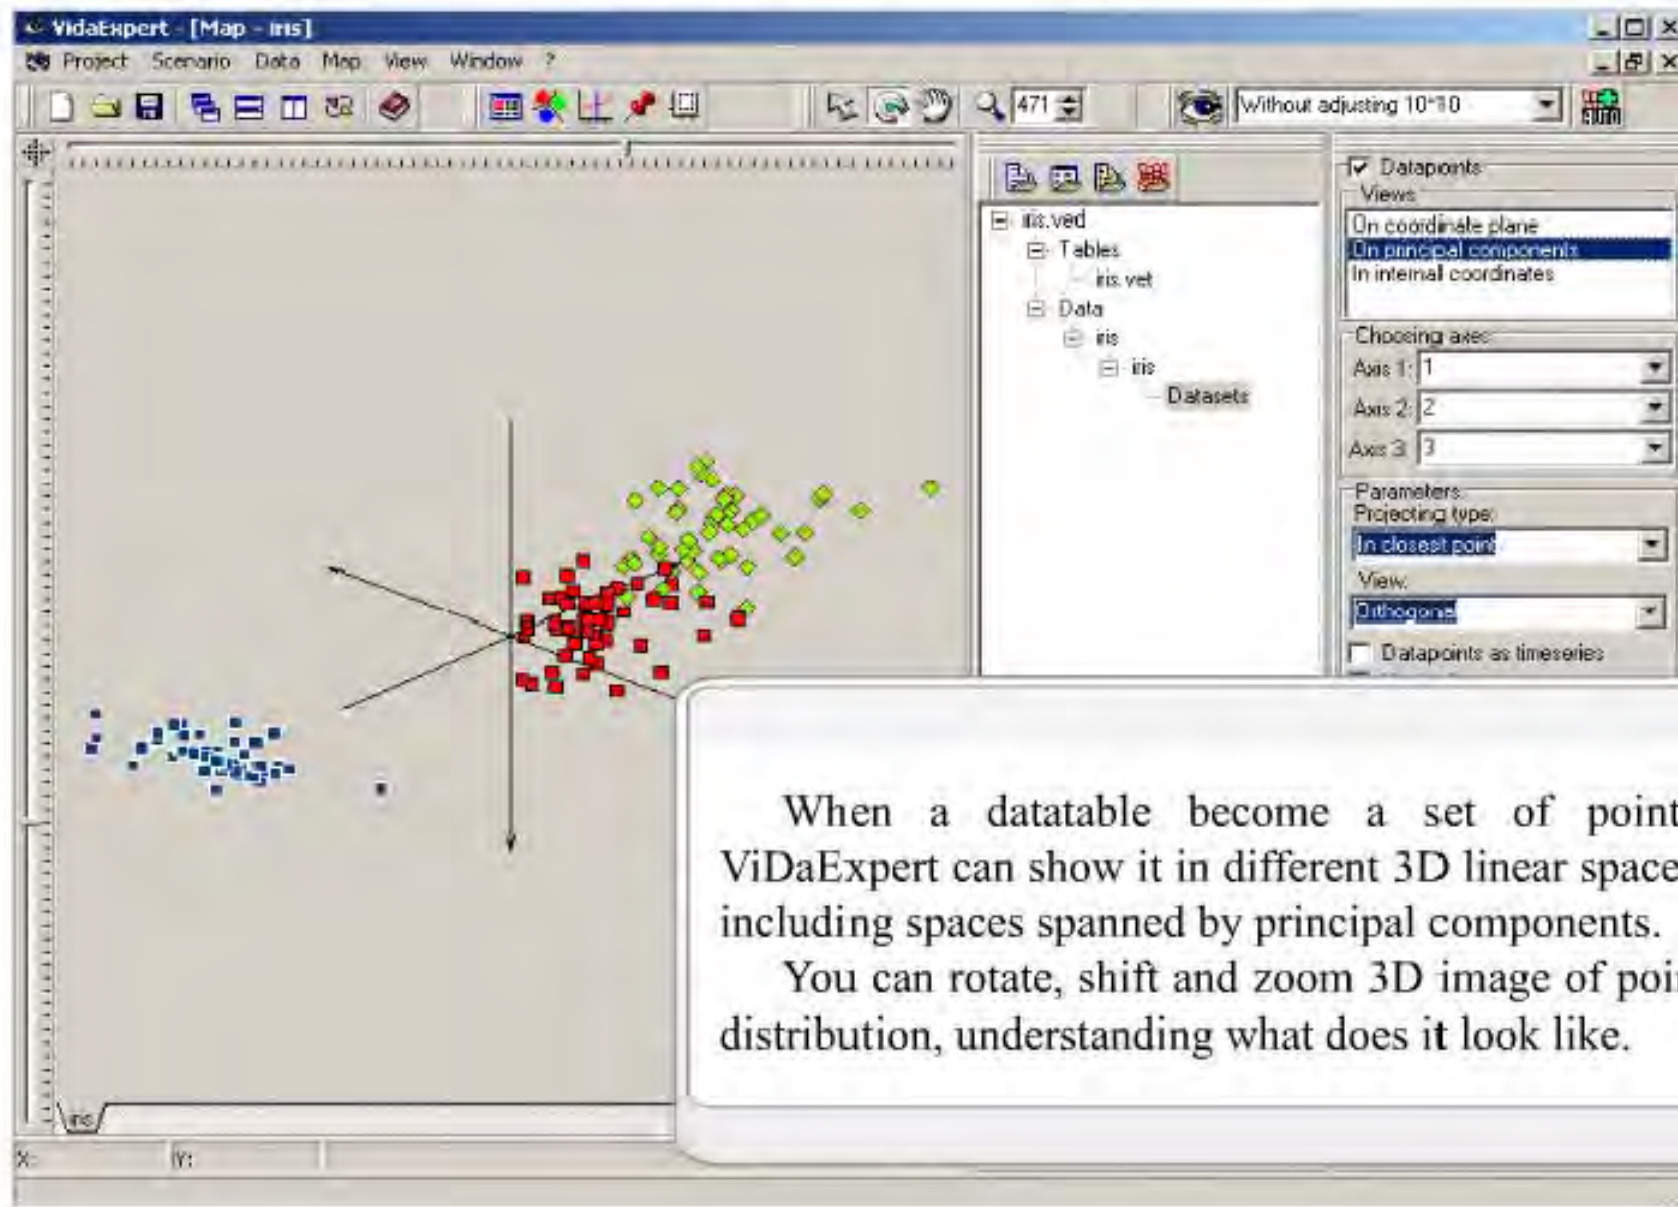

## VIDAEXPERT OVERVIEW

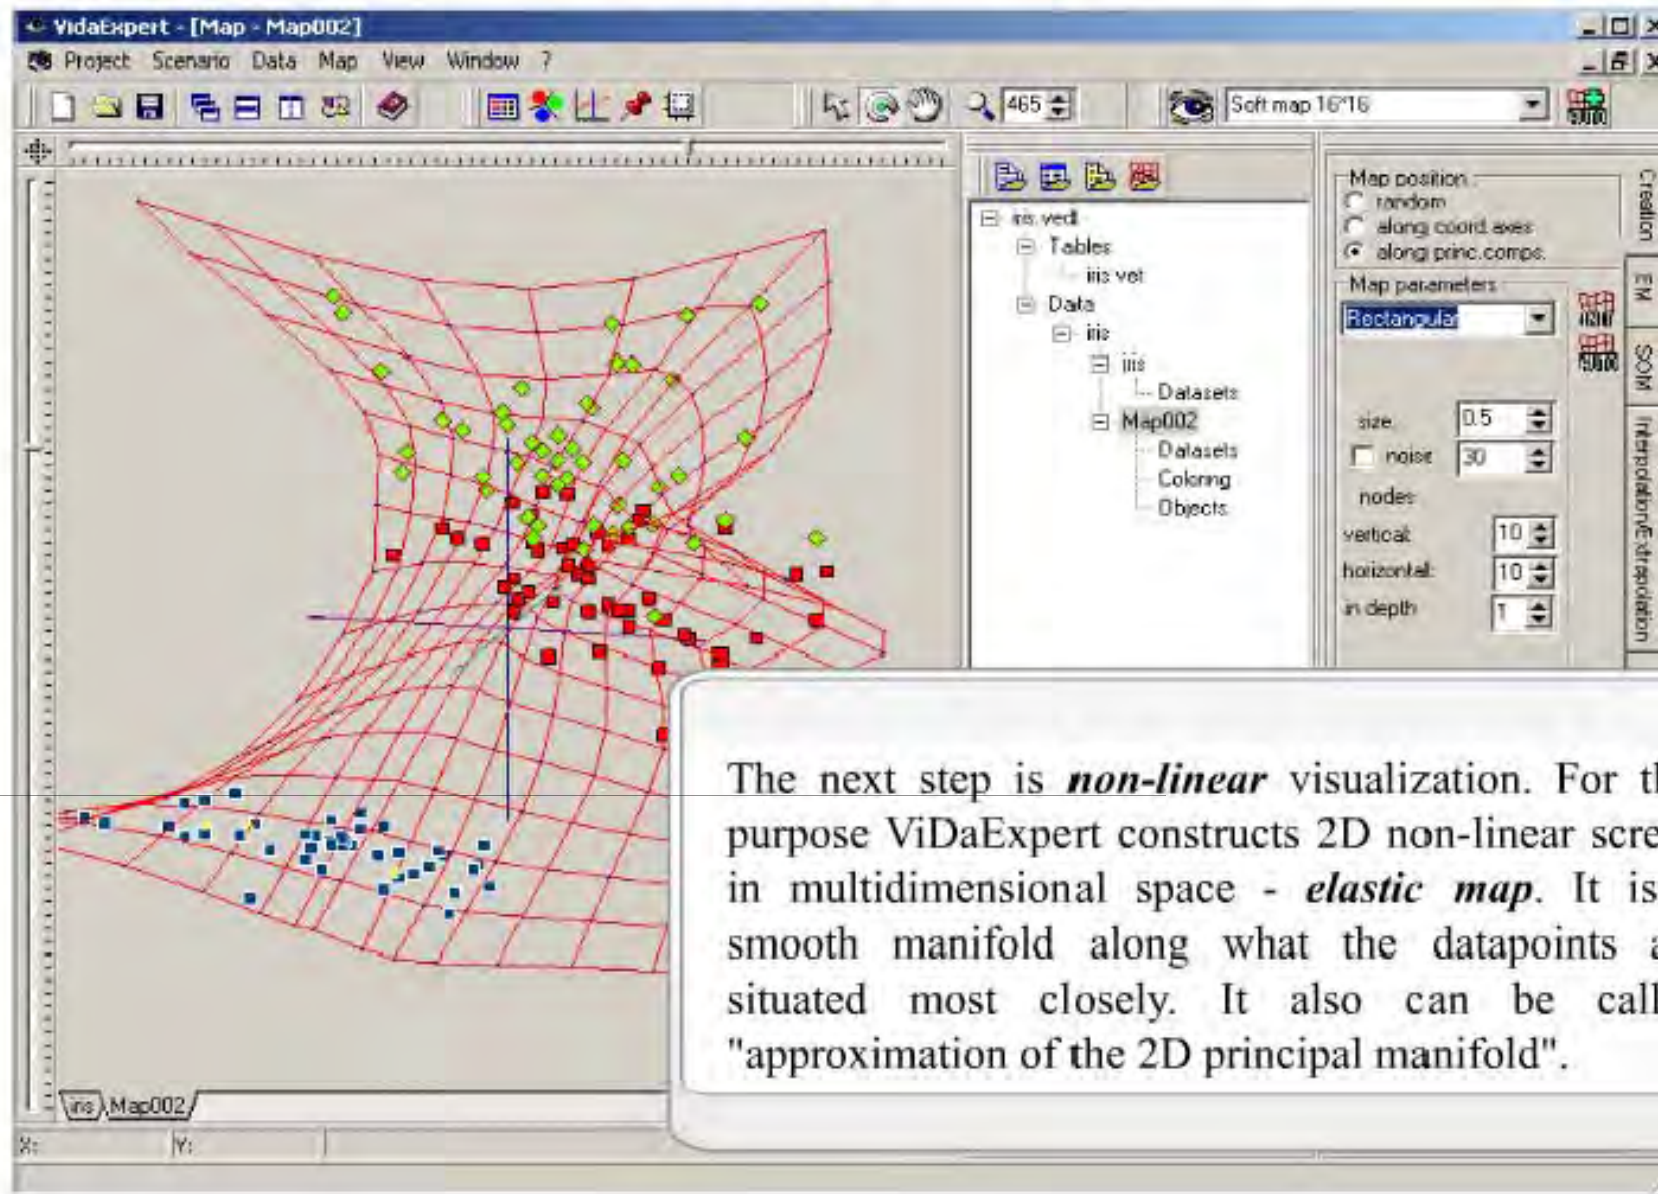



# VIDAEXPERT OVERVIEW

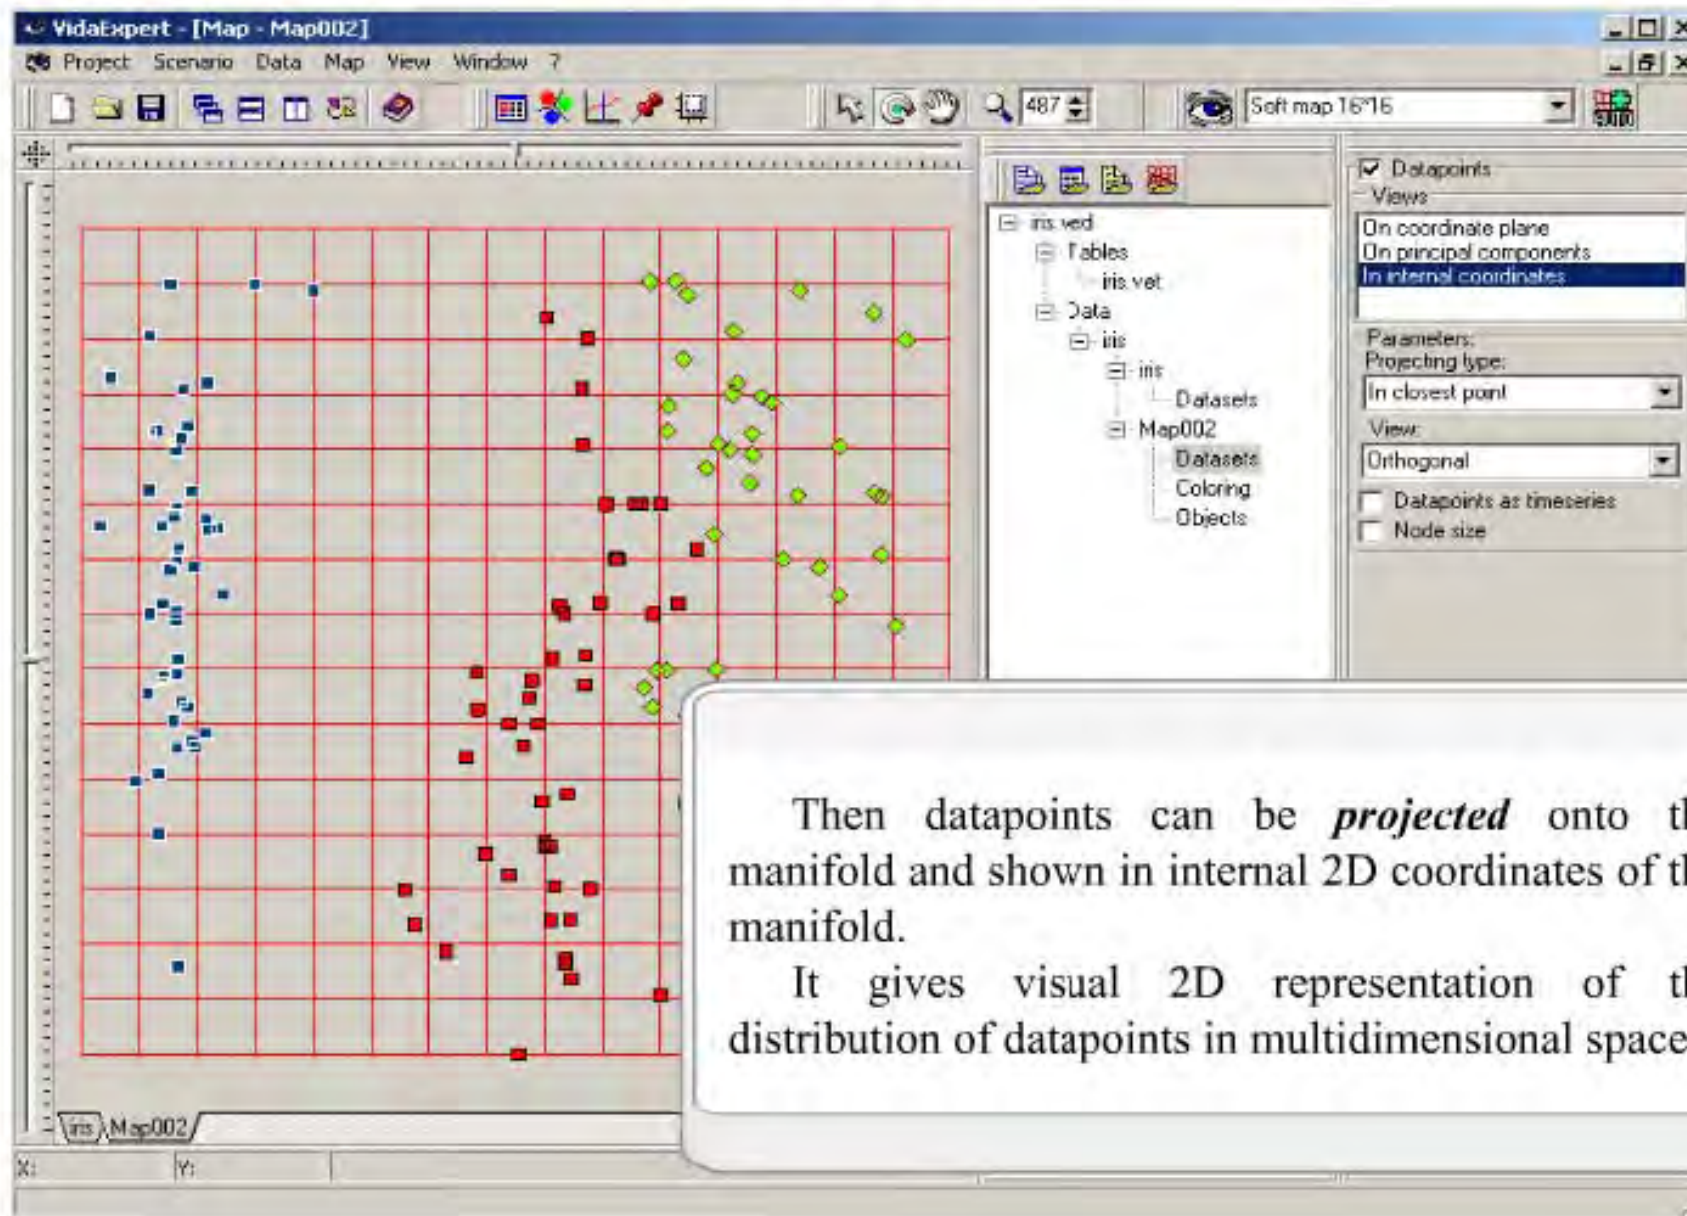



## VIDAEXPERT OVERVIEW

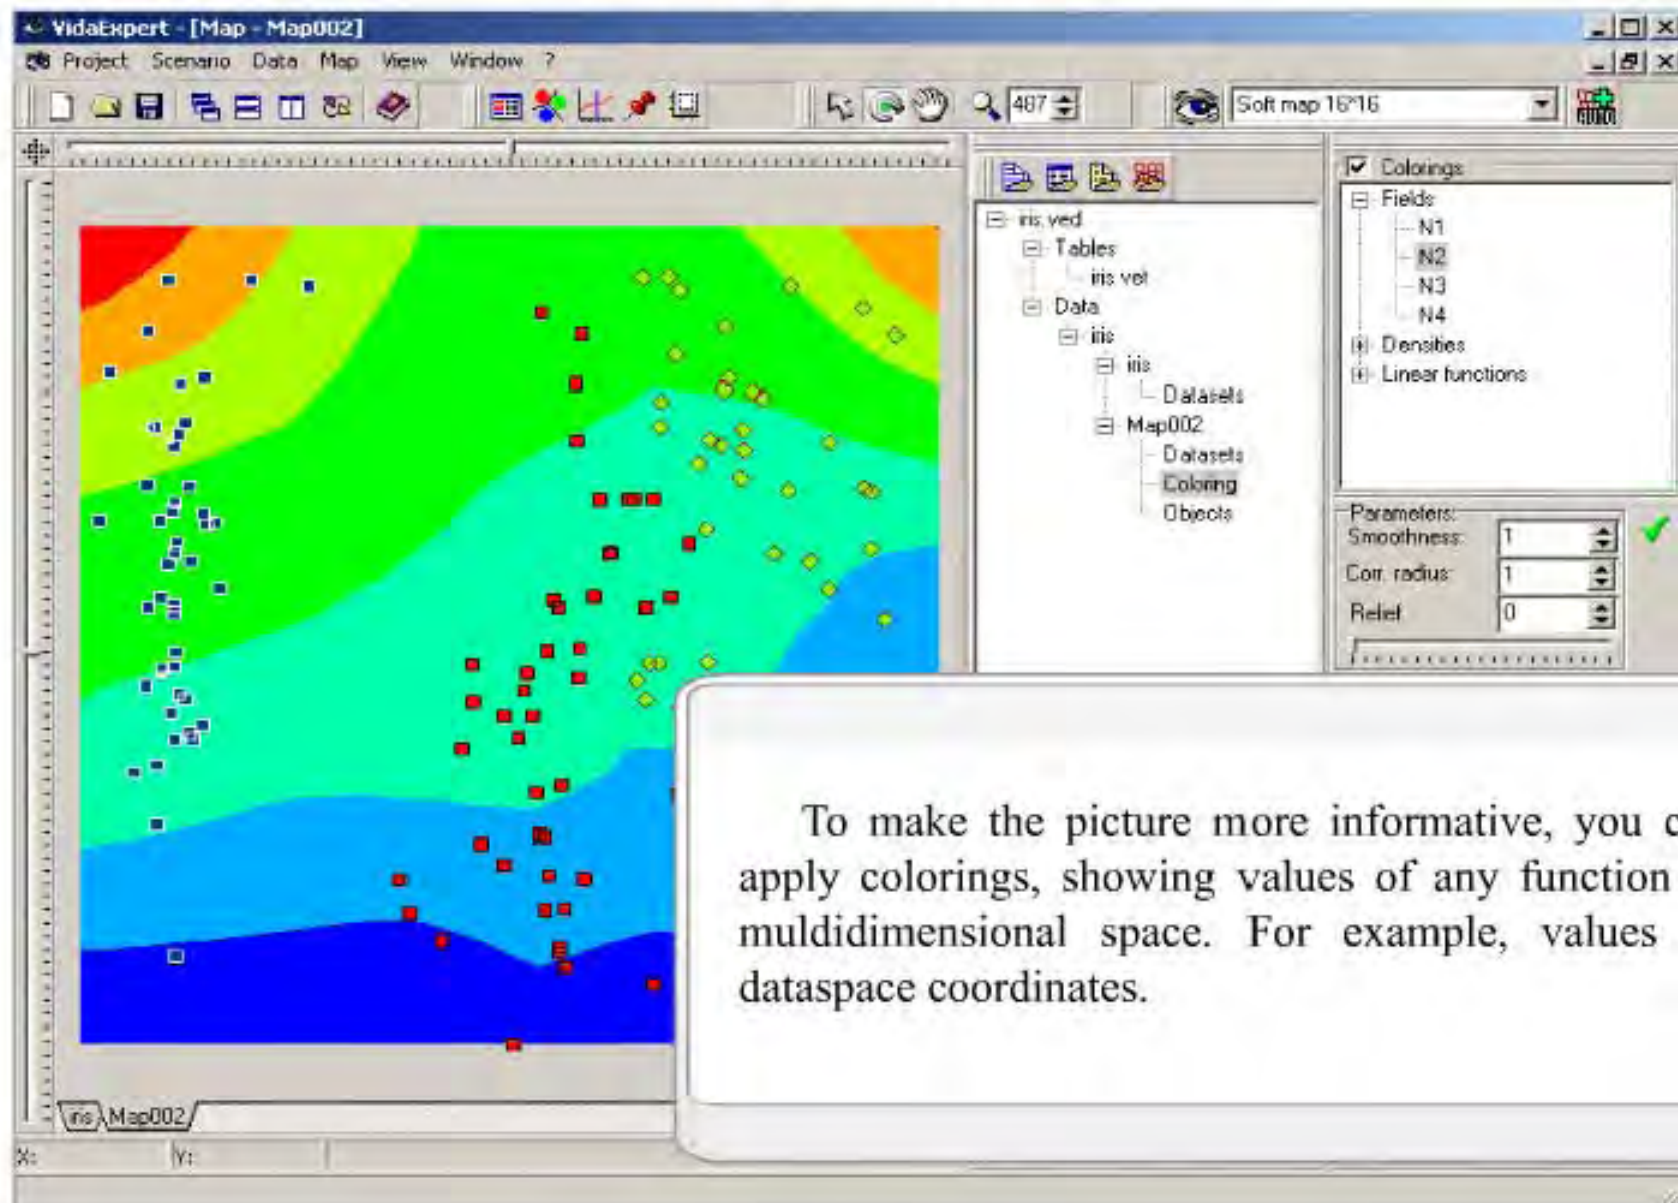

## VIDAEXPERT OVERVIEW

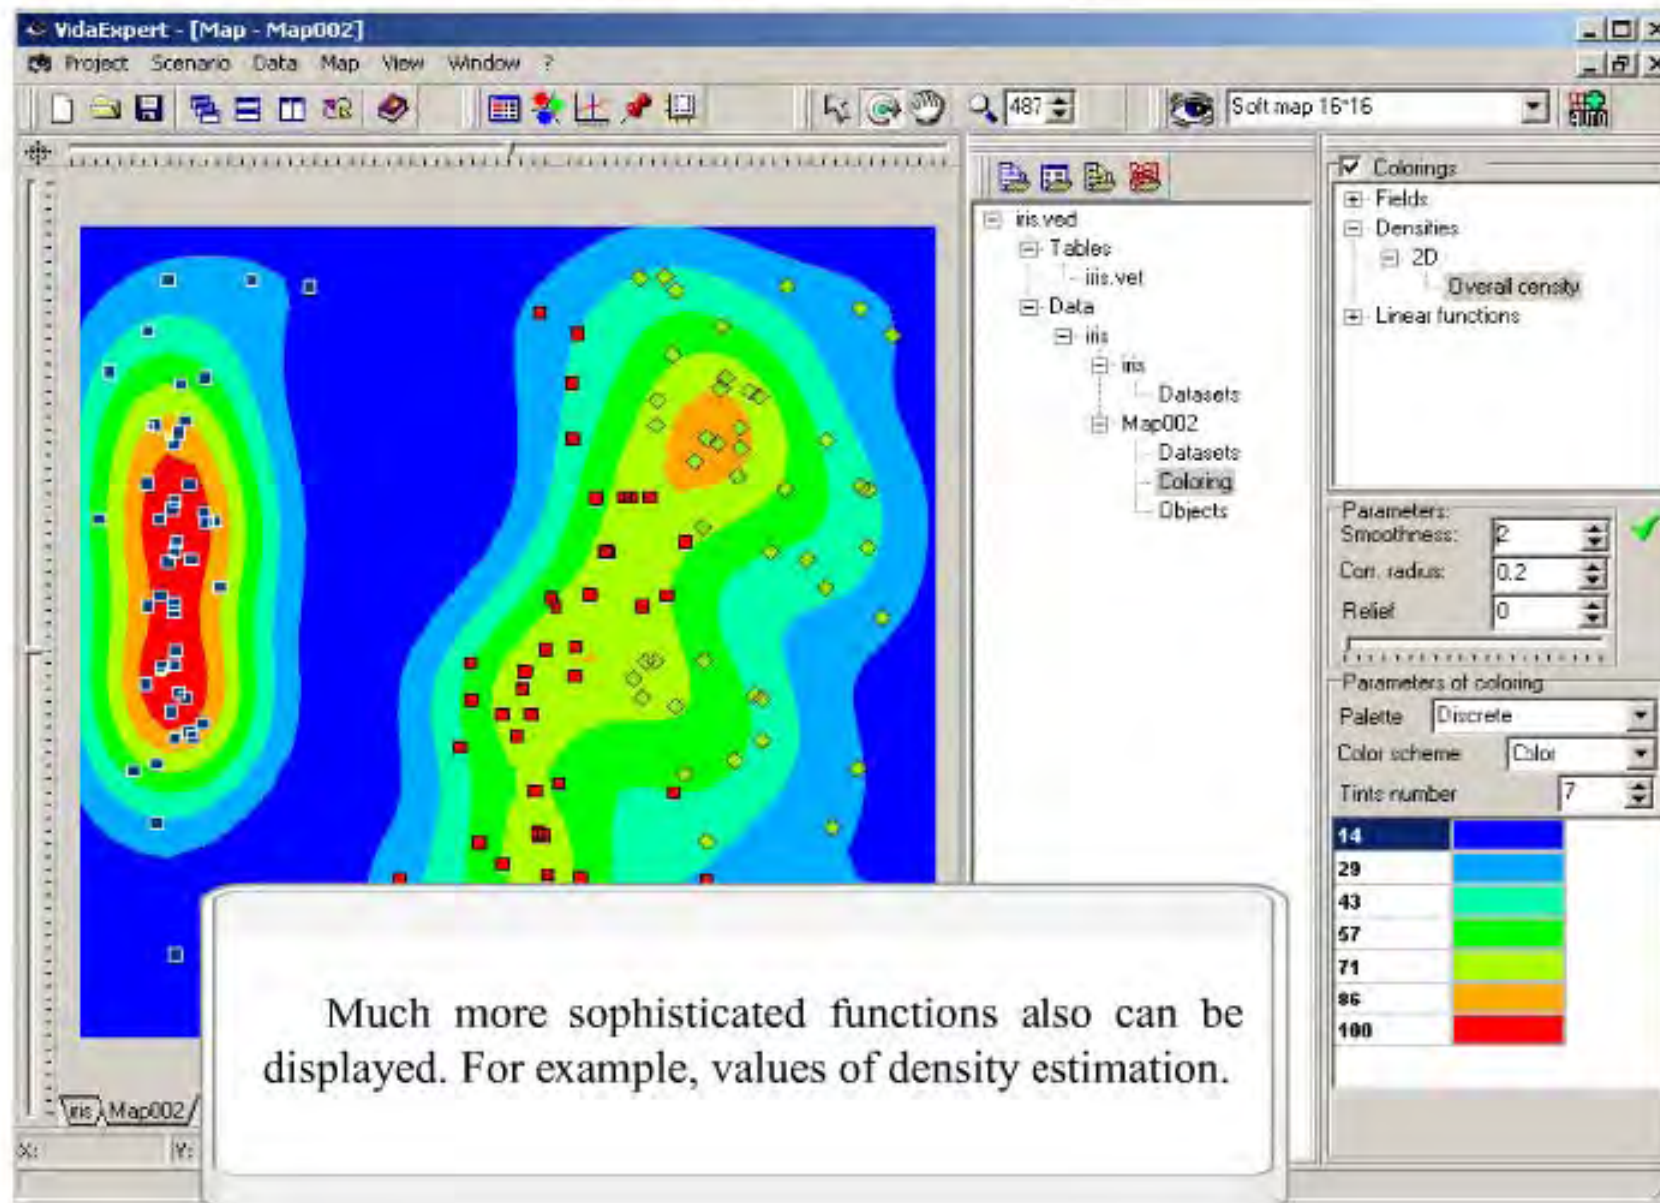



# VIDAEXPERT OVERVIEW

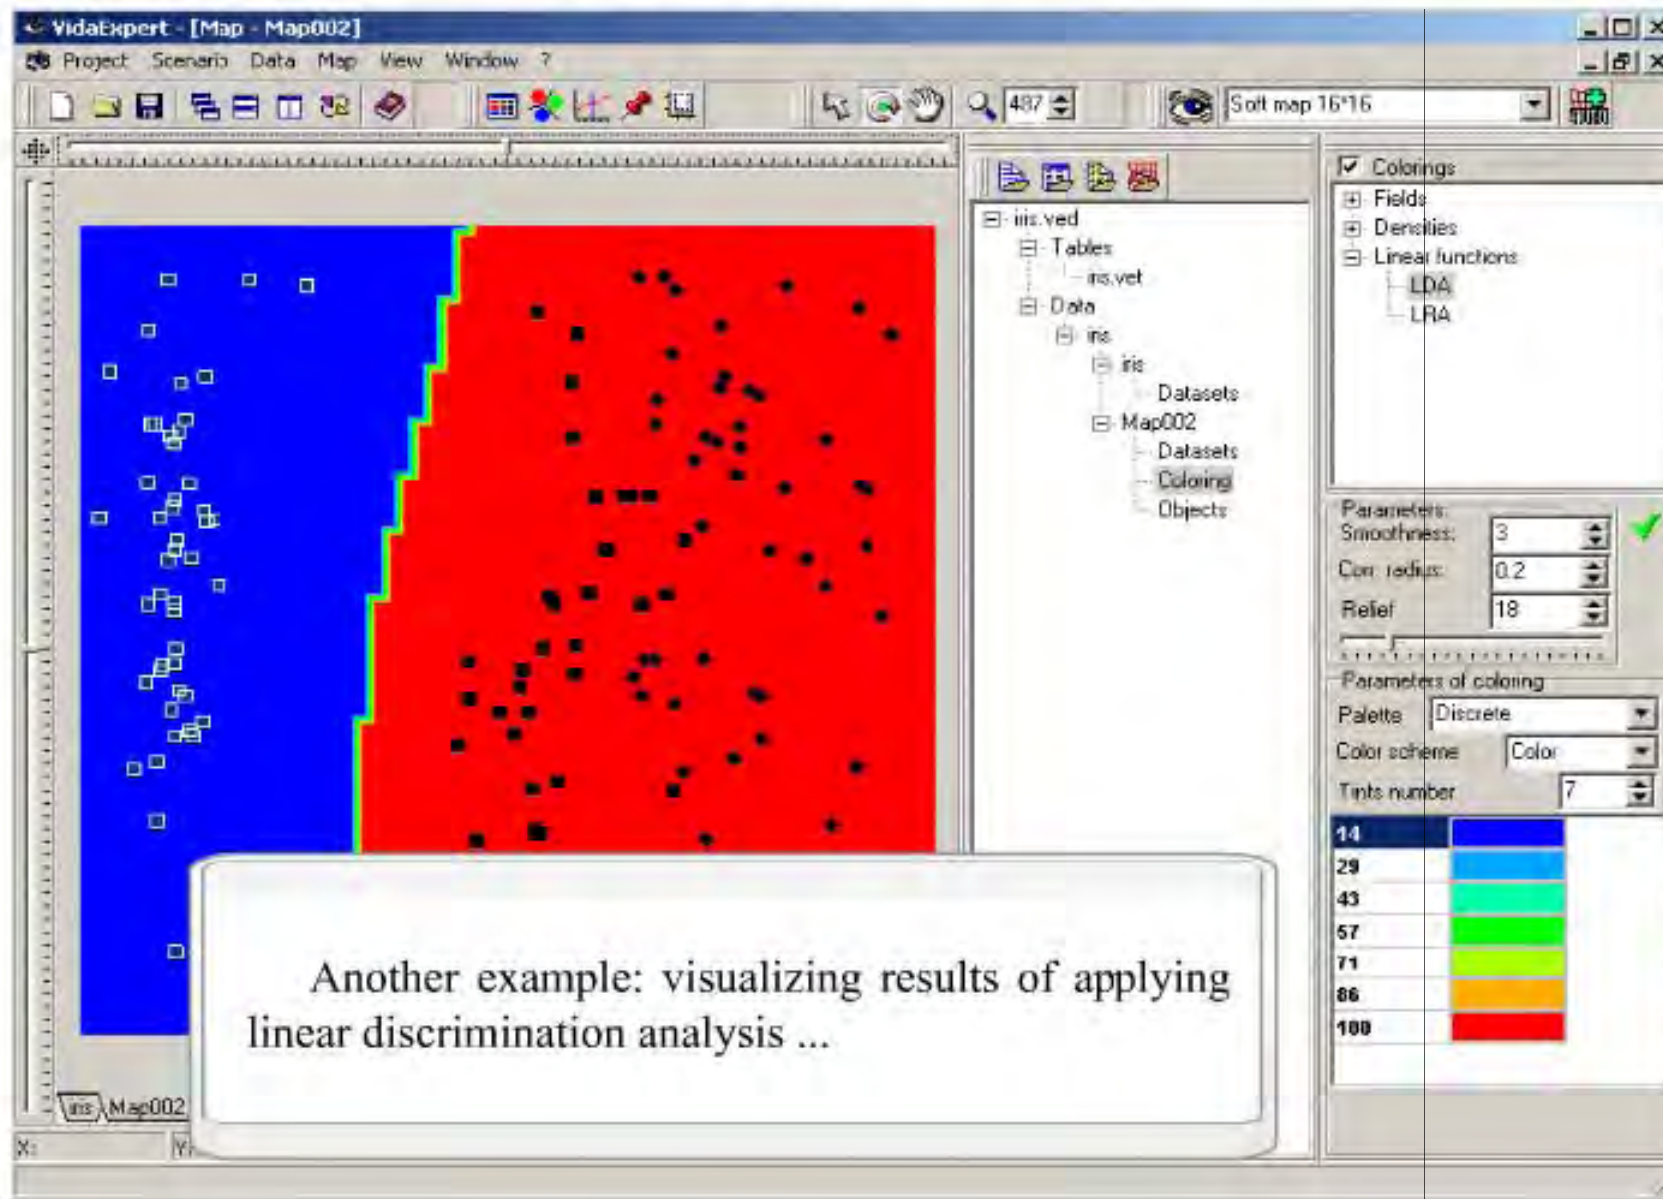

# VIDAEXPERT OVERVIEW

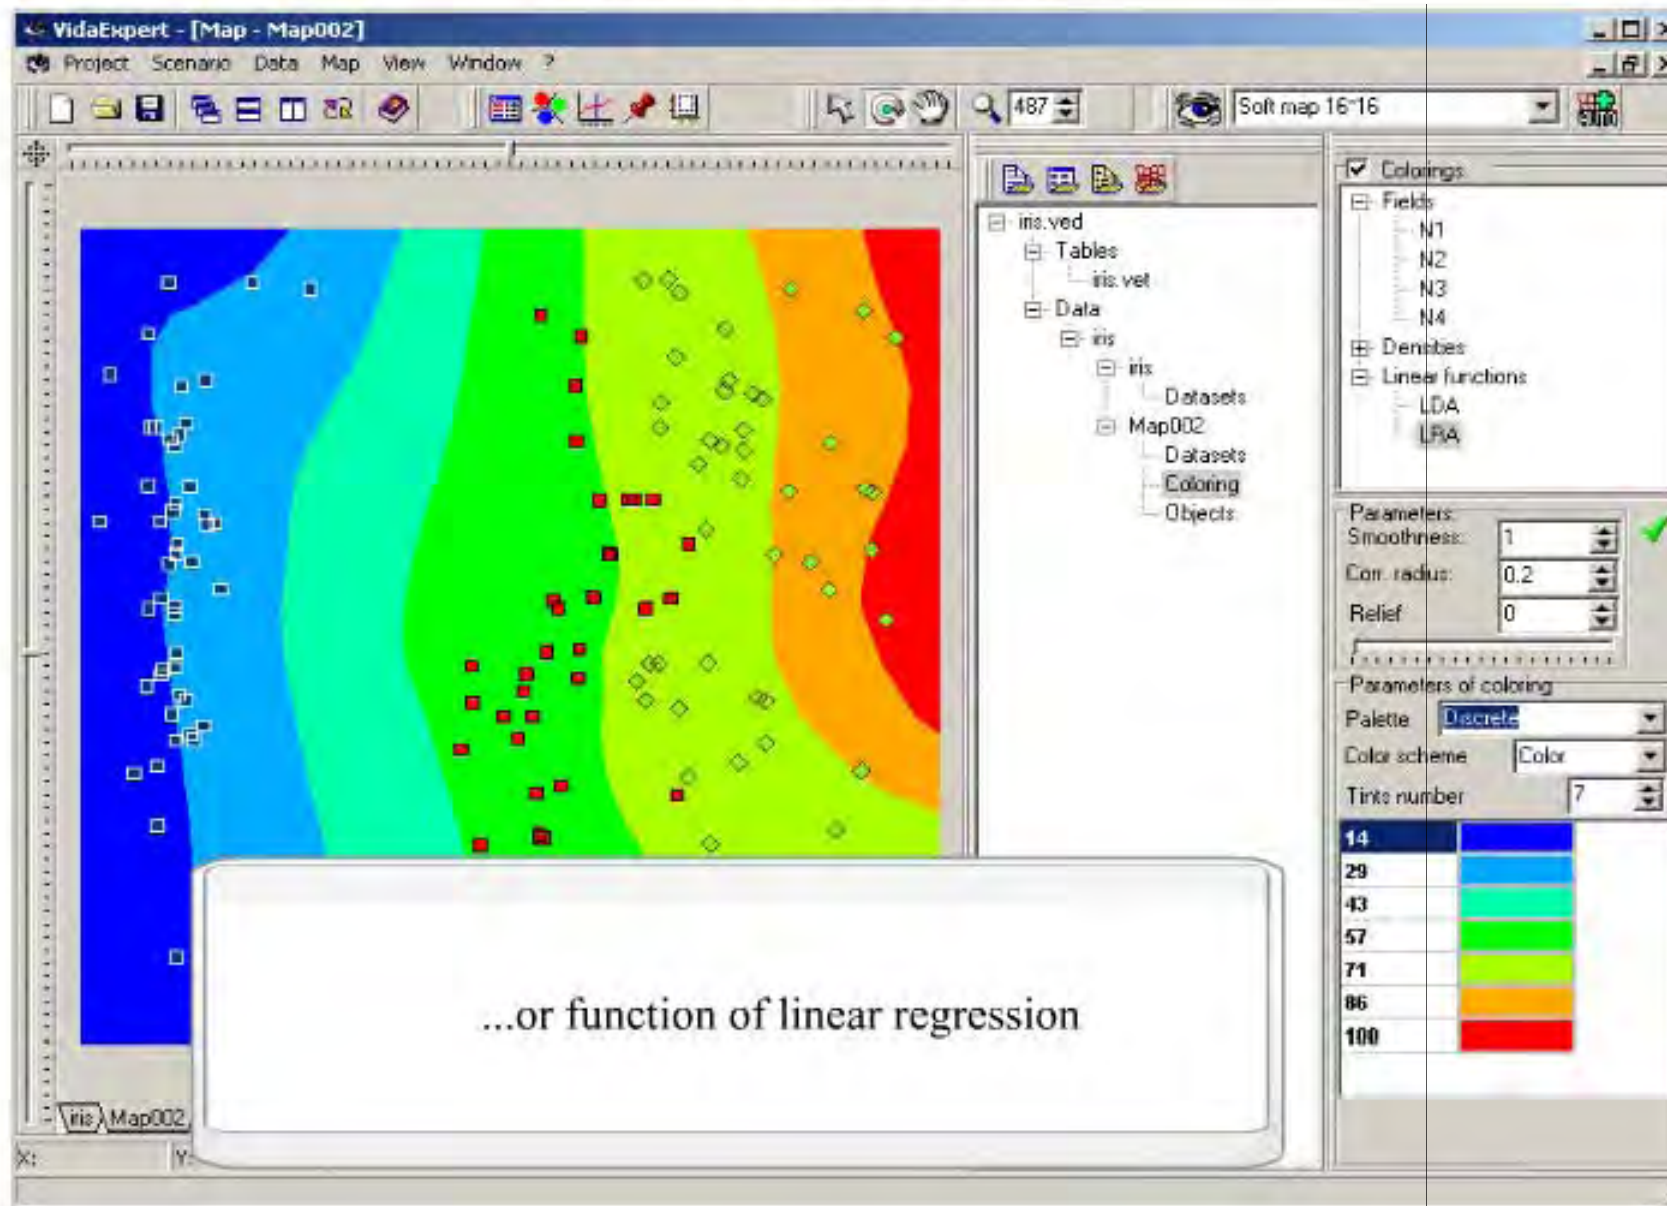



## VIDAEXPERT OVERVIEW

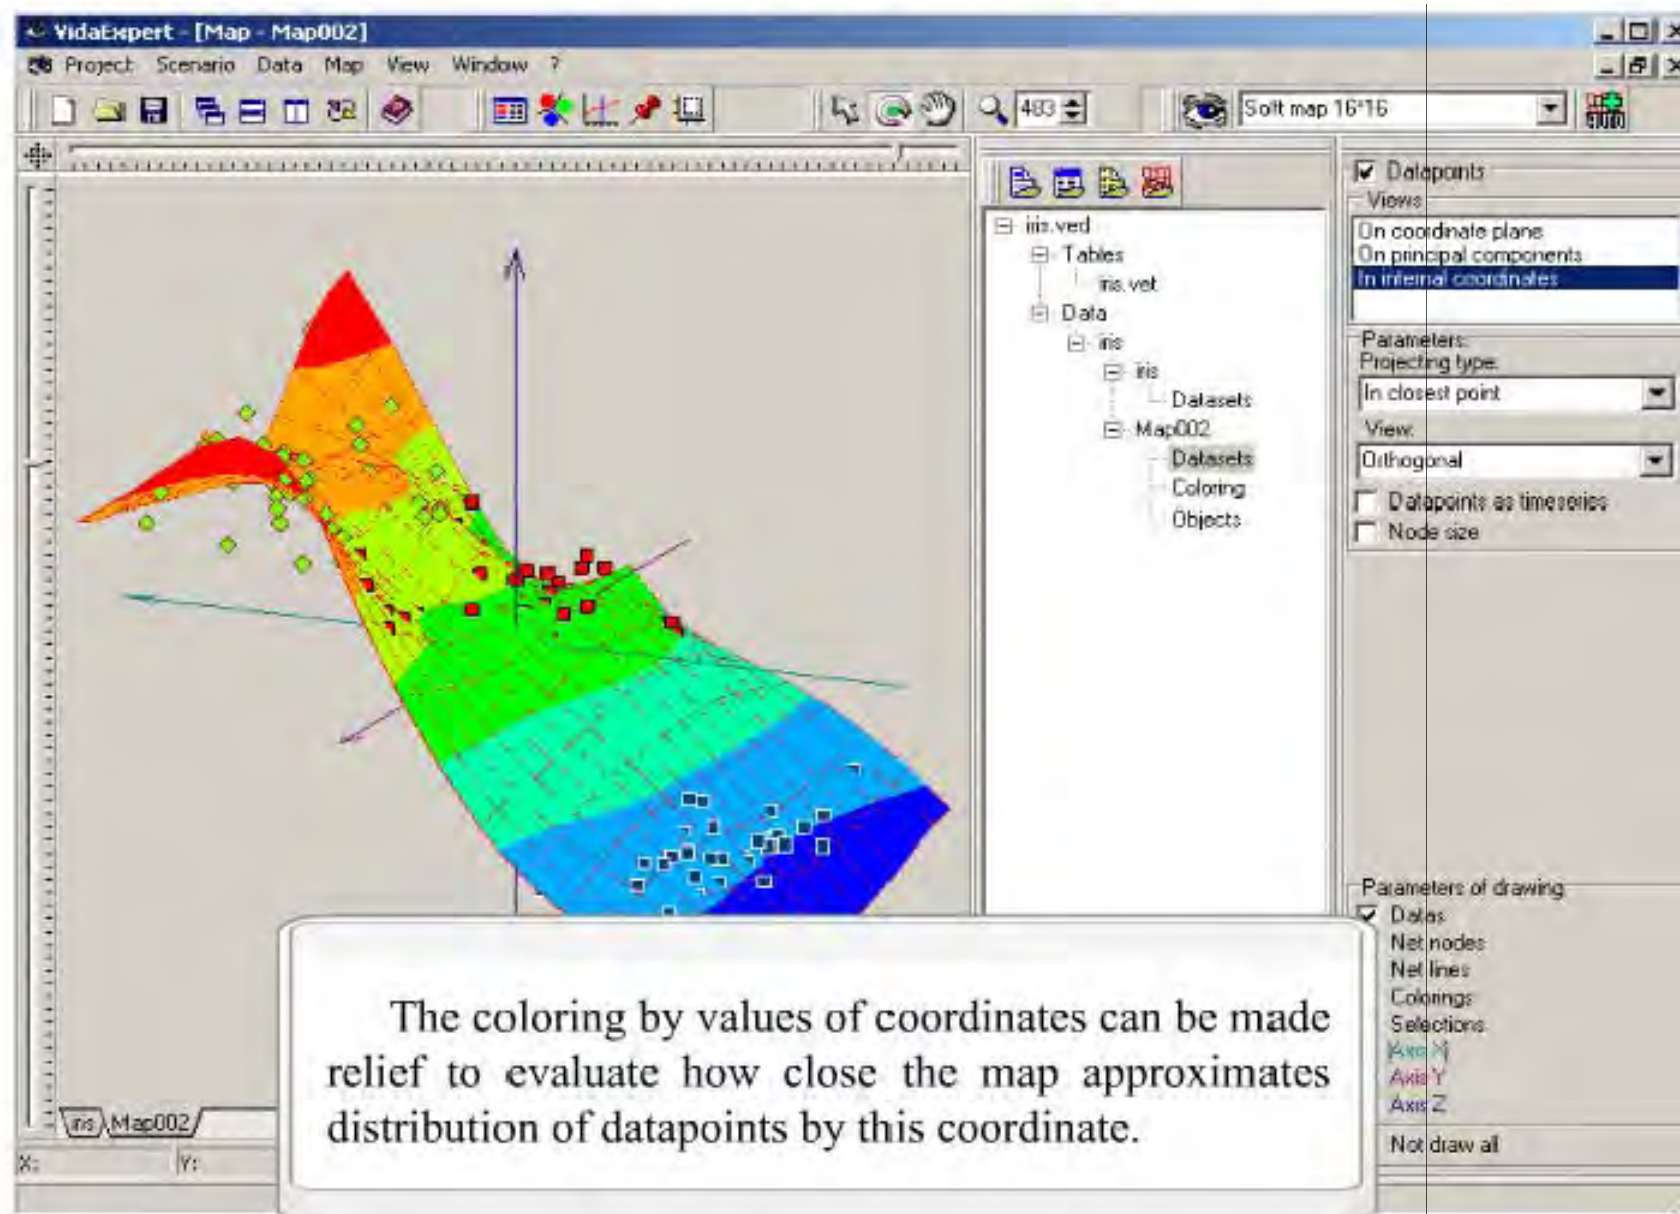

## VIDAEXPERT OVERVIEW

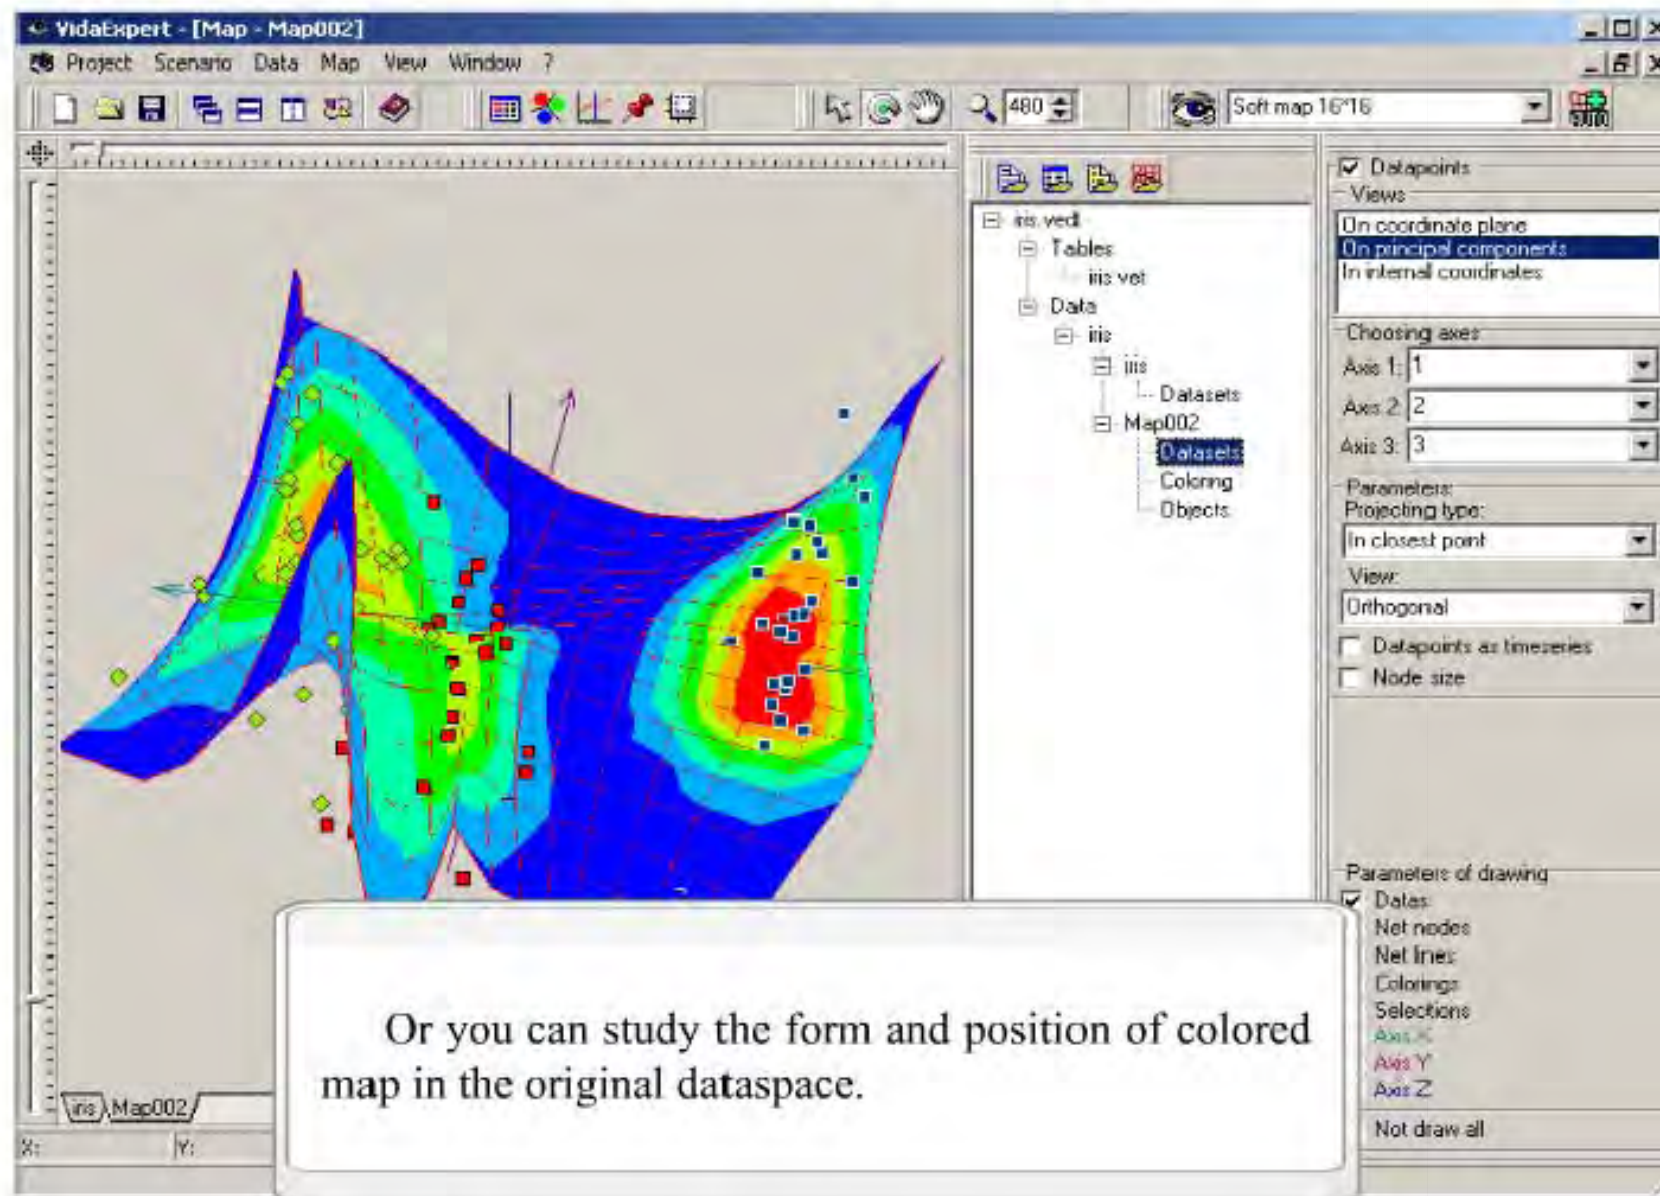



## VIDAEXPERT OVERVIEW

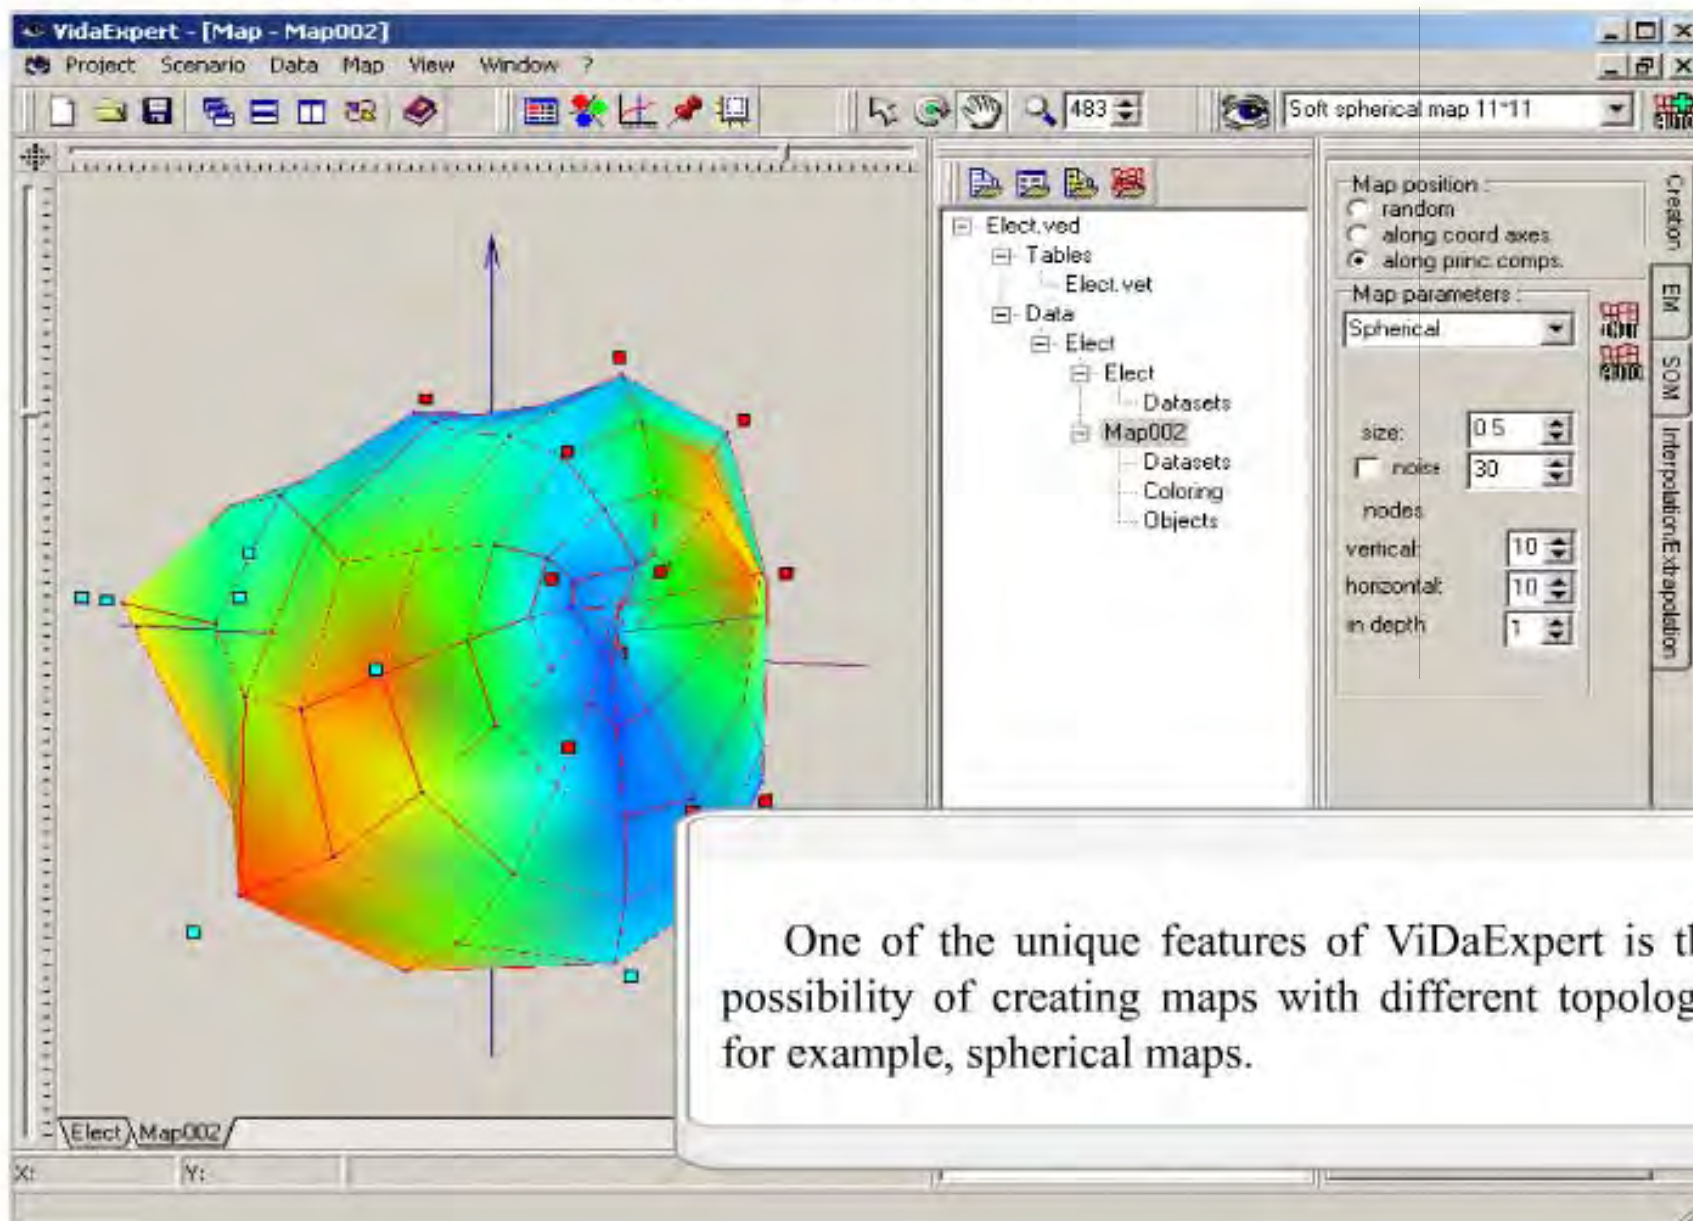

## VIDAEXPERT OVERVIEW

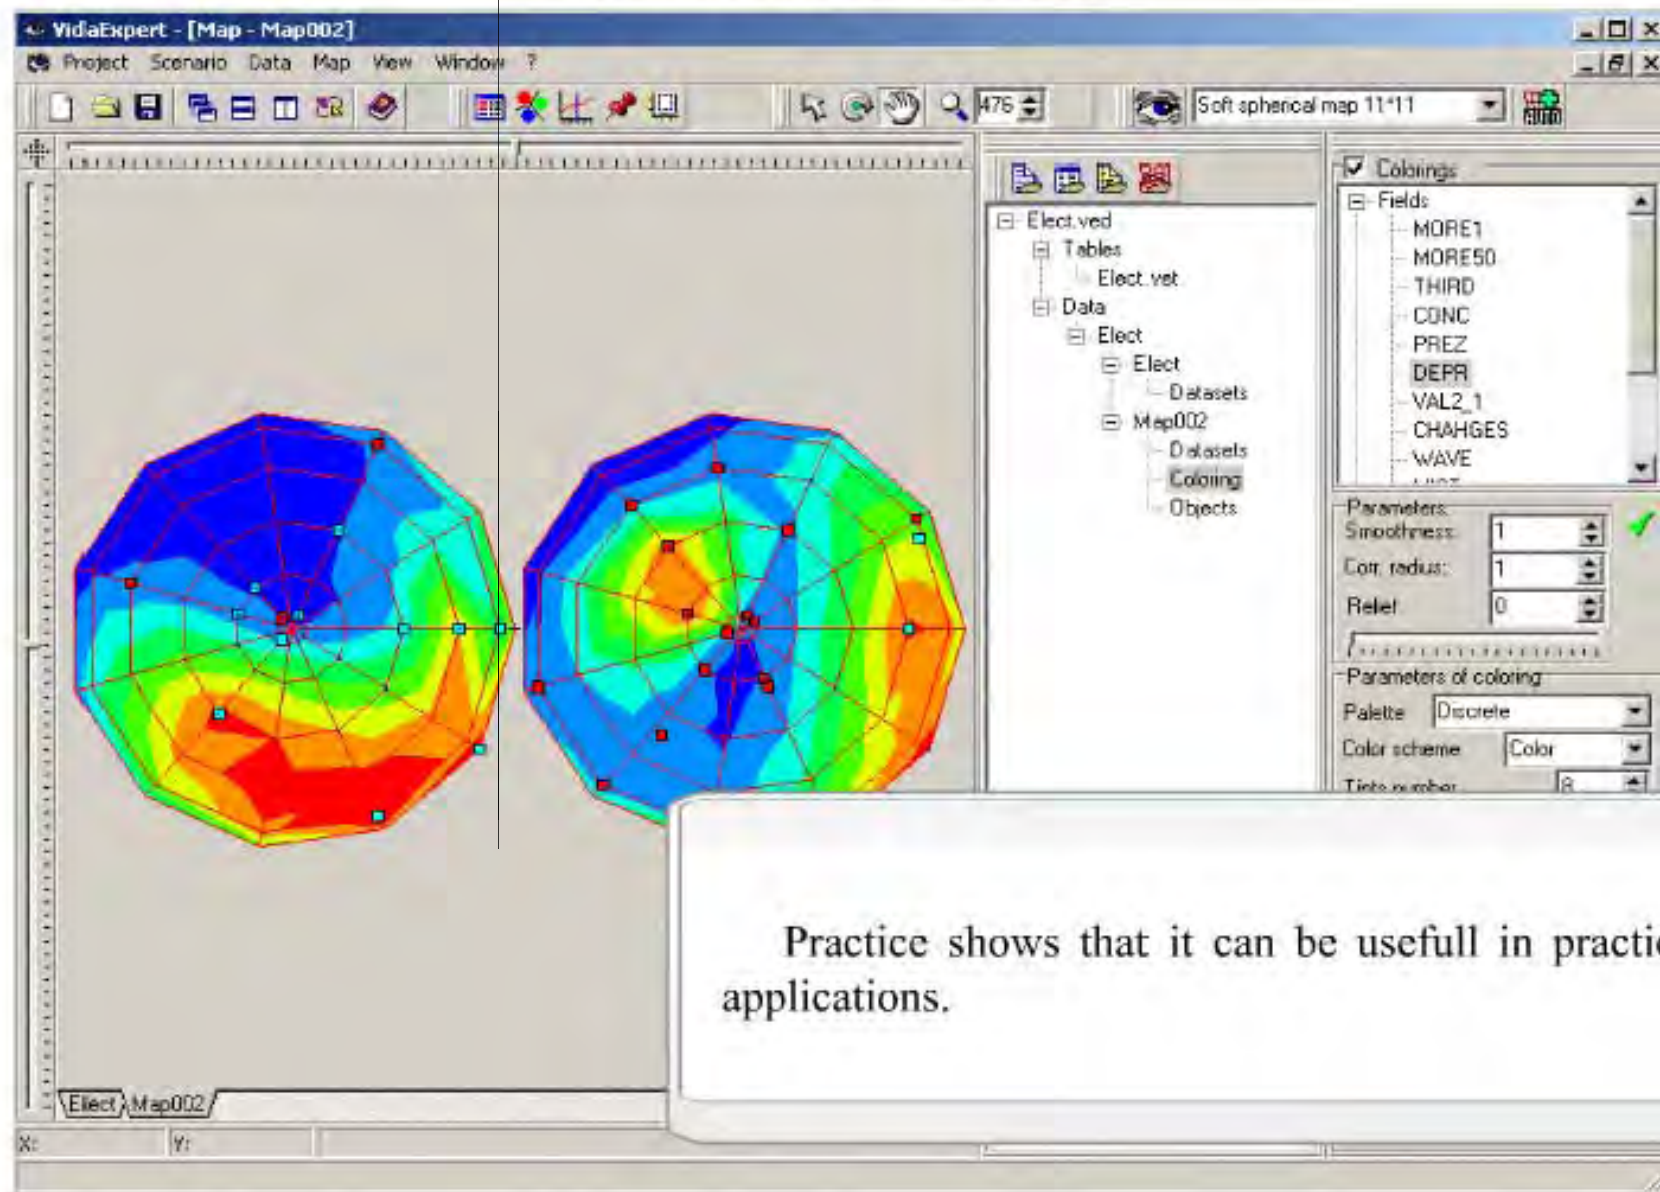



## VIDAEXPERT OVERVIEW

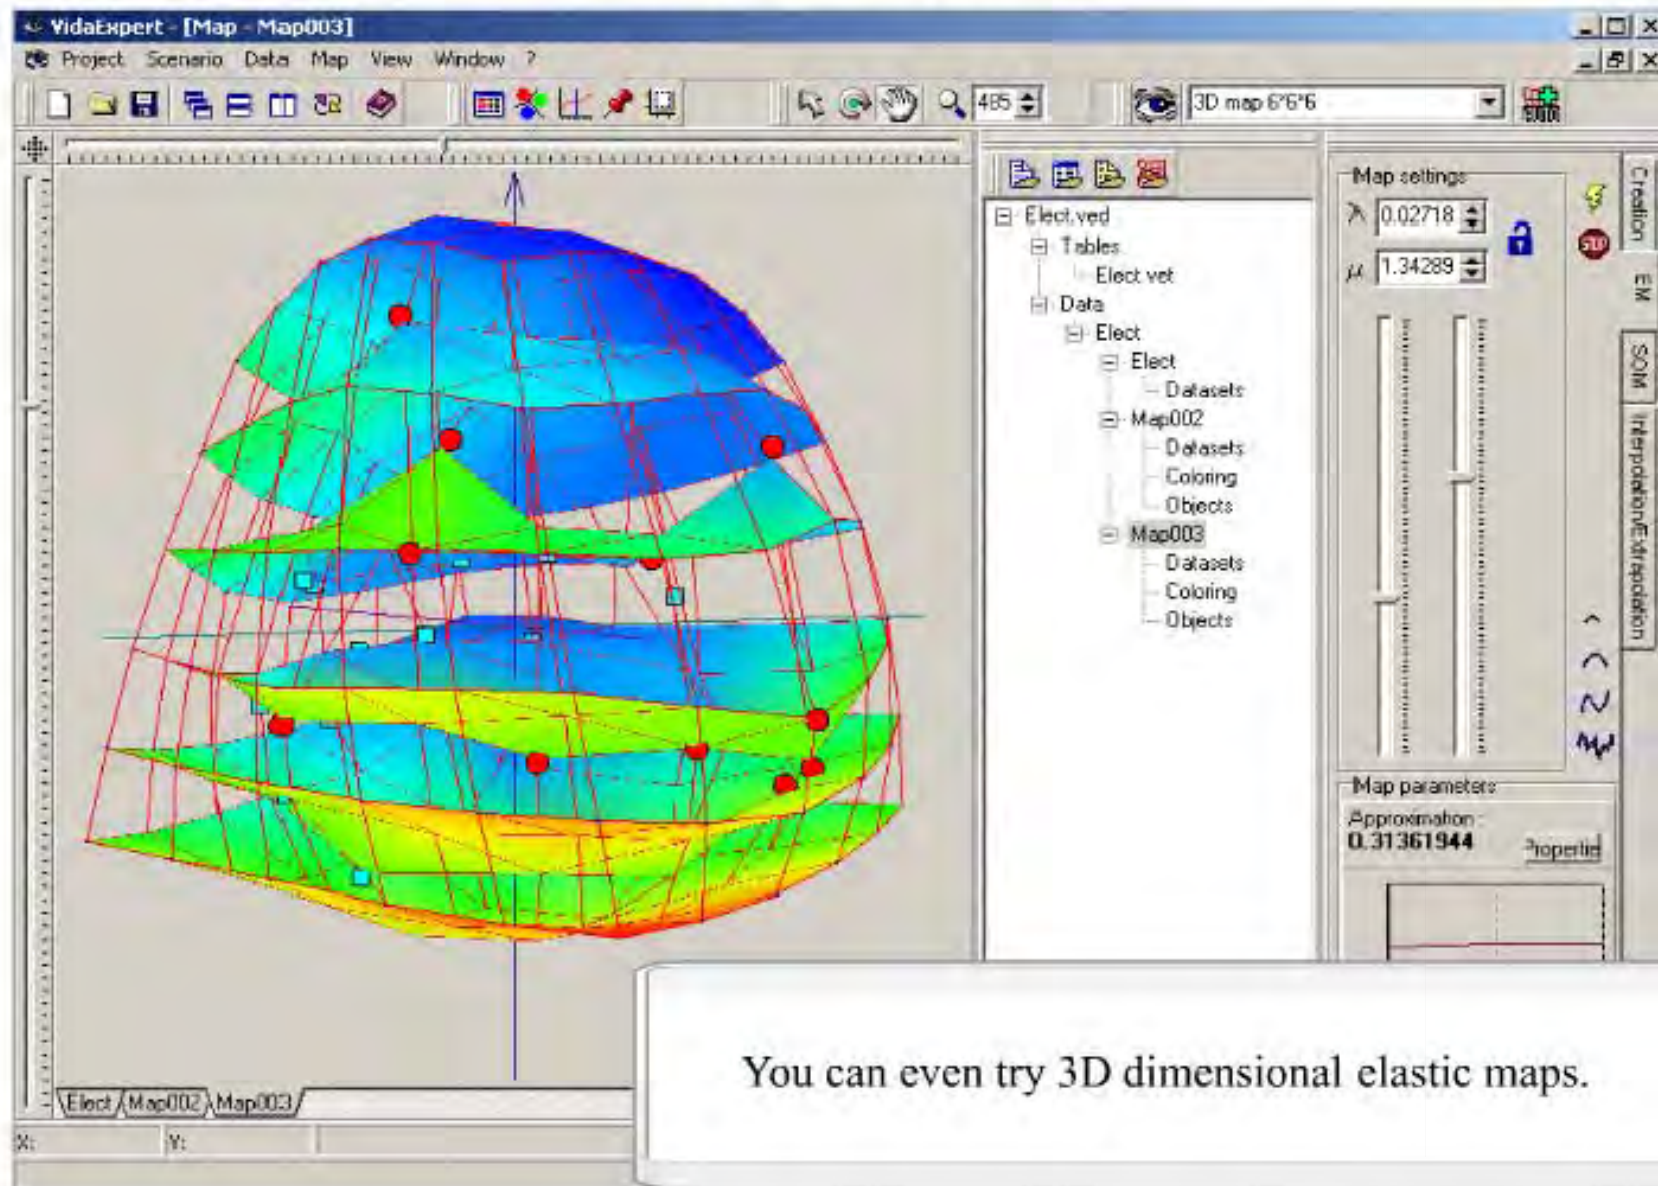

## VIDAEXPERT OVERVIEW

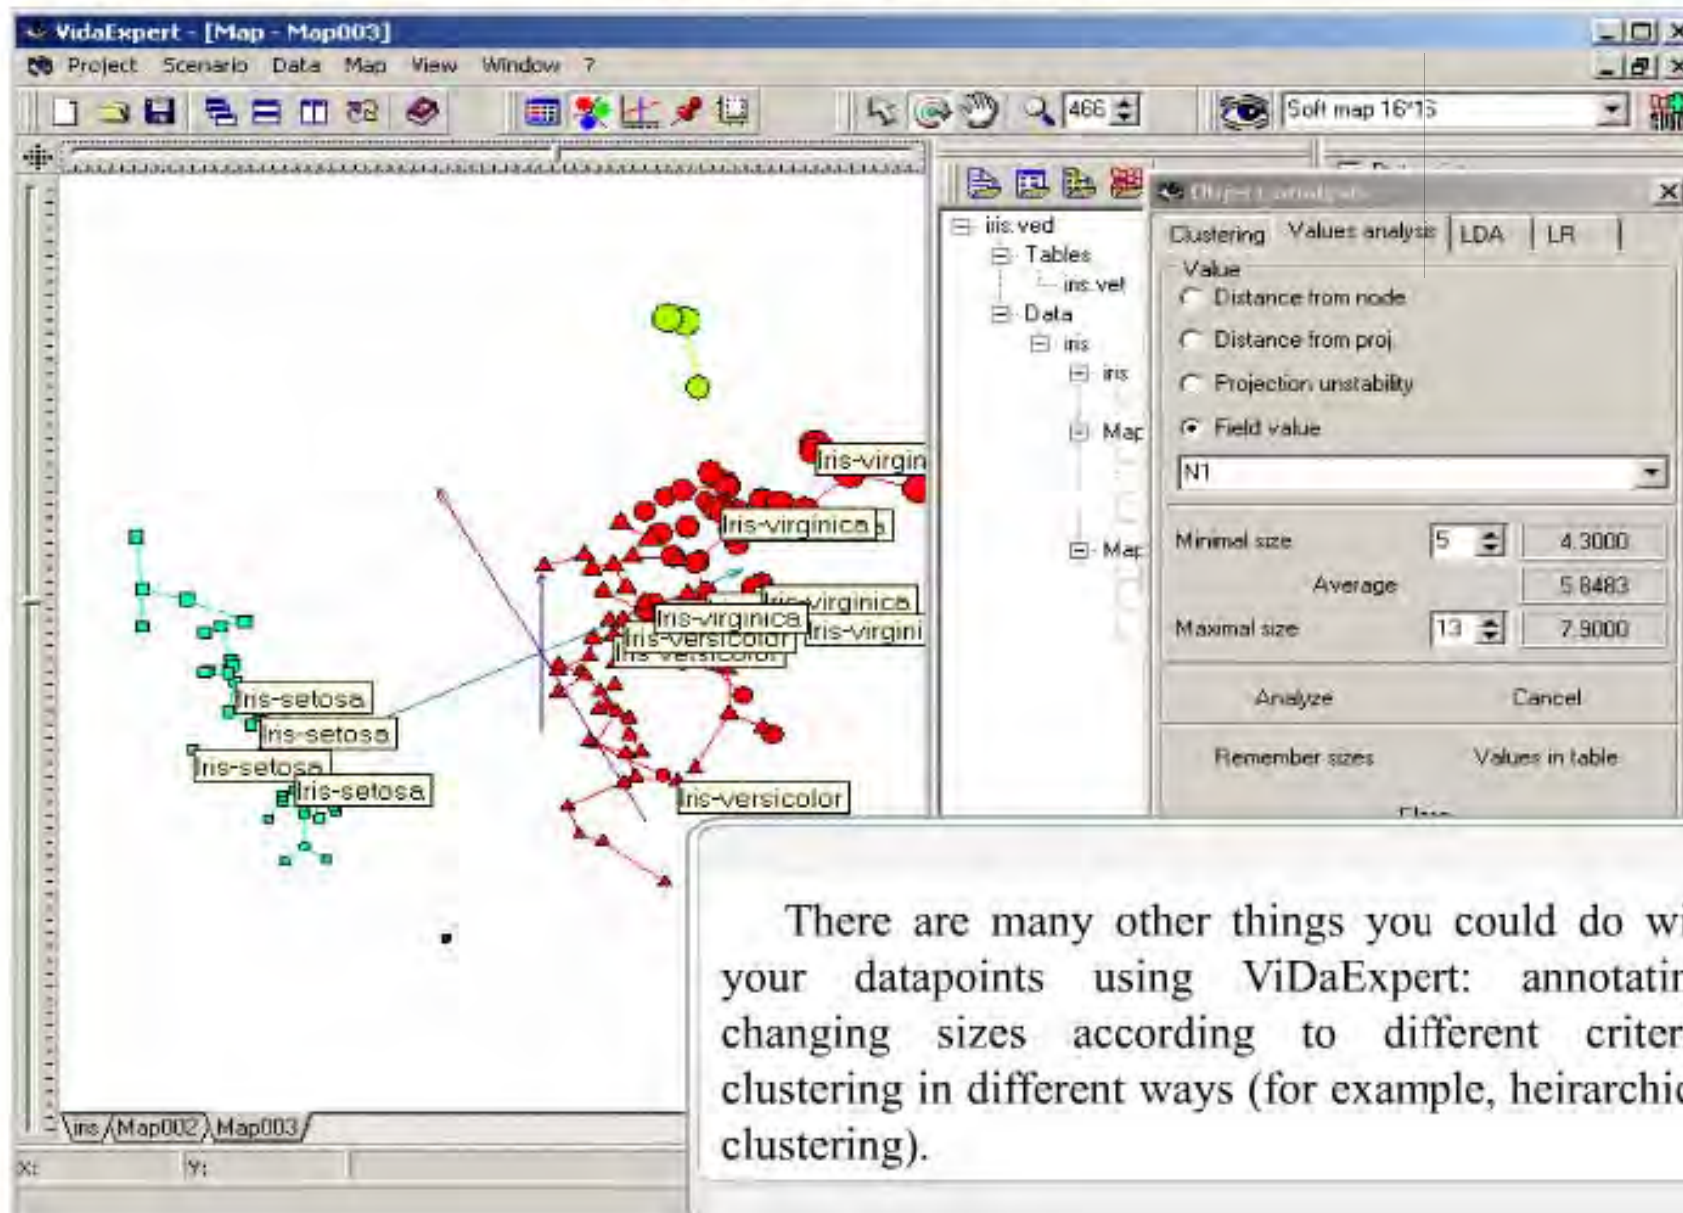



## VIDAEXPERT OVERVIEW

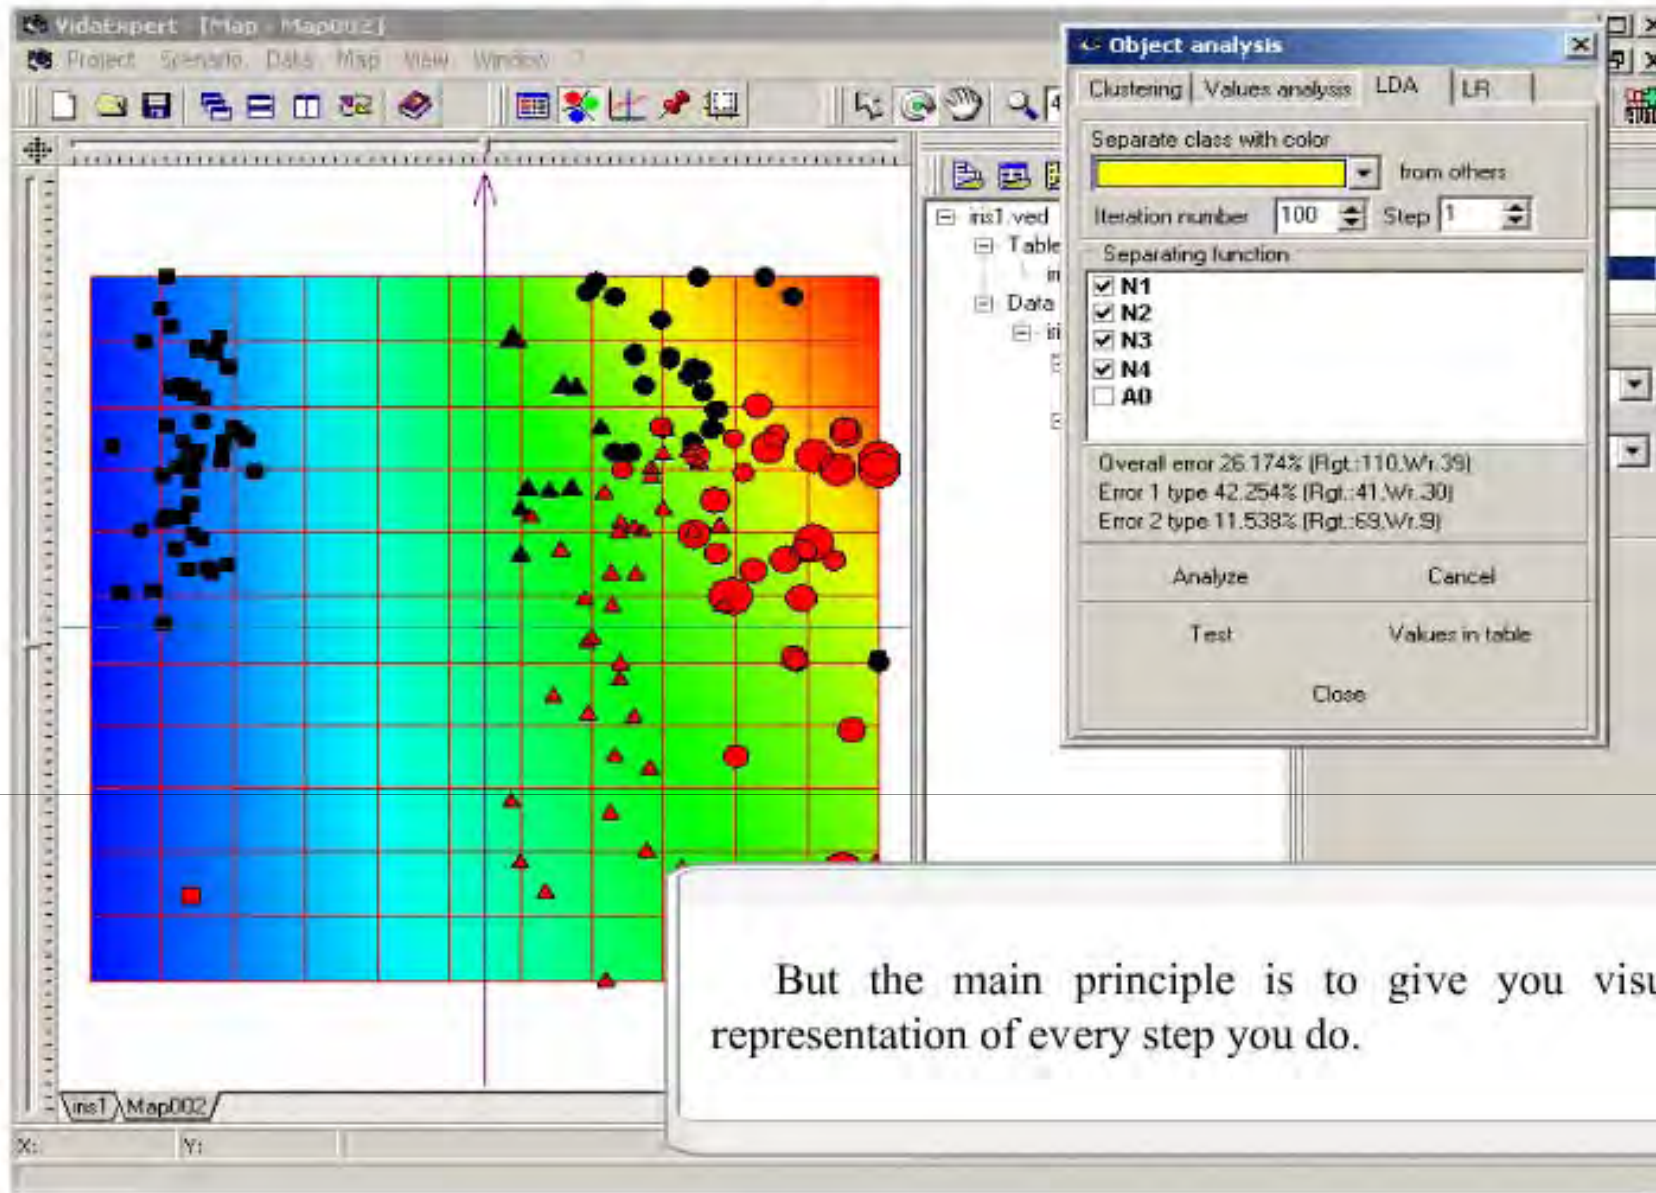

## VIDAEXPERT OVERVIEW

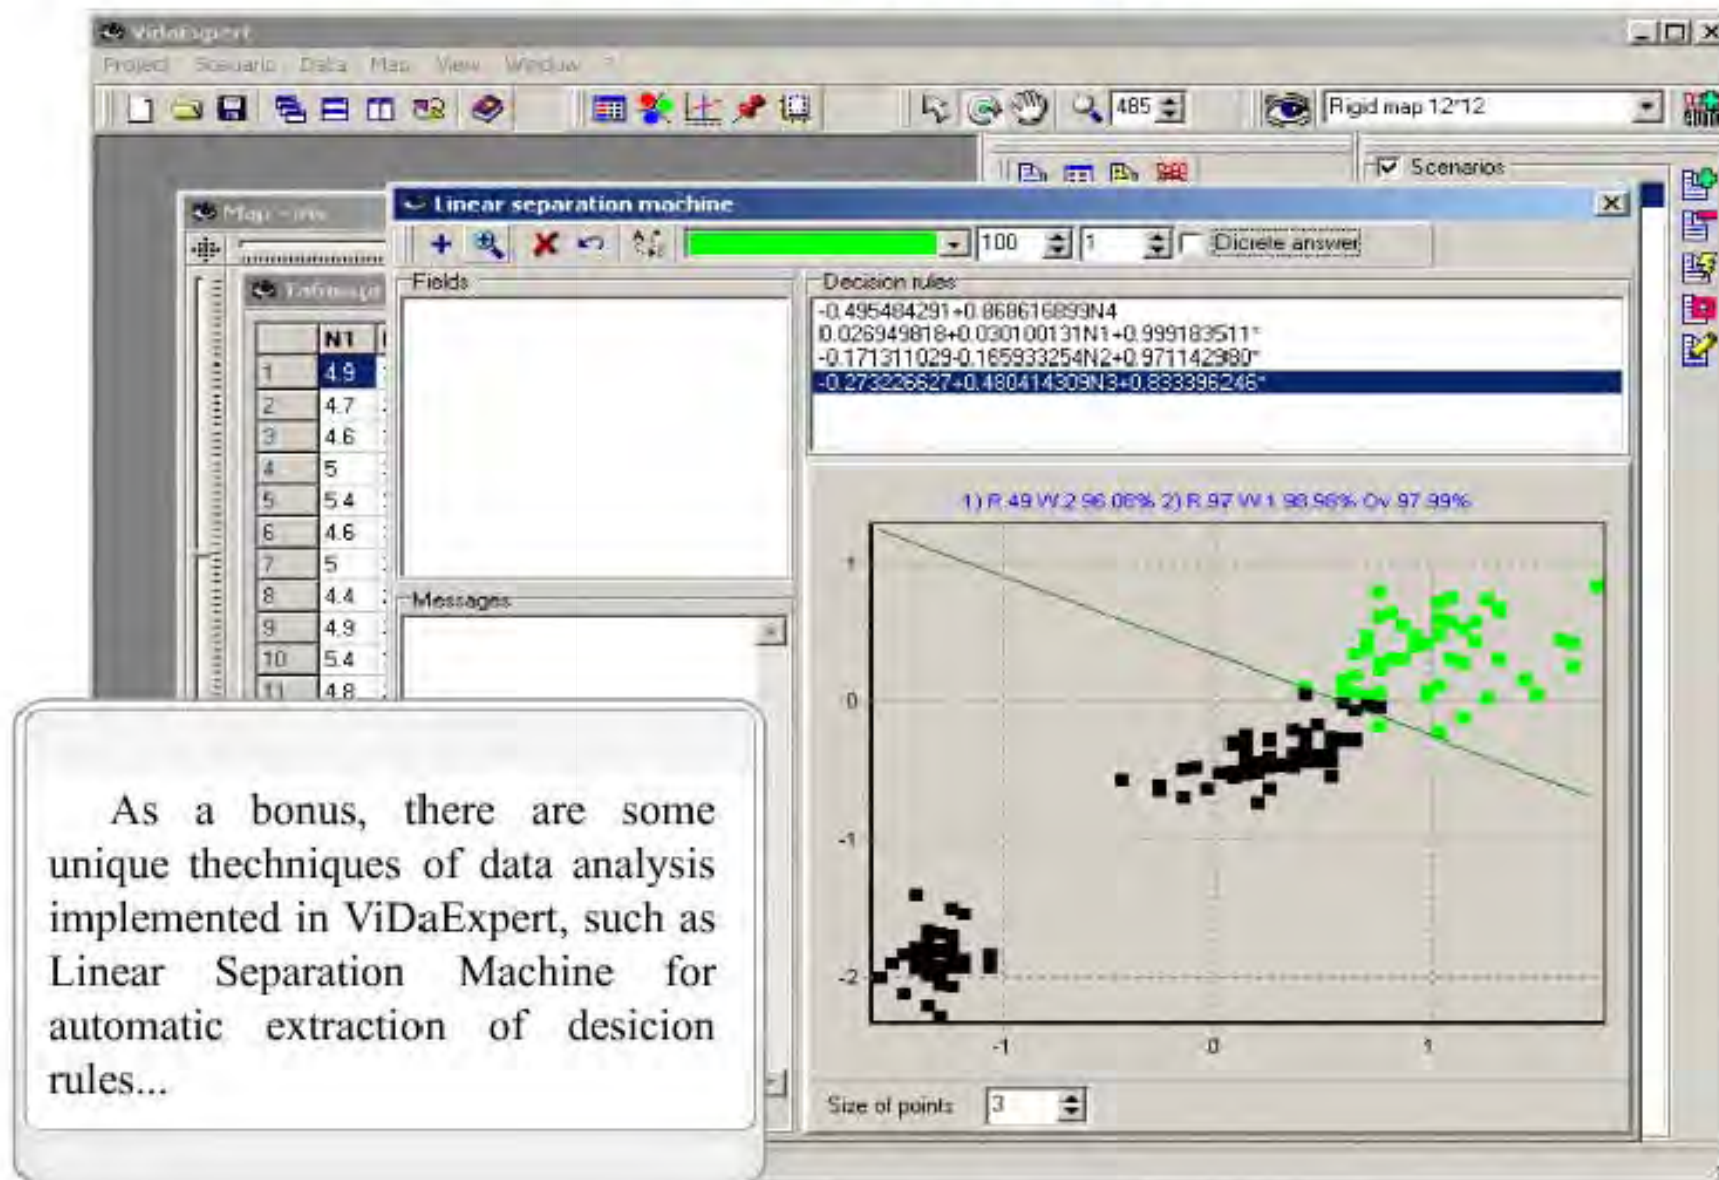



# VIDAEXPERT OVERVIEW

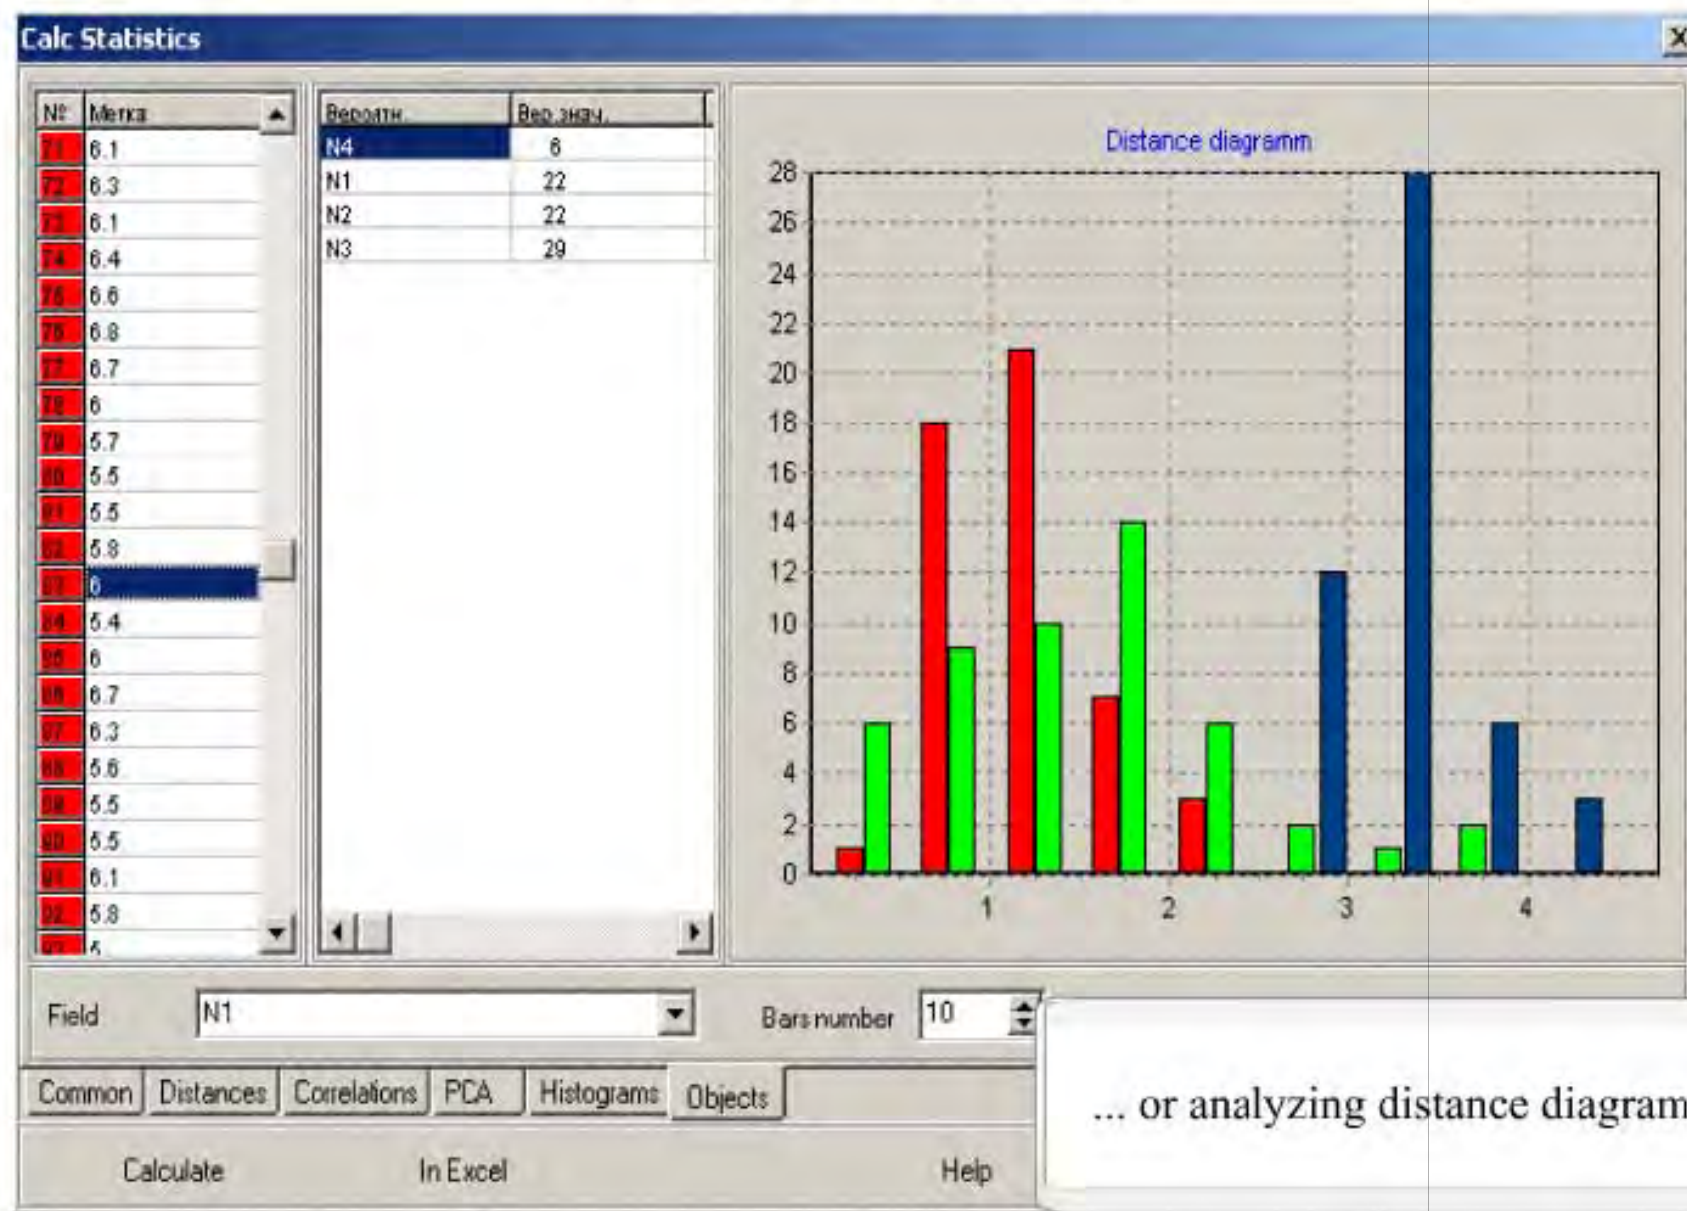

## *ViDaExpert 1.0* - data visualization software.

Conditions of distribution:  
free for non-commercial use.

Created by  
Zinovyev Andrey *auranic@hotmail.com*,  
Pitenko Alexander *pitty@iem.krasn.ru*.

## VIDAEXPERT: WORKING WITH DATASET

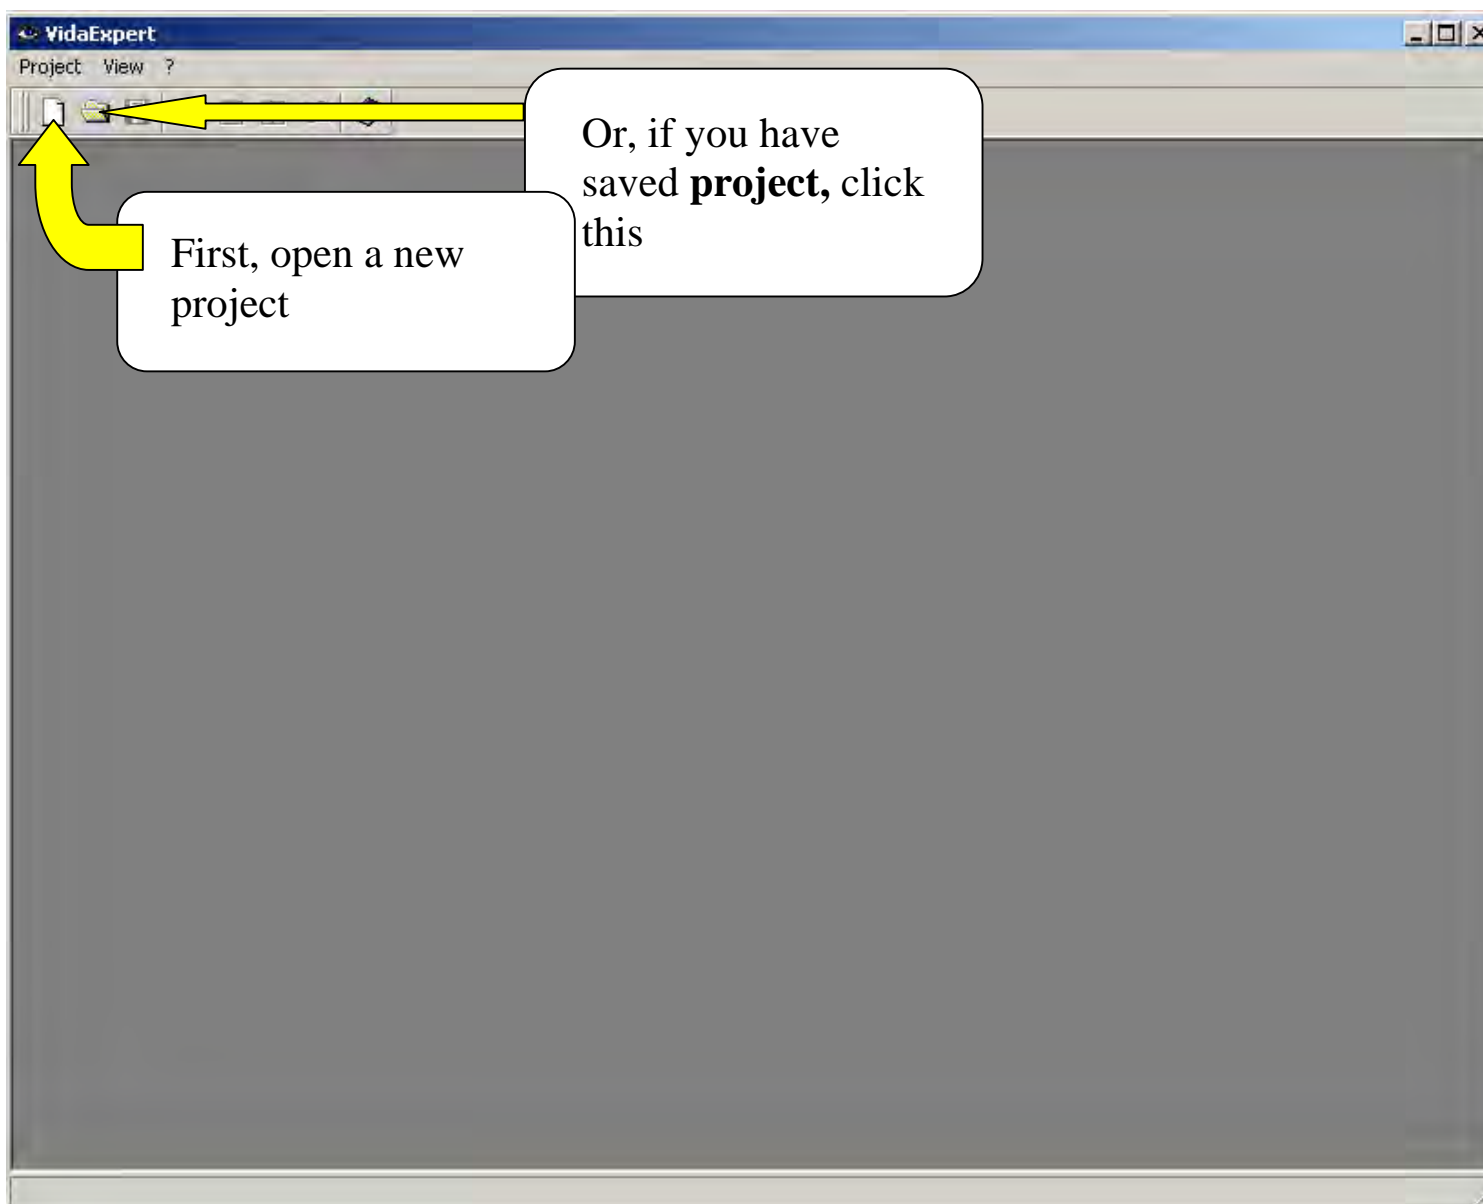

## VIDAEXPERT: WORKING WITH DATASETS

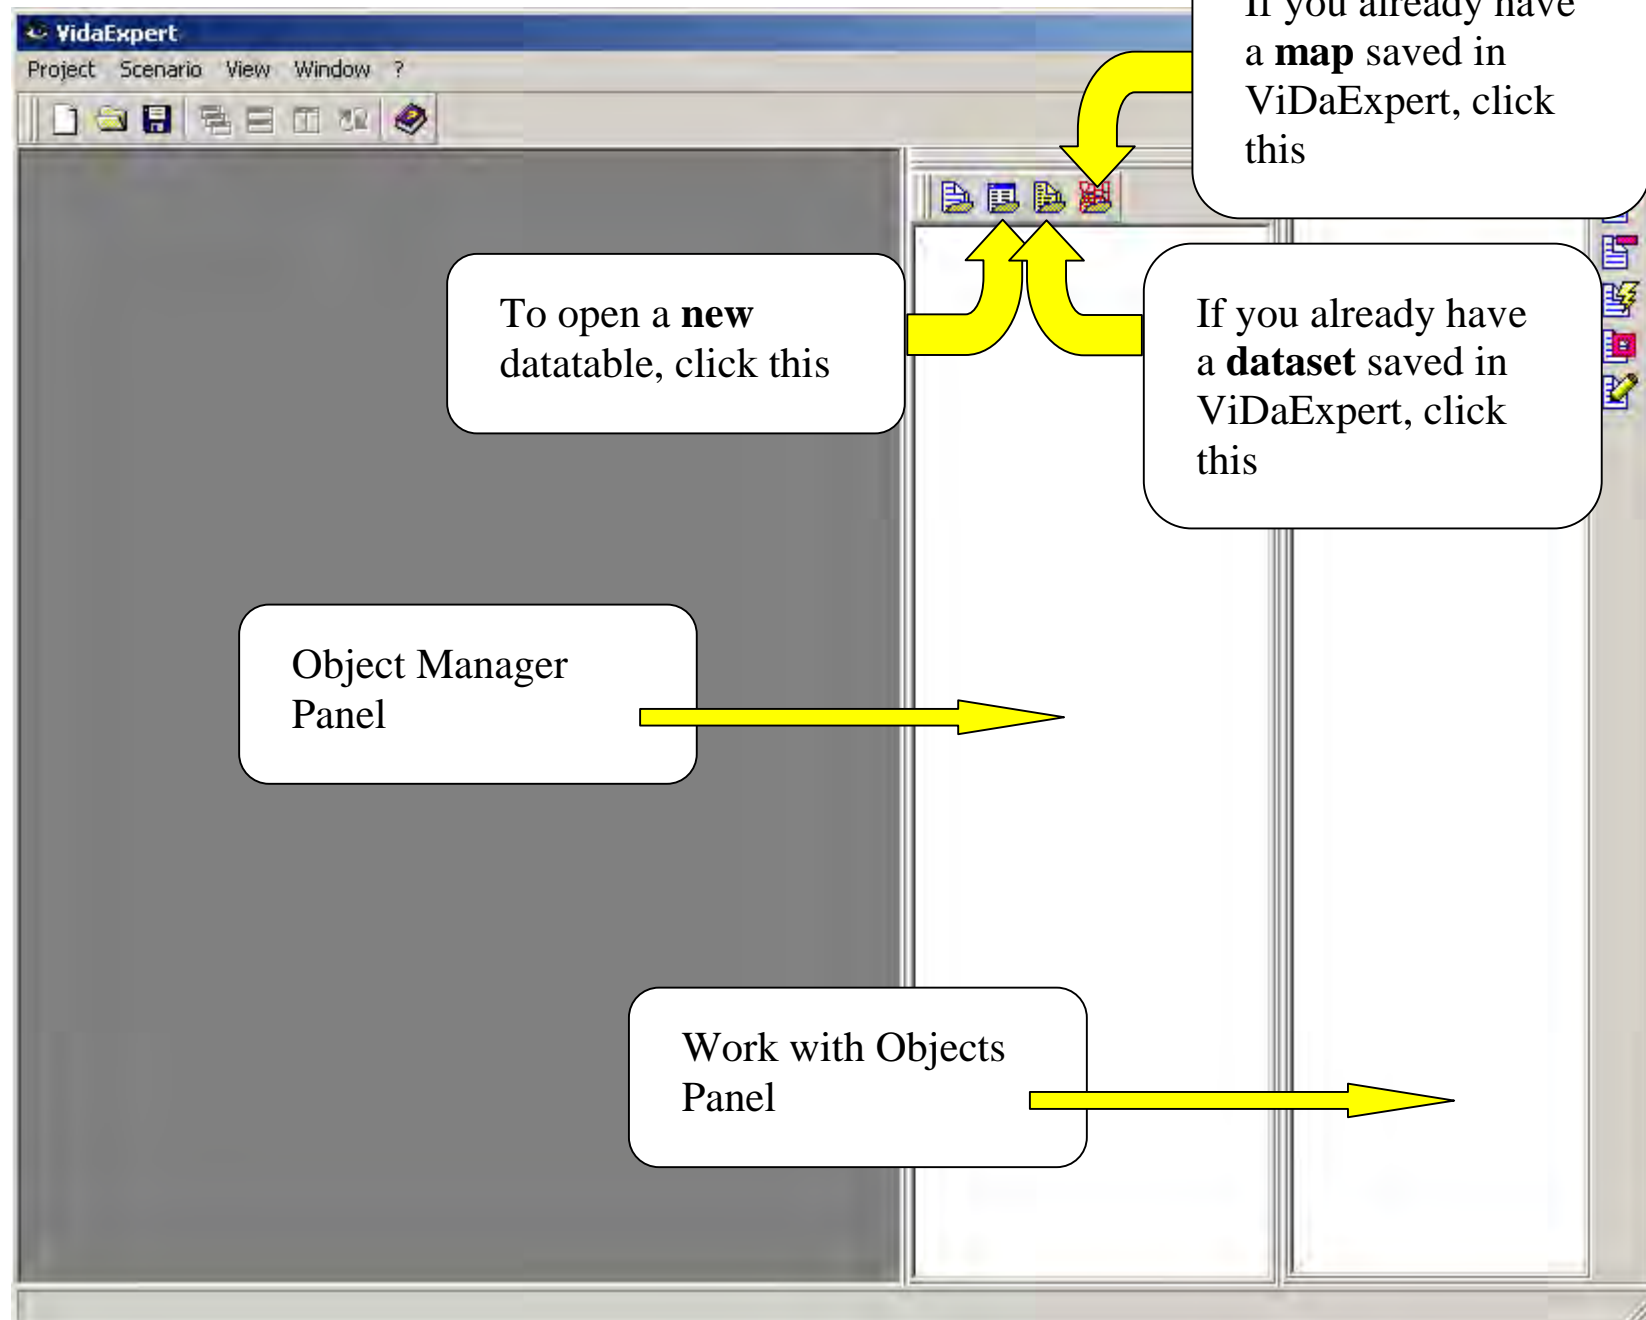



## VIDAEXPERT: WORKING WITH DATASET

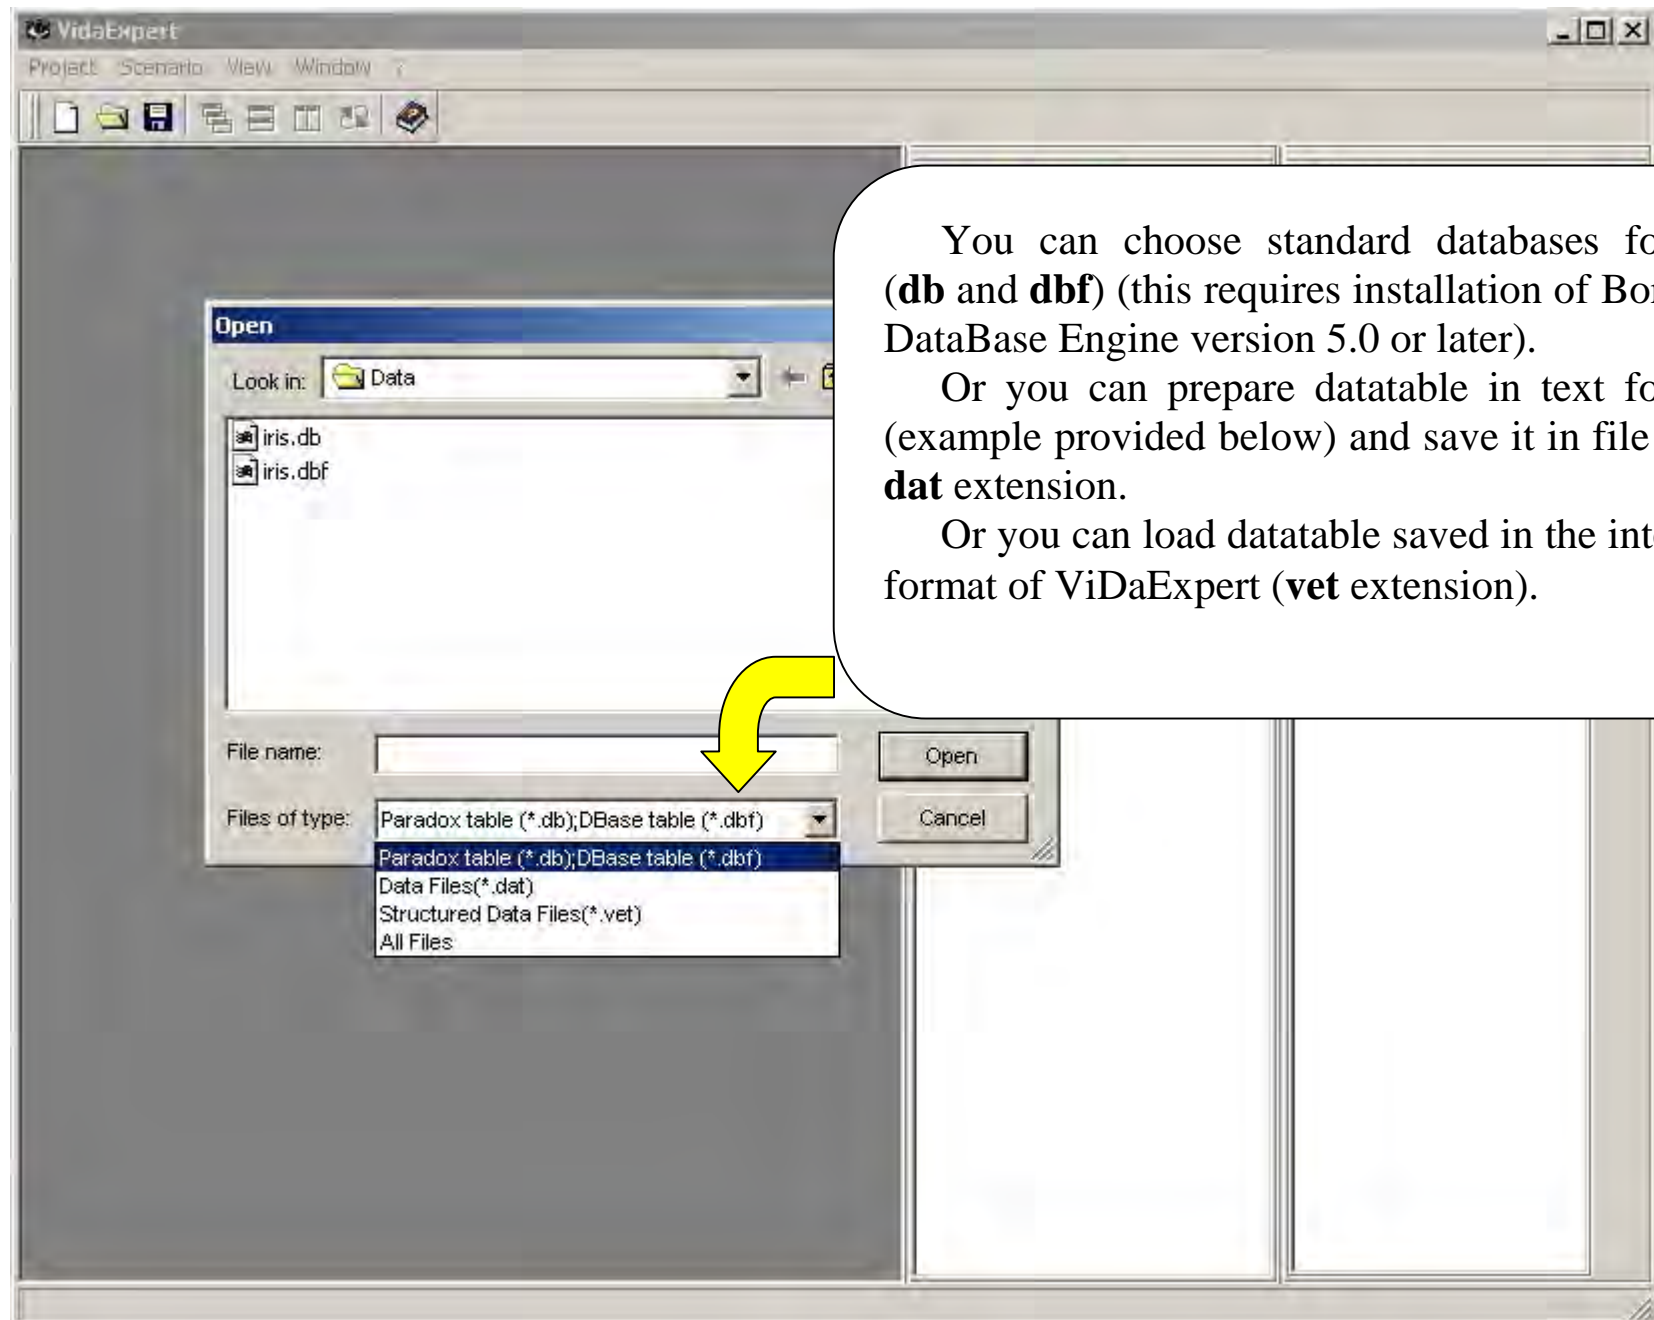

You can choose standard databases format (**db** and **dbf**) (this requires installation of Borland DataBase Engine version 5.0 or later).

Or you can prepare datatable in text format (example provided below) and save it in file with **dat** extension.

Or you can load datatable saved in the internal format of ViDaExpert (**vet** extension).

# VIDAEXPERT: WORKING WITH DATASET

## EXAMPLE OF DAT-FILE

----- Beginning of file -----

```
5 150
N1 FLOAT
N2 FLOAT
N3 FLOAT
N4 FLOAT
IRIS-SETOS STRING
4.9 3.0 1.4 0.2 "Iris-setosa with spaces"
4.7 3.2 1.3 @ Iris-setosa
4.6 3.1 1.5 0.2 Iris-setosa
5.0 3.6 1.4 0.2 Iris-setosa
5.4 3.9 1.7 0.4 Iris-setosa
4.6 3.4 1.4 0.3 Iris-setosa
5.0 3.4 1.5 0.2 Iris-setosa
4.4 2.9 1.4 0.2 Iris-setosa
4.9 3.1 1.5 0.1 Iris-setosa
5.4 3.7 1.5 0.2 Iris-setosa
----- .....
6.0 3.0 4.8 1.8 Iris-virginica
6.9 3.1 5.4 2.1 Iris-virginica
6.7 3.1 5.6 2.4 Iris-virginica
6.9 3.1 5.1 2.3 Iris-virginica
5.8 2.7 5.1 1.9 Iris-virginica
```

----- End of file -----

First line is the number of columns and the number of records in the datatable.

After one should provide description of every field in form “FIELD\_NAME FIELD\_TYPE”. Possible types are FLOAT and STRING.

After that, line after line, values of columns of every record separated by **spaces**. If a string-type value has spaces, it must be in quotes.

If you have **gap** (unknown value), then it should be marked by @ symbol.

## VIDAEXPERT: WORKING WITH DATASET

The screenshot displays the VidaExpert application window. The main panel shows a table titled "Таблица - iris.vet" with columns N1, N2, N3, and a list of Iris-setosa samples. Some cells in the N1 column are blank, representing gaps in the data. The right side of the interface features an "Object Manager Panel" with a tree view showing the hierarchy: iris > Tables > iris.vet > Data. A "Scenarios" panel on the far right shows a list of scenarios, including "iris".

Gaps in the datatable are displayed as blank spaces

This is the loaded table. It is displayed in Object Manager Panel. You can see that Scenario *iris* contains one **datatable** *iris.vet* and empty list of **datasets**. Now you see list of scenarios in Work With Objects Panel.

If you click on *Tables* in Object Manager Panel you will see the list of **datatables** in Work With Objects Panel.

If you click on *Data* in Object Manager Panel you will see the list of **datasets** in Work With Objects Panel.

You can add and delete scenarios by clicking on these buttons.

|   | N1  | N2  | N3  |                         |
|---|-----|-----|-----|-------------------------|
| 1 | 4.9 | 3.0 | 1.4 | Iris-setosa with spaces |
| 2 | 4.7 | 3.2 | 1.3 | Iris-setosa             |
| 3 | 4.6 | 3.1 | 1.5 | 0.2 Iris-setosa         |
| 4 | 5.0 | 3.6 | 1.4 | 0.2 Iris-setosa         |
| 5 | 5.4 | 3.9 | 1.7 | 0.4 Iris-setosa         |
| 6 | 4.6 | 3.4 | 1.4 | 0.3 Iris-setosa         |
| 7 | 5.0 | 3.4 | 1.5 | 0.2 Iris-setosa         |
| 8 | 4.4 | 2.9 | 1.4 | 0.2 Iris-setosa         |
| 9 | 4.9 | 3.1 | 1.5 | 0.1 Iris-setosa         |



## VIDAEXPERT: WORKING WITH DATASET

The screenshot shows the VidaExpert application window. The main window displays a table titled "Таблица - iris.vet" with columns N1, N2, N3, N4, and IRIS-SETOS. The table contains 21 rows of data. A context menu is open over the table, showing options: Mark, Unmark, Sort ascending, Sort descending, Change table, Transpose, In Excel, and In CSV. A yellow arrow points to the context menu. On the right, there is a "Scenarios" panel with a checkbox for "iris" and a tree view showing "iris" containing "Tables" (iris.vet) and "Data".

Highlight several records in the table and you can **mark** and **unmark** these records (right-click). Unmarked records will not be included in the dataset.

In addition, you can **sort** table by the values of current column, you can **change** table for another one, transpose table (columns become rows and rows become columns), print out the table (as you see it) in **Excel** or **CSV** file.

|    | N1  | N2  | N3  | N4  | IRIS-SETOS  |
|----|-----|-----|-----|-----|-------------|
| 1  | 4.9 | 3   | 1.4 | 0.2 | Iris-setosa |
| 2  | 4.7 | 3.2 | 1.3 | 0.2 | Iris-setosa |
| 3  | 4.6 | 3.1 | 1.5 | 0.2 | Iris-setosa |
| 4  | 5   | 3.6 | 1.4 | 0.2 | Iris-setosa |
| 5  | 5.4 | 3.9 | 1.7 | 0.4 | Iris-setosa |
| 6  | 4.6 | 3.4 | 1.4 | 0.3 | Iris-setosa |
| 7  | 5   | 3.4 | 1.5 | 0.2 | Iris-setosa |
| 8  | 4.4 | 2.9 | 1.4 | 0.2 | Iris-setosa |
| 9  | 4.9 | 3.1 | 1.5 | 0.1 | Iris-setosa |
| 10 | 5.4 | 3.7 | 1.5 | 0.2 | Iris-setosa |
| 11 | 4.8 | 3.4 | 1.6 | 0.2 | Iris-setosa |
| 12 | 4.8 | 3   | 1.4 | 0.1 | Iris-setosa |
| 13 | 4.3 | 3   | 1.1 | 0.1 | Iris-setosa |
| 14 | 5.8 | 4   | 1.2 | 0.2 | Iris-setosa |
| 15 | 5.7 | 4.4 | 1.5 | 0.4 | Iris-setosa |
| 16 | 5.4 | 3.9 | 1.3 | 0.4 | Iris-setosa |
| 17 | 5.1 | 3.5 | 1.4 | 0.3 | Iris-setosa |
| 18 | 5.7 | 3.8 | 1.7 | 0.3 | Iris-setosa |
| 19 | 5.1 | 3.8 | 1.5 | 0.3 | Iris-setosa |
| 20 | 5.4 | 3.4 | 1.7 | 0.2 | Iris-setosa |
| 21 | 5.1 | 3.7 | 1.5 | 0.4 | Iris-setosa |

## VIDAEXPERT: WORKING WITH DATASET

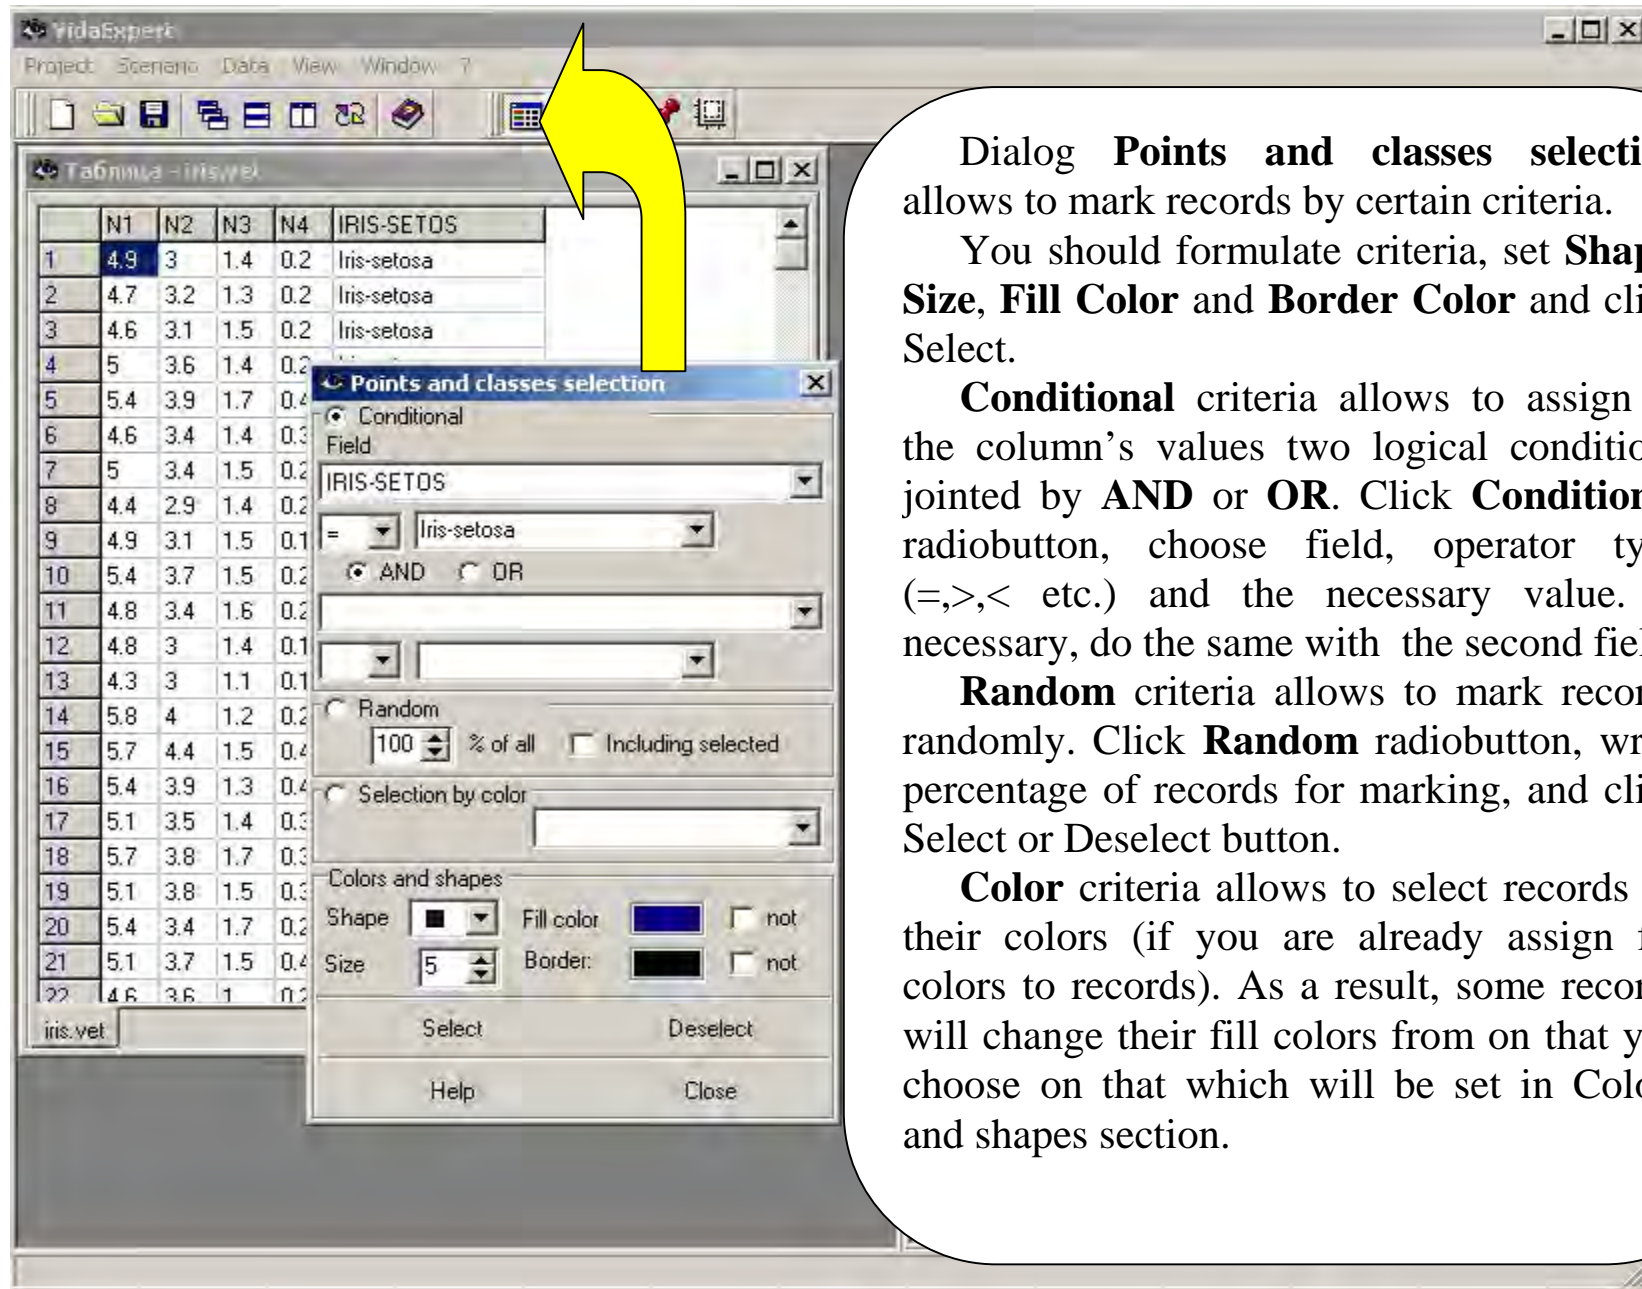

The screenshot shows the VidaExpert application window. The main window displays a table with columns N1, N2, N3, N4, and IRIS-SETOS. The table contains 22 rows of data. A yellow arrow points from the 'Points and classes selection' dialog box to the table. The dialog box is titled 'Points and classes selection' and has three main sections: 'Conditional', 'Random', and 'Selection by color'. The 'Conditional' section is selected, showing a field 'IRIS-SETOS' with a dropdown menu set to 'Iris-setosa'. The 'Random' section has a '100' value and a 'Including selected' checkbox. The 'Selection by color' section has a 'Shape' dropdown set to '5' and a 'Fill color' dropdown set to 'not'. The 'Colors and shapes' section has a 'Shape' dropdown set to '5' and a 'Fill color' dropdown set to 'not'. The 'Border' section has a 'Border' dropdown set to 'not'. The 'Select' and 'Deselect' buttons are visible at the bottom of the dialog box.

Dialog **Points and classes selection** allows to mark records by certain criteria.

You should formulate criteria, set **Shape**, **Size**, **Fill Color** and **Border Color** and click **Select**.

**Conditional** criteria allows to assign to the column's values two logical conditions jointed by **AND** or **OR**. Click **Conditional** radiobutton, choose field, operator type (=,>,< etc.) and the necessary value. If necessary, do the same with the second field.

**Random** criteria allows to mark records randomly. Click **Random** radiobutton, write percentage of records for marking, and click **Select** or **Deselect** button.

**Color** criteria allows to select records by their colors (if you are already assign fill colors to records). As a result, some records will change their fill colors from on that you choose on that which will be set in Colors and shapes section.

## VIDAEXPERT: WORKING WITH DATASET

The screenshot shows the VidaExpert software interface. The main window displays a table titled "Таблица - iris.vet" with columns N1, N2, N3, N4, and IRIS-SETOS. The table contains 20 rows of data. A yellow arrow points from the table to the "iris.vet" entry in the "Tables" pane on the right. Another yellow arrow points from the "iris.vet" entry to the "Table fields" list, which includes N1, N2, N3, N4, and IRIS-SETOS. A third yellow arrow points from the "Table fields" list to the "Exclude gaps" checkbox. A fourth yellow arrow points from the "Table fields" list to the "Normalizing selected fields" section, which includes checkboxes for "On logarithm", "On hyperbolic tangent", "On standart deviation", and "On (-1;1) diapason".

3. Finally, click **Create dataset** button.

1. Click on the table in Object Manager to go to the final stage of creating dataset.

2. You should mark the fields for including in the dataset and set the rule of normalization for every field.

The fields which are not marked will not be included in the resulting dataset.

**Exclude gaps** checkbox allows not to include in the dataset those records which contain gaps (unknown values).

|    | N1  | N2  | N3  | N4  | IRIS-SETOS      |
|----|-----|-----|-----|-----|-----------------|
| 39 | 5.1 |     |     |     |                 |
| 40 | 5   |     |     |     |                 |
| 41 | 4.5 |     |     |     |                 |
| 42 | 4.4 |     |     |     |                 |
| 43 | 5   |     |     |     |                 |
| 44 | 5.1 |     |     |     |                 |
| 45 | 4.8 |     |     |     |                 |
| 46 | 5.1 |     |     |     |                 |
| 47 | 4.6 | 3.2 | 1.4 | 0.2 | Iris            |
| 48 | 5.3 | 3.7 | 1.5 | 0.2 | Iris            |
| 49 | 5   | 3.3 | 1.4 | 0.2 | Iris            |
| 50 | 7   | 3.2 | 4.7 | 1.4 | Iris            |
| 51 | 6.4 | 3.2 | 4.5 | 1.5 | Iris            |
| 52 | 6.9 | 3.1 | 4.9 | 1.5 | Iris            |
| 53 | 5.5 | 2.3 | 4   | 1.3 | Iris            |
| 54 | 6.5 | 2.8 | 4.6 | 1.5 | Iris            |
| 55 | 5.7 | 2.8 | 4.5 | 1.3 | Iris            |
| 56 | 6.3 | 3.3 | 4.7 | 1.6 | Iris            |
| 57 | 4.9 | 2.4 | 3.3 | 1   | Iris            |
| 58 | 6.6 | 2.9 | 4.6 | 1.3 | Iris            |
| 59 | 5.2 | 2.7 | 3.9 | 1.4 | Iris            |
| 60 | 5   | 2   | 3.5 | 1   | Iris-versicolor |
| 61 | 5.9 | 3   | 4.2 | 1.5 | Iris-versicolor |
| 62 | 6   | 2.2 | 4   | 1   | Iris-versicolor |
| 63 | 6.1 | 2.9 | 4.7 | 1.4 | Iris-versicolor |



## VIDAEXPERT: WORKING WITH DATASET

The screenshot displays the VidaExpert application window. The main area shows a table titled "Таблица - iris.vet" with 25 rows of data. The columns are labeled N1, N2, N3, N4, and IRIS-SETOS. The data represents the Iris dataset, with the last column listing the species as "Iris-setosa".

On the right side, the Object Manager shows a tree structure with "iris" as the root, containing "Tables" (with "iris.vet" listed) and "Data" (with "Datasets01" listed). A yellow arrow points from a text box to the "Datasets01" entry.

A text box with a yellow border contains the following text:

After creating dataset, click on it in Object Manager, and click on **Create Map** button.

The "Create Map" button is located in the bottom right corner of the interface, represented by a red icon with a green plus sign.

|    | N1  | N2  | N3  | N4  | IRIS-SETOS  |
|----|-----|-----|-----|-----|-------------|
| 1  | 4.9 | 3   | 1.4 | 0.2 | Iris-setosa |
| 2  | 4.7 | 3.2 | 1.3 | 0.2 | Iris-setosa |
| 3  | 4.6 | 3.1 | 1.5 | 0.2 | Iris-setosa |
| 4  | 5   | 3.7 | 1.6 | 0.4 | Iris-setosa |
| 5  | 5.4 | 3.7 | 1.5 | 0.2 | Iris-setosa |
| 6  | 4.6 | 3.1 | 1.5 | 0.2 | Iris-setosa |
| 7  | 5   | 3.7 | 1.6 | 0.4 | Iris-setosa |
| 8  | 4.4 | 2.8 | 1.4 | 0.2 | Iris-setosa |
| 9  | 4.9 | 3.1 | 1.5 | 0.2 | Iris-setosa |
| 10 | 5.4 | 3.7 | 1.5 | 0.2 | Iris-setosa |
| 11 | 4.8 | 3.4 | 1.6 | 0.2 | Iris-setosa |
| 12 | 4.8 | 3   | 1.4 | 0.1 | Iris-setosa |
| 13 | 4.3 | 3   | 1.1 | 0.1 | Iris-setosa |
| 14 | 5.8 | 4   | 1.2 | 0.2 | Iris-setosa |
| 15 | 5.7 | 4.4 | 1.5 | 0.4 | Iris-setosa |
| 16 | 5.4 | 3.9 | 1.3 | 0.4 | Iris-setosa |
| 17 | 5.1 | 3.5 | 1.4 | 0.3 | Iris-setosa |
| 18 | 5.7 | 3.8 | 1.7 | 0.3 | Iris-setosa |
| 19 | 5.1 | 3.8 | 1.5 | 0.3 | Iris-setosa |
| 20 | 5.4 | 3.4 | 1.7 | 0.2 | Iris-setosa |
| 21 | 5.1 | 3.7 | 1.5 | 0.4 | Iris-setosa |
| 22 | 4.6 | 3.6 | 1   | 0.2 | Iris-setosa |
| 23 | 5.1 | 3.3 | 1.7 | 0.5 | Iris-setosa |
| 24 | 4.8 | 3.4 | 1.9 | 0.2 | Iris-setosa |
| 25 | 5   | 3   | 1.6 | 0.2 | Iris-setosa |

## VIDAEXPERT: WORKING WITH DATASET

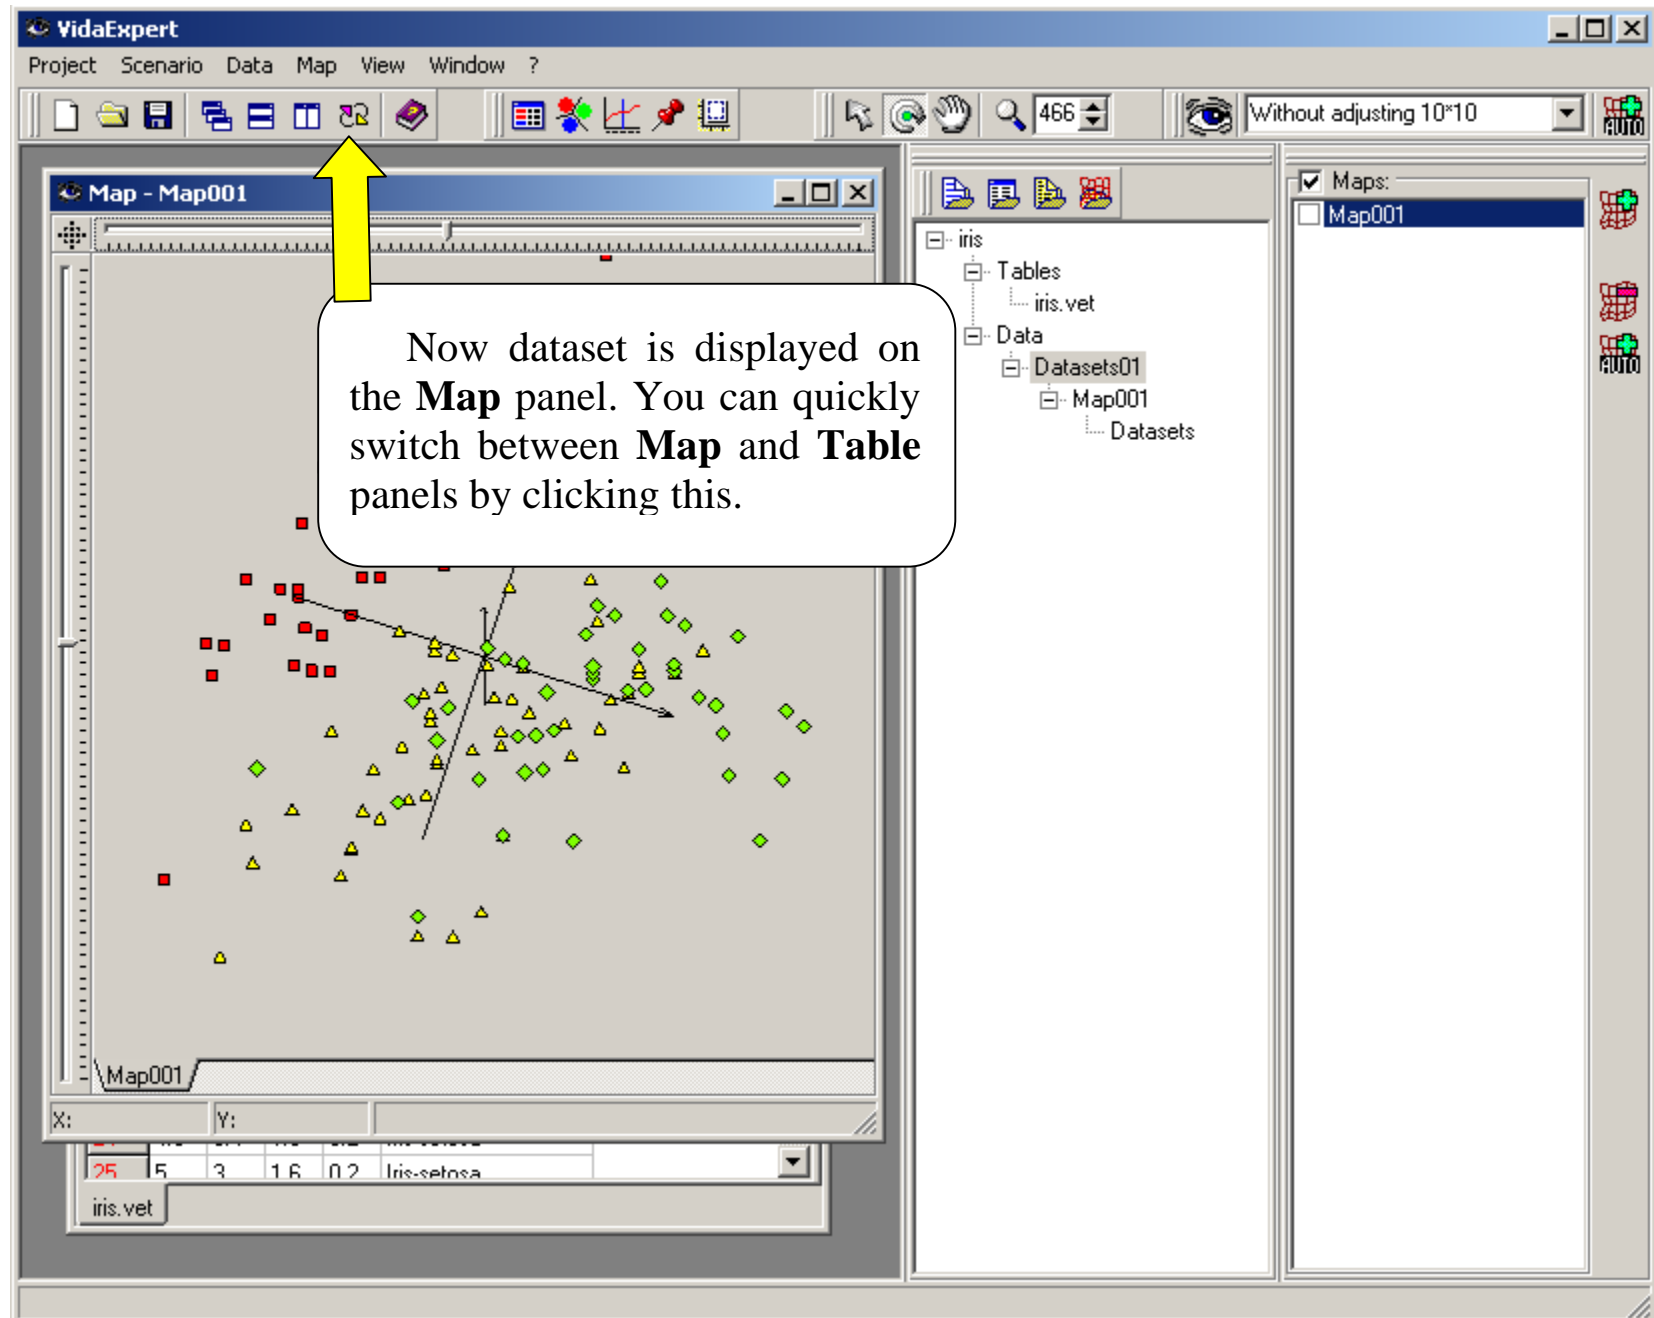

## VIDAEXPERT: WORKING WITH DATASET

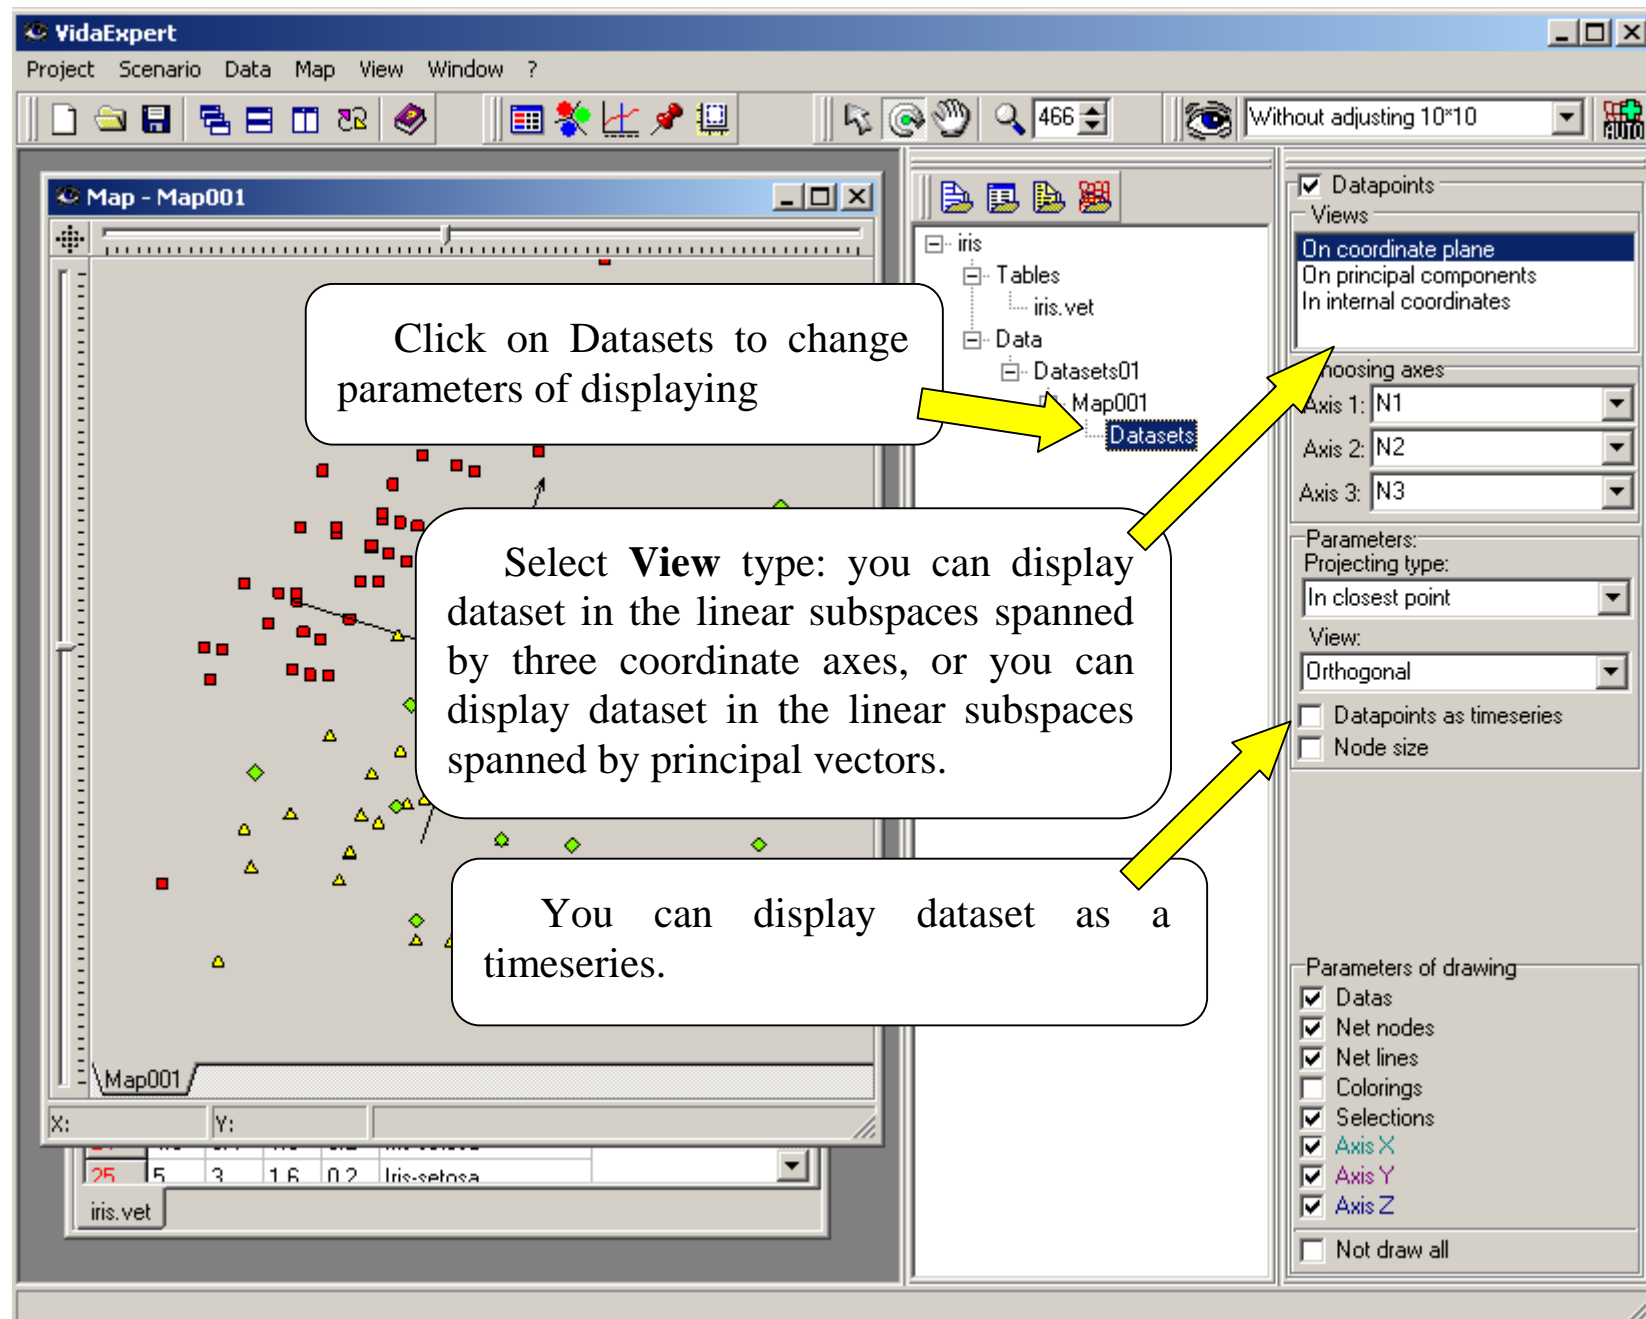



## VIDAEXPERT: WORKING WITH DATASET

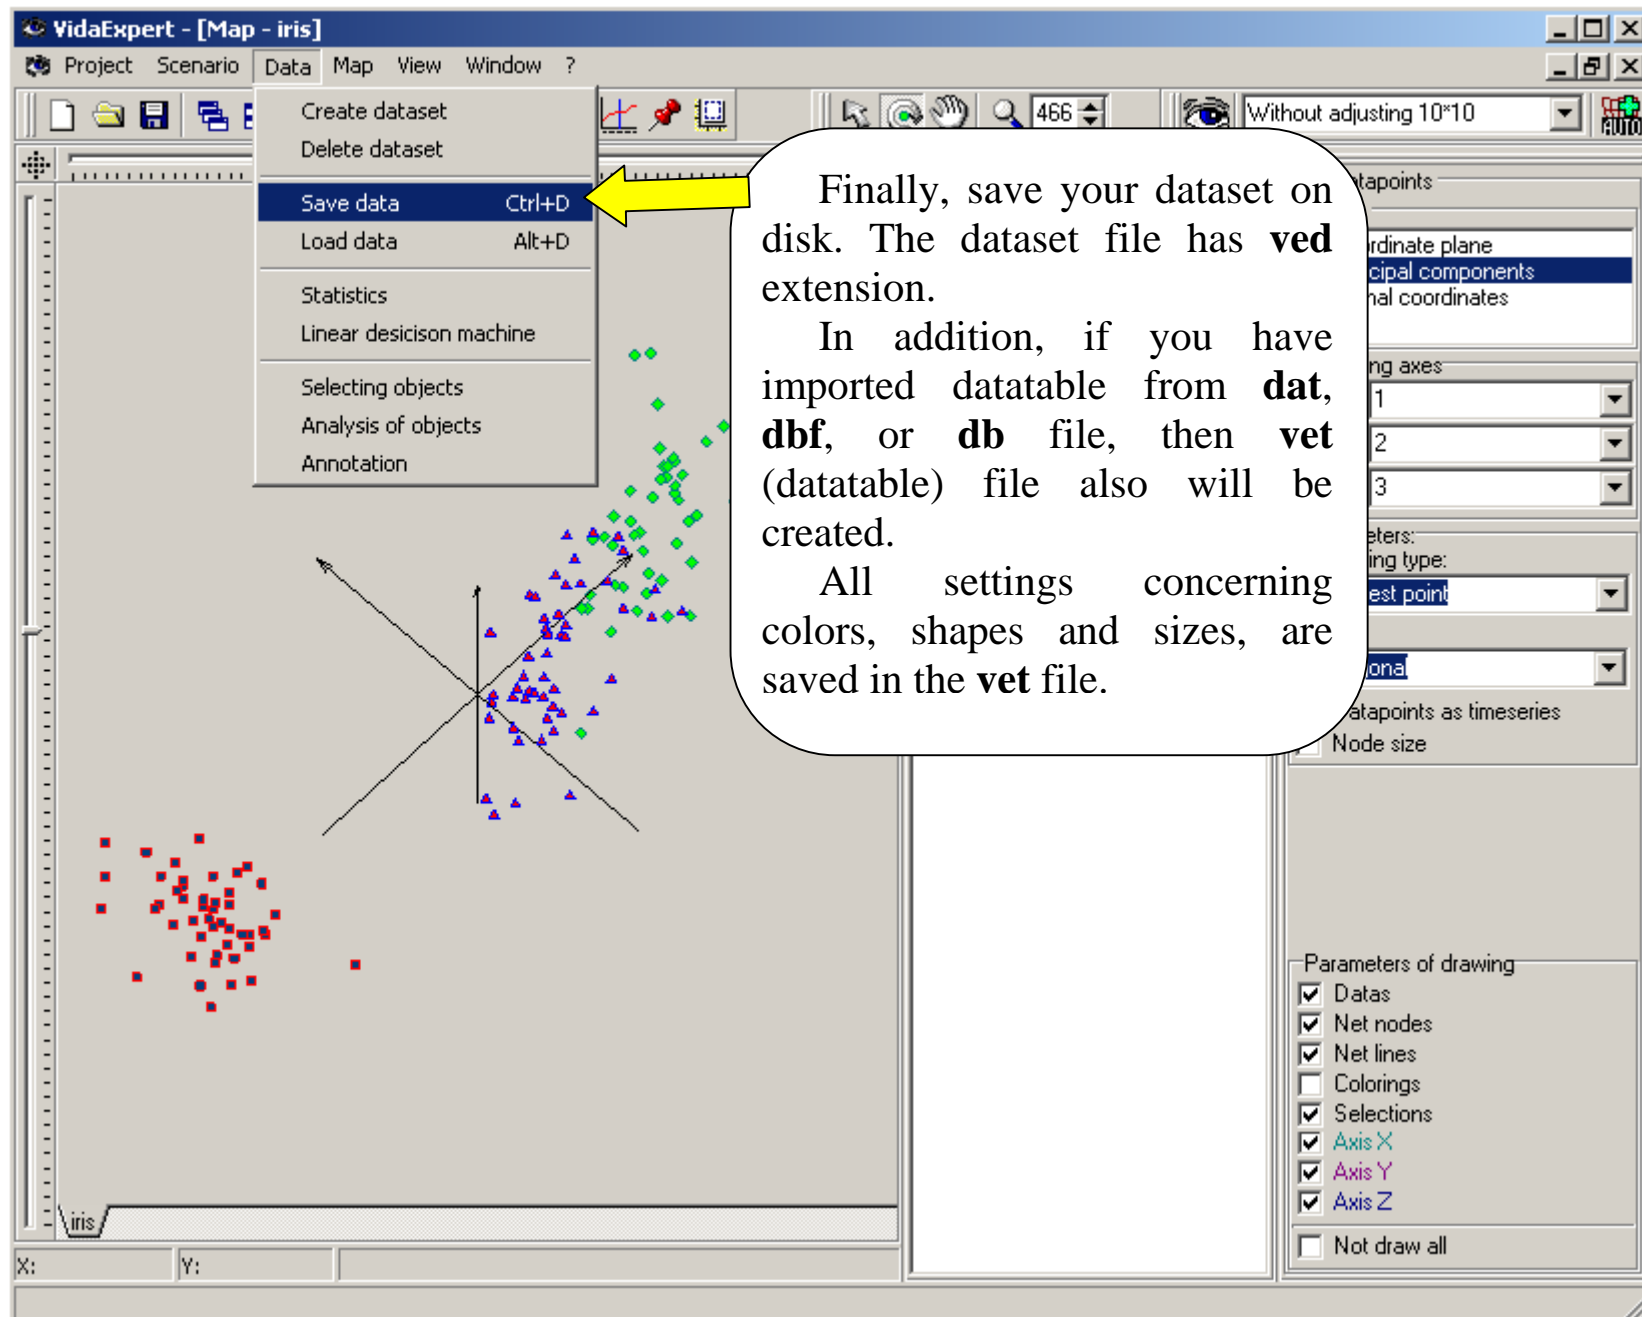

The screenshot shows the VidaExpert software interface. The main window displays a scatter plot with three clusters of data points: red squares, green diamonds, and purple triangles. A yellow arrow points to the 'Save data' option in the 'Data' menu, which is highlighted. The menu also includes 'Create dataset', 'Delete dataset', 'Load data', 'Statistics', 'Linear decision machine', 'Selecting objects', 'Analysis of objects', and 'Annotation'. The right sidebar contains various settings, including 'Datapoints', 'Coordinate plane', 'Principal components', 'Principal coordinates', 'Drawing axes', 'Parameters', 'Drawing type', 'Test point', 'Dona', 'Datapoints as timeseries', 'Node size', and 'Parameters of drawing'.

Finally, save your dataset on disk. The dataset file has **ved** extension.

In addition, if you have imported datatable from **dat**, **dbf**, or **db** file, then **vet** (datatable) file also will be created.

All settings concerning colors, shapes and sizes, are saved in the **vet** file.

## VIDAEXPERT: DATASET VISUALIZATION

The screenshot displays the VidaExpert application window. The main workspace shows a scatter plot of data points (yellow squares, red triangles, and green circles) on a grid. A yellow arrow points from a text box to the 'iris1' dataset in the Object Manager Panel. Another yellow arrow points from the same text box to the 'See It!' button in the map type selection menu. A third yellow arrow points from the 'See It!' button to the 'Rigid map 12\*12' option in the same menu.

After creating dataset (or loading saved dataset) you can create **elastic map**.  
First, select the dataset in Object Manager Panel.

Then choose appropriate map type. For the first preliminary visualization, type "Rigid 12\*12" can be recommended.  
Then click "See It!" button.

The interface includes a menu bar (Project, Scenario, Data, Map, View, Window, ?), a toolbar with various icons, and a status bar at the bottom with X and Y coordinates.

## VIDAEXPERT: DATASET VISUALIZATION

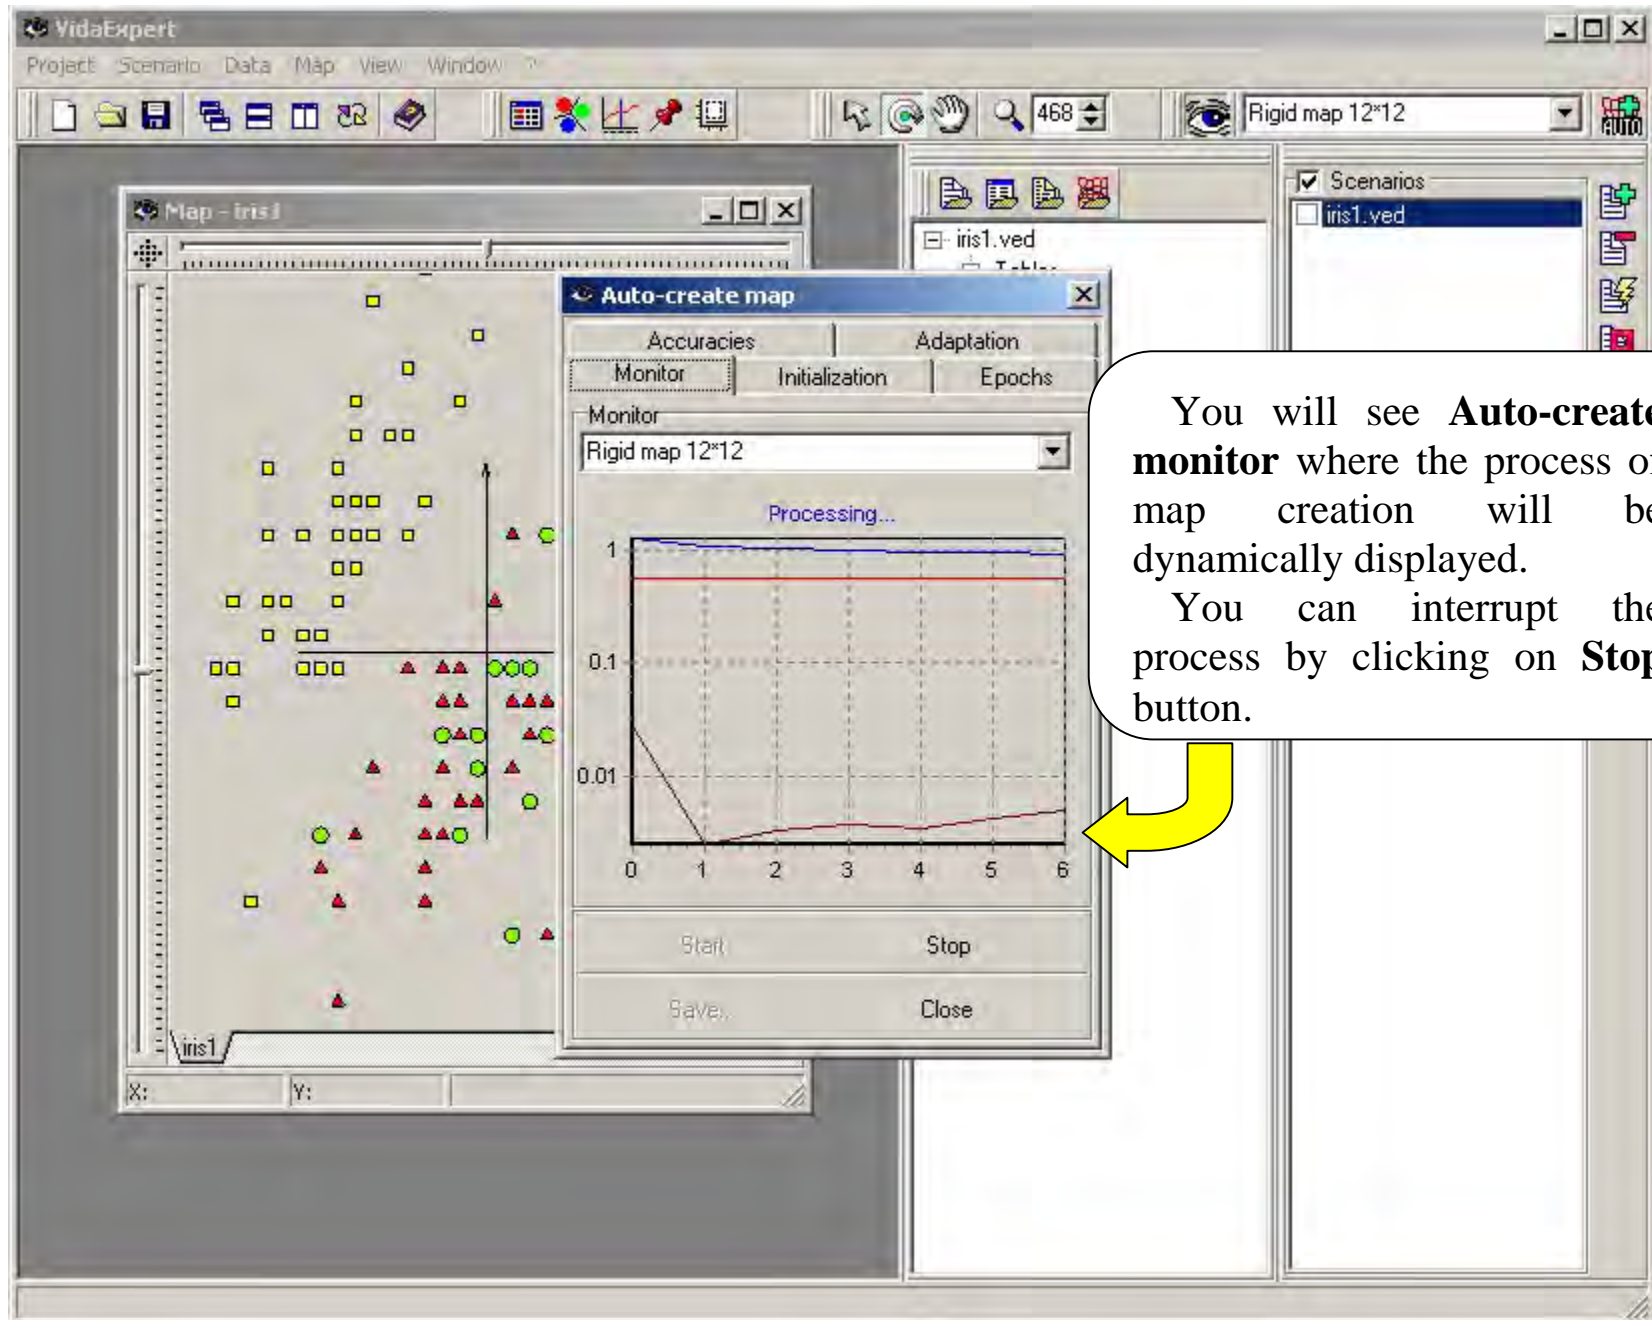



## VIDAEXPERT: DATASET VISUALIZATION

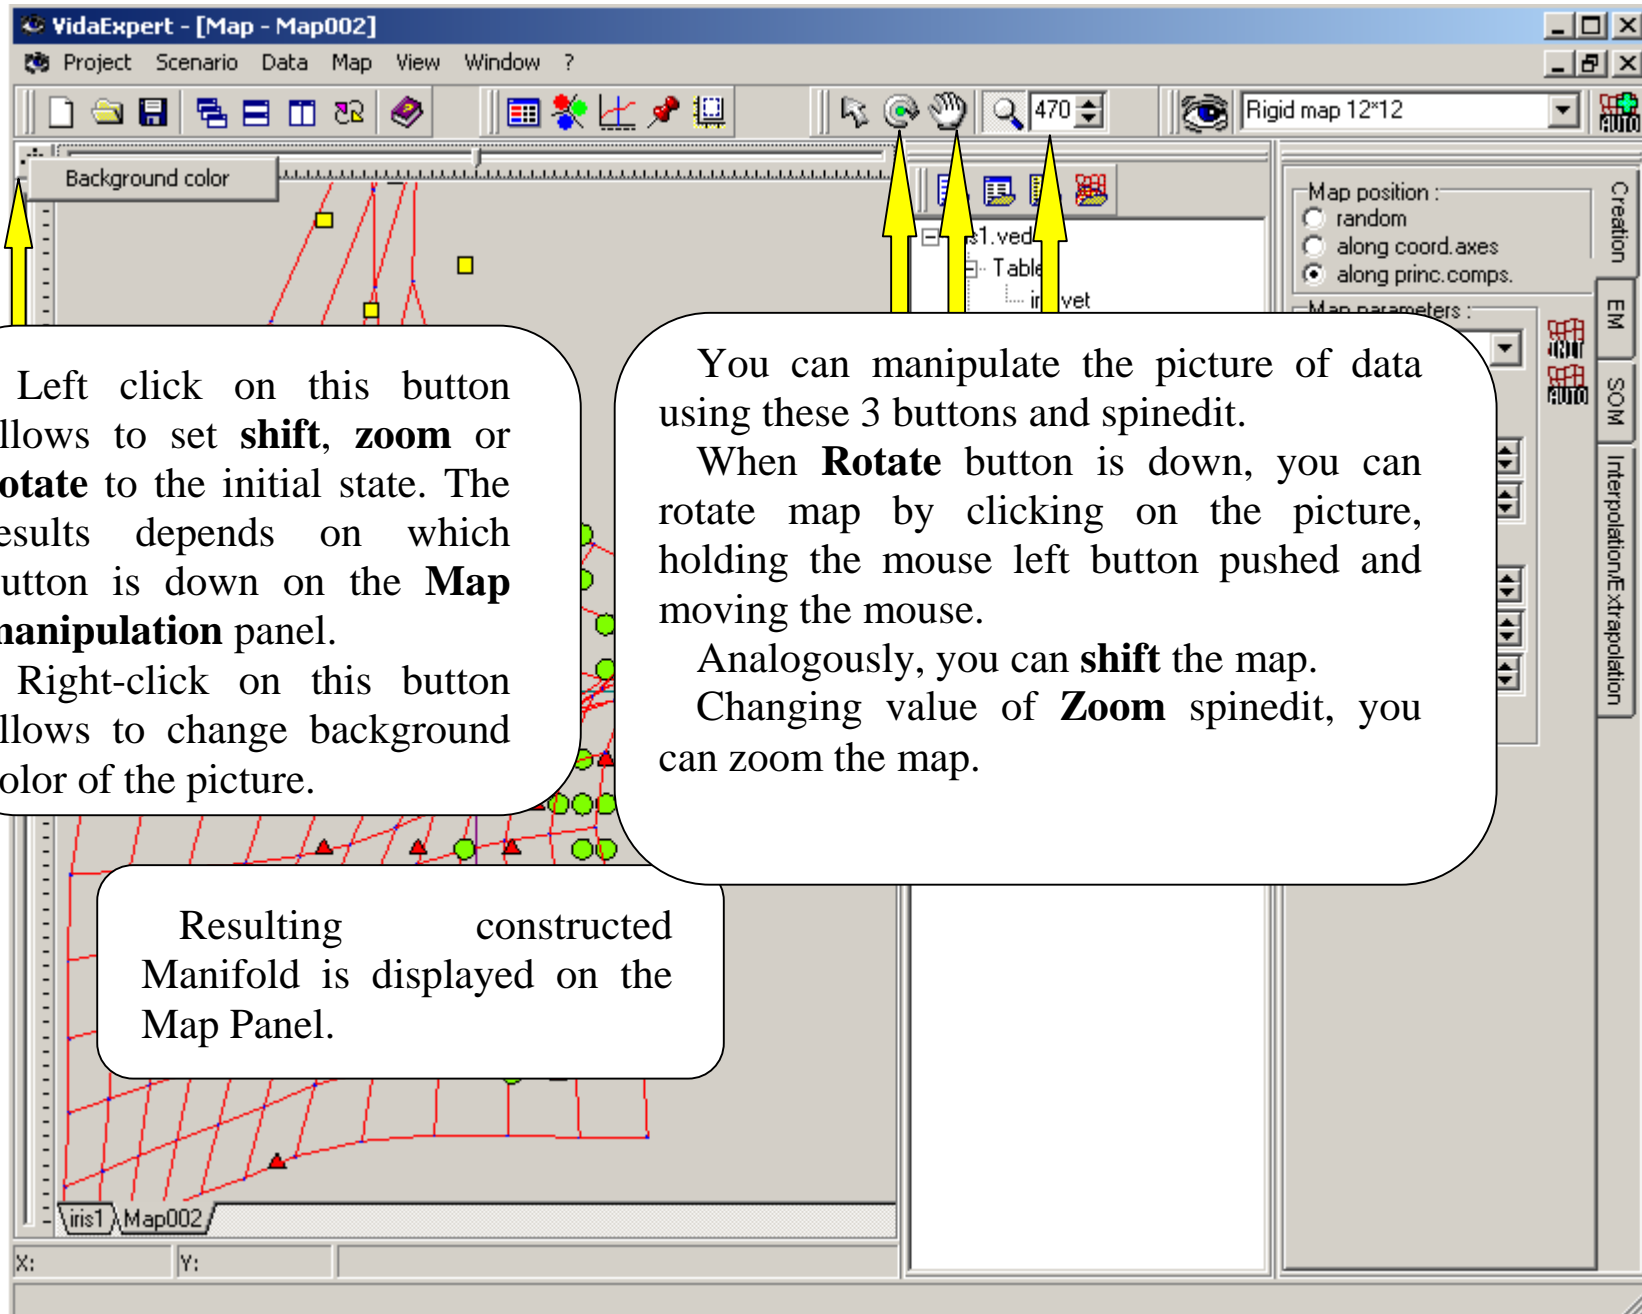

## VIDAEXPERT: DATASET VISUALIZATION

The screenshot displays the VidaExpert software interface. The main window shows a 3D plot of data points (green circles, red triangles, and yellow squares) on a grid. A yellow arrow points from a text box to the 'Datasets' section in the right-hand panel. Another yellow arrow points from a text box to the 'Parameters of drawing' section in the right-hand panel.

**Click on **Datasets** section to change parameters of displaying the dataset.**

**Choose and specify 3D space for displaying the dataset.**  
**Specify which elements of the picture need to be displayed.**

**Right-hand panel configuration:**

- Datapoints:**
  - ☒ Views
    - ☒ On coordinate plane
    - ☐ On principal components
    - ☐ In internal coordinates
- Choosing axes:**
  - Axis 1: N1
  - Axis 2: N2
  - Axis 3: N3
- Parameters:**
  - Projecting type: In closest point
  - View: Orthogonal
  - ☐ Datapoints as timeseries
  - ☐ Node size
- Parameters of drawing:**
  - ☒ Datas
  - ☒ Net nodes
  - ☒ Net lines
  - ☐ Colorings
  - ☒ Selections
  - ☒ Axis X
  - ☒ Axis Y
  - ☒ Axis Z
  - ☐ Not draw all

## VIDAEXPERT: DATASET VISUALIZATION

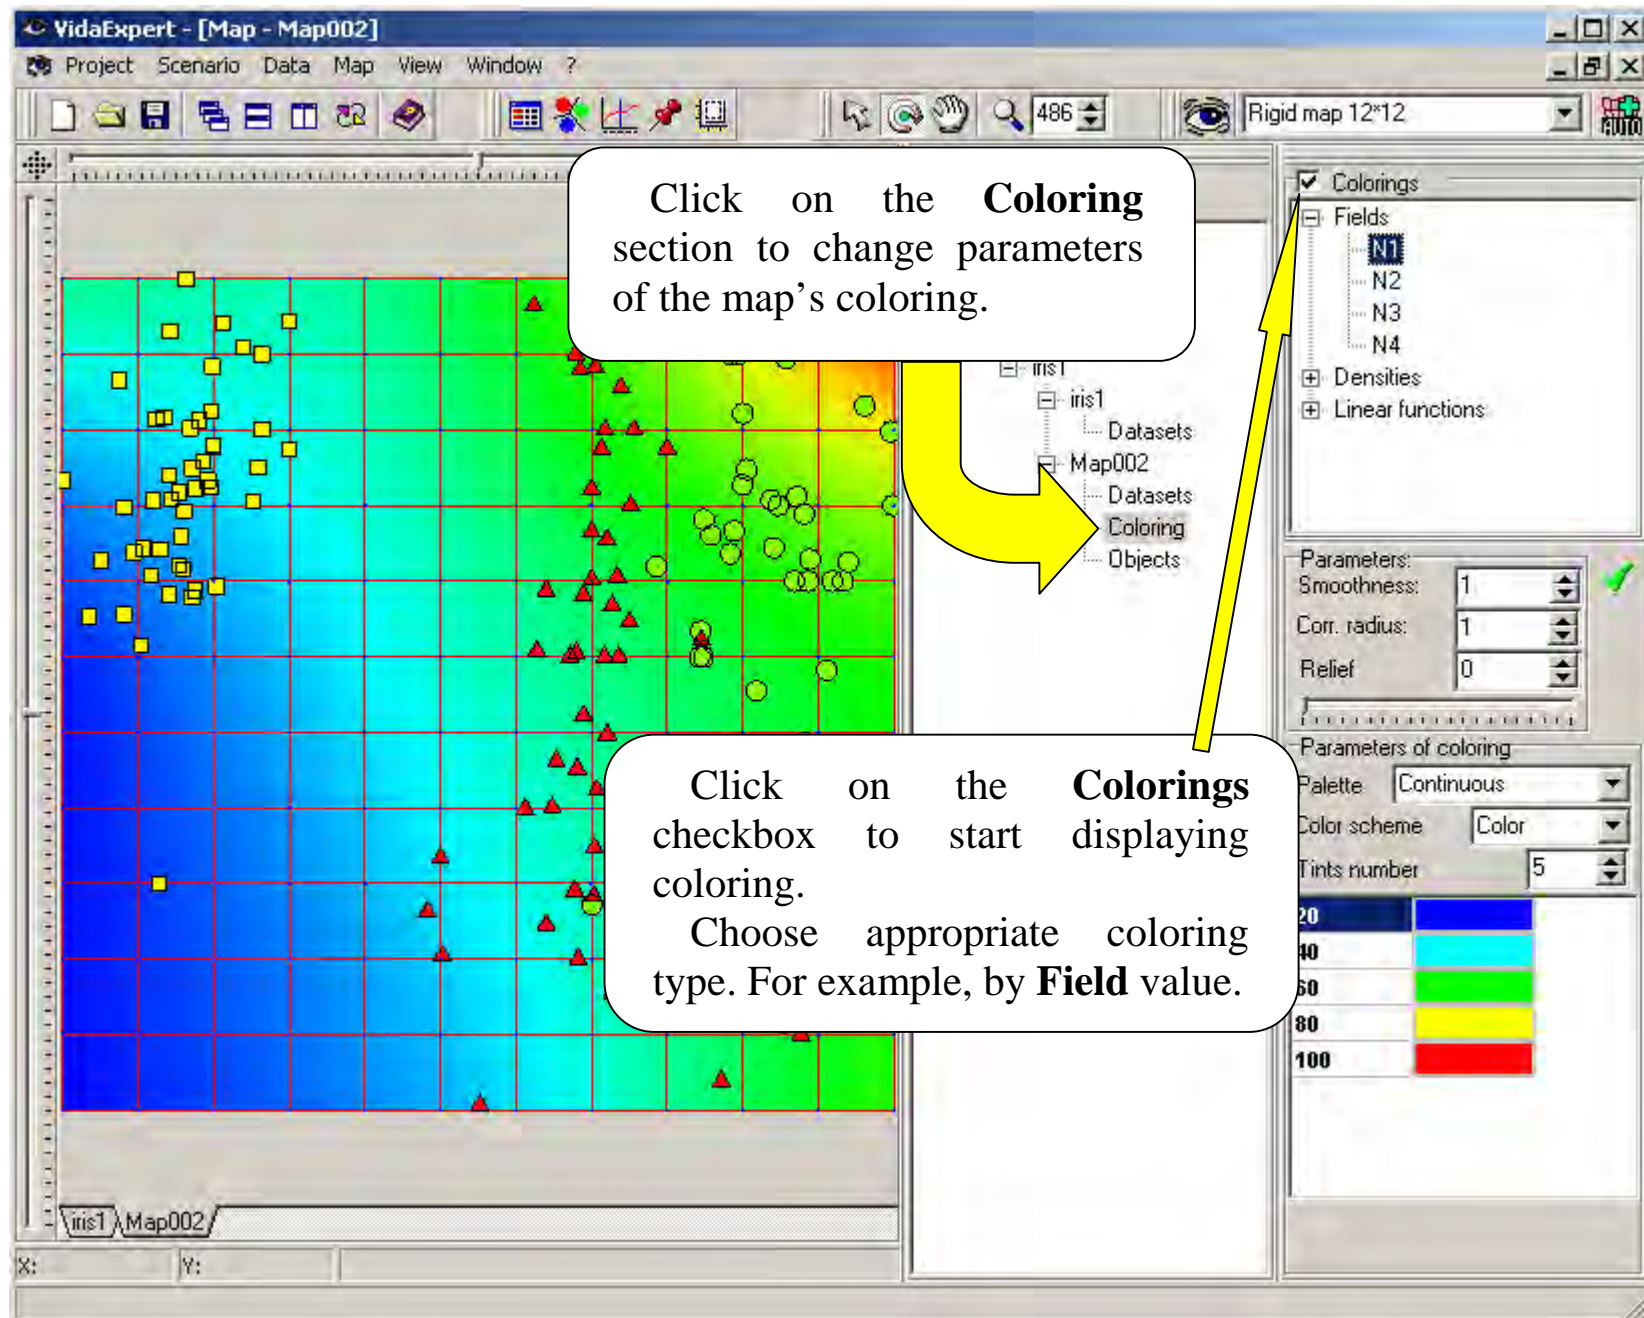

## VIDAEXPERT: DATASET VISUALIZATION

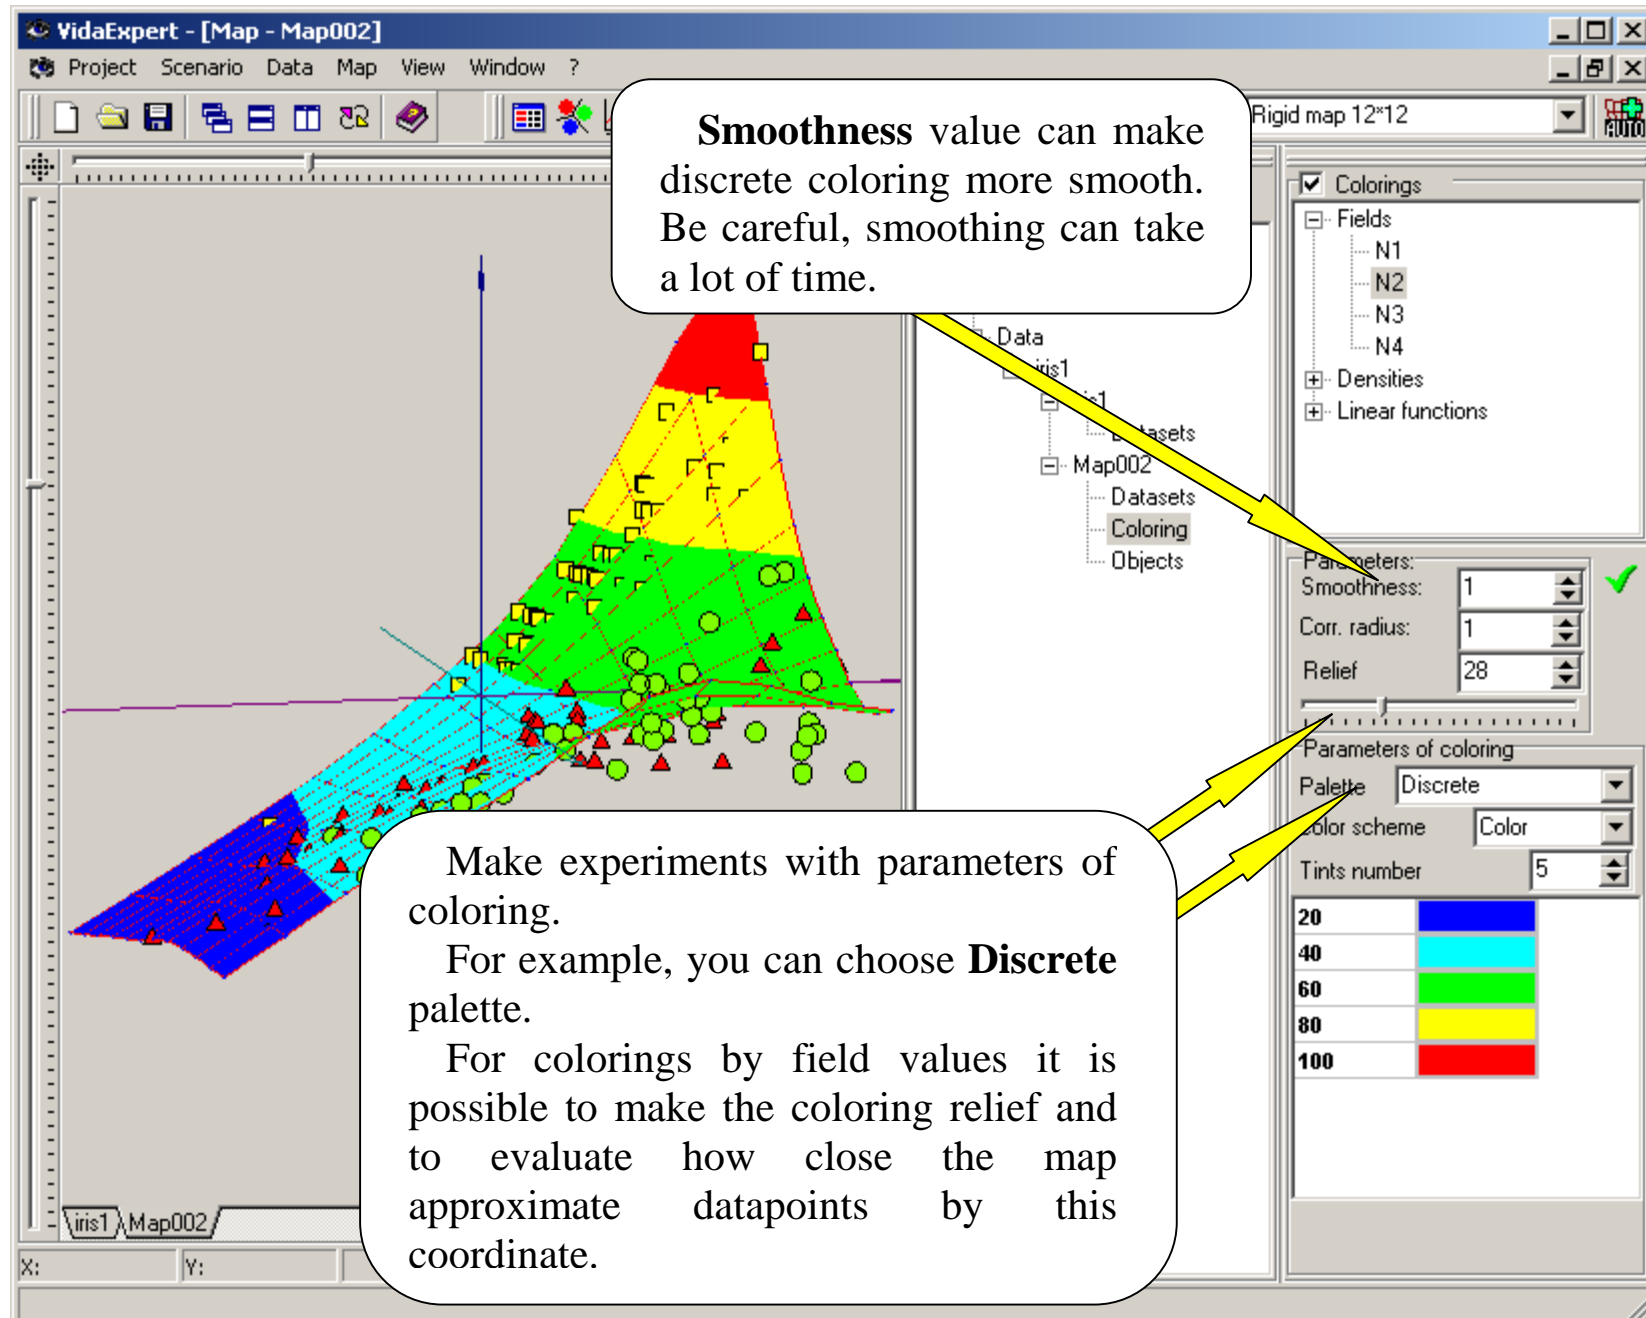



## VIDAEXPERT: DATASET VISUALIZATION

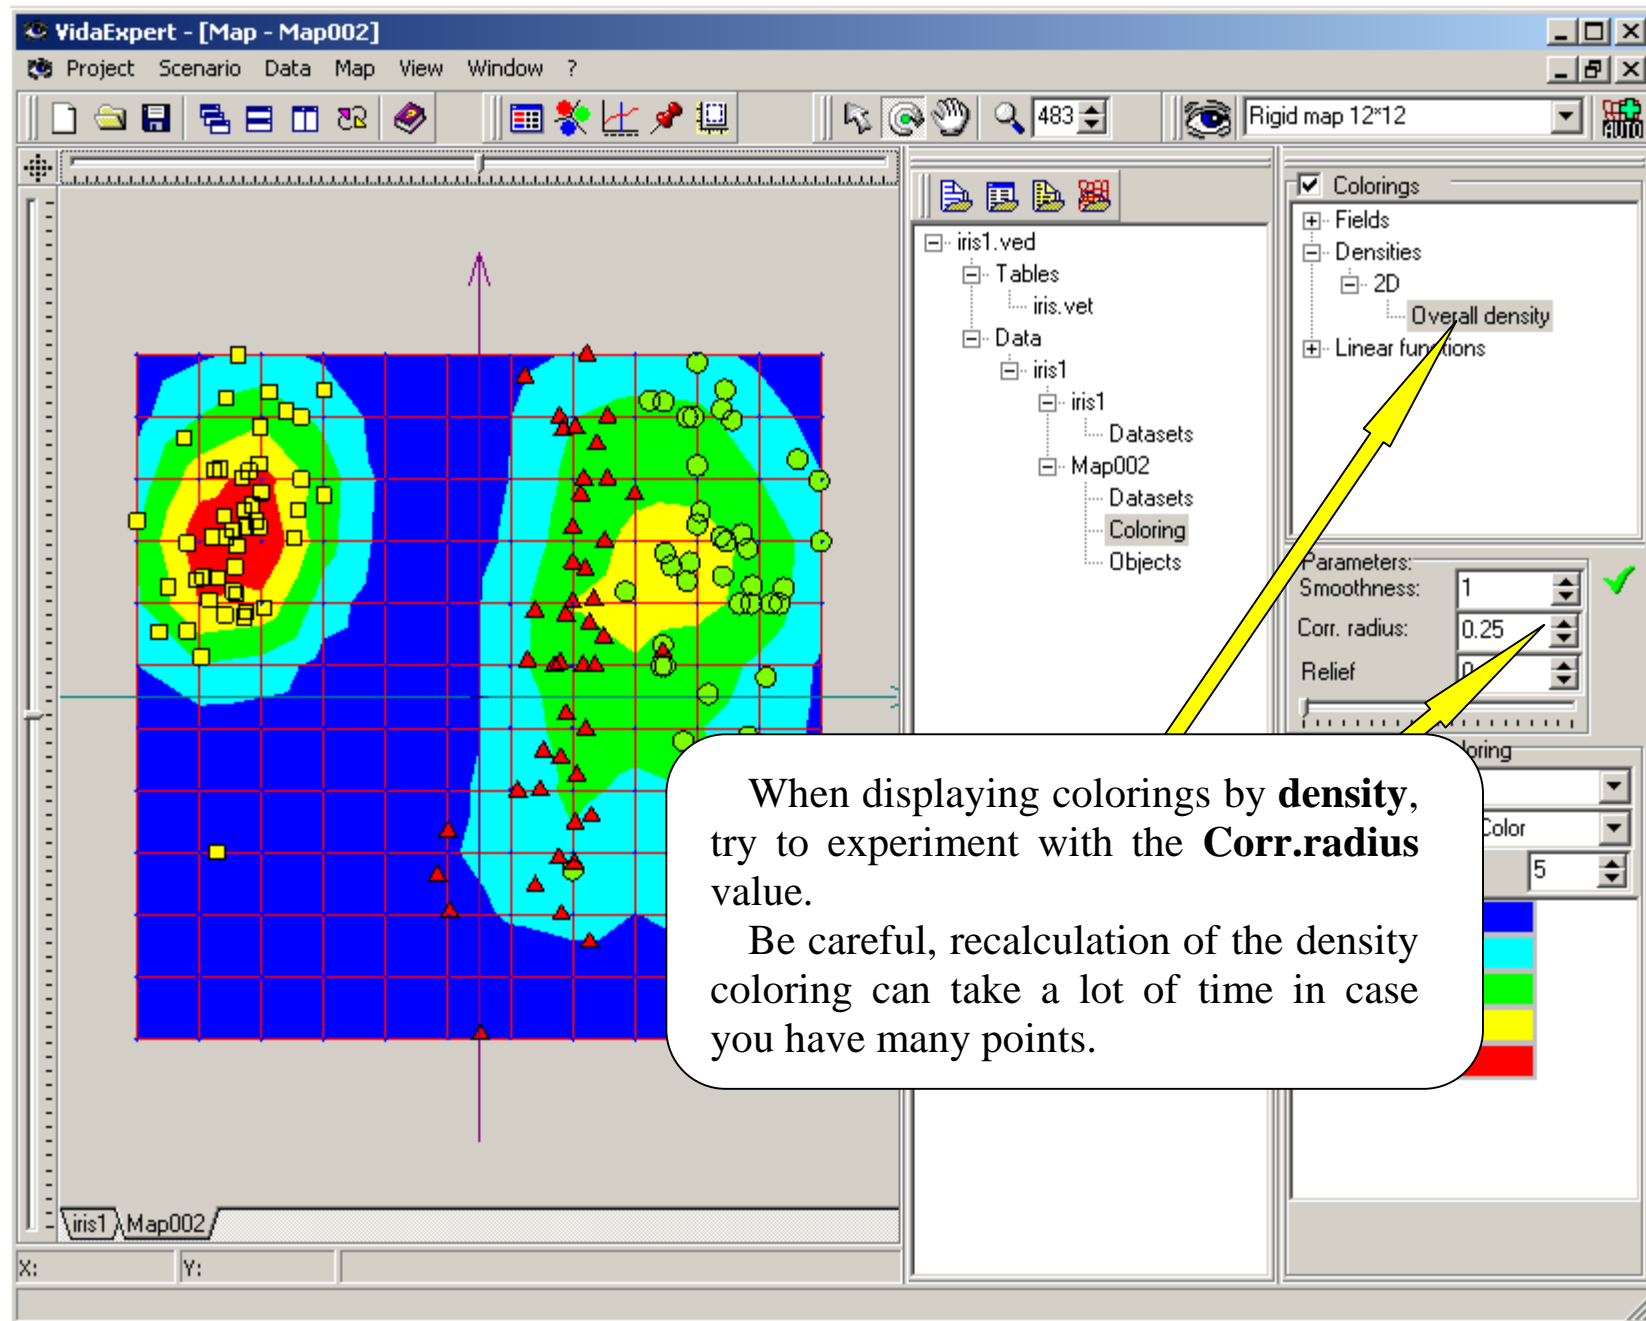

## VIDAEXPERT: DATASET VISUALIZATION

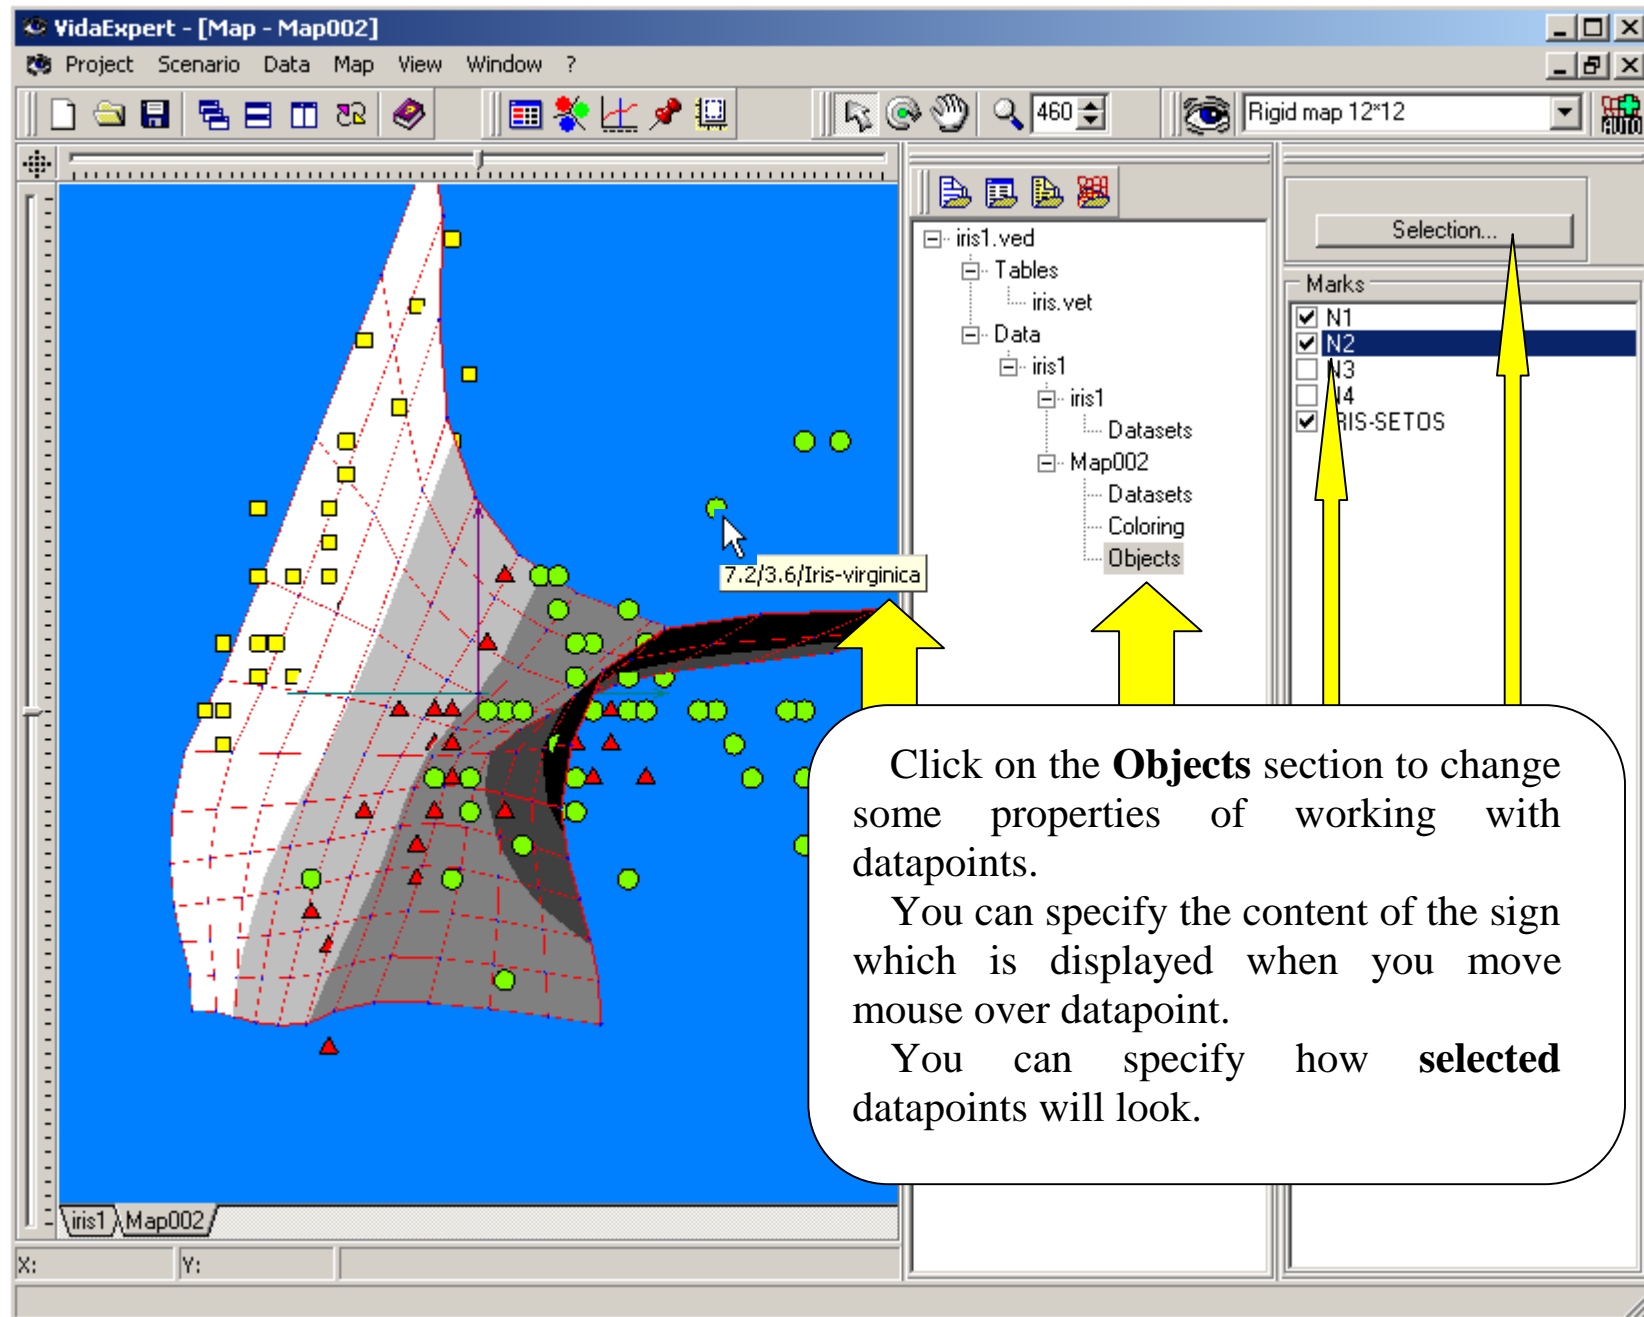

## VIDAEXPERT: DATASET VISUALIZATION

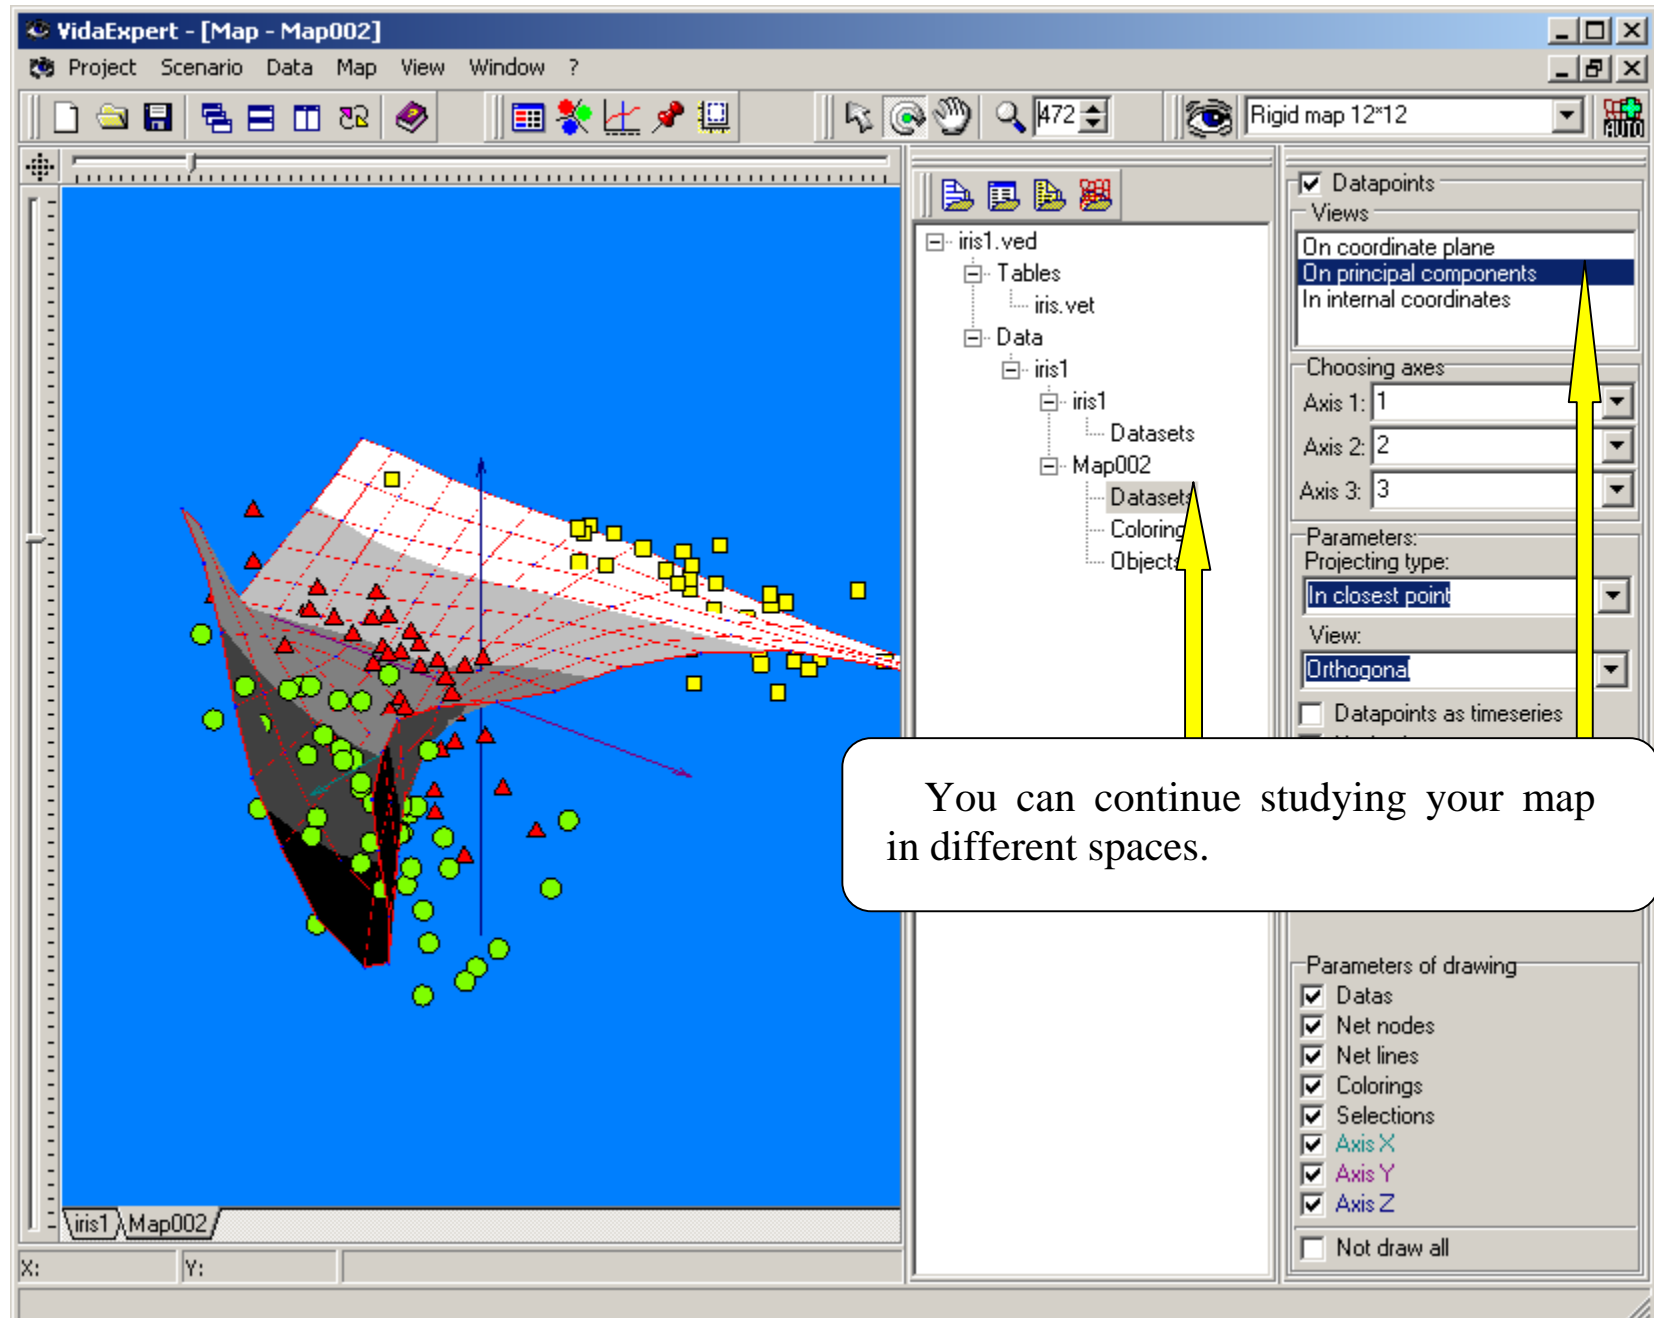

## VIDAEXPERT: DATASET VISUALIZATION

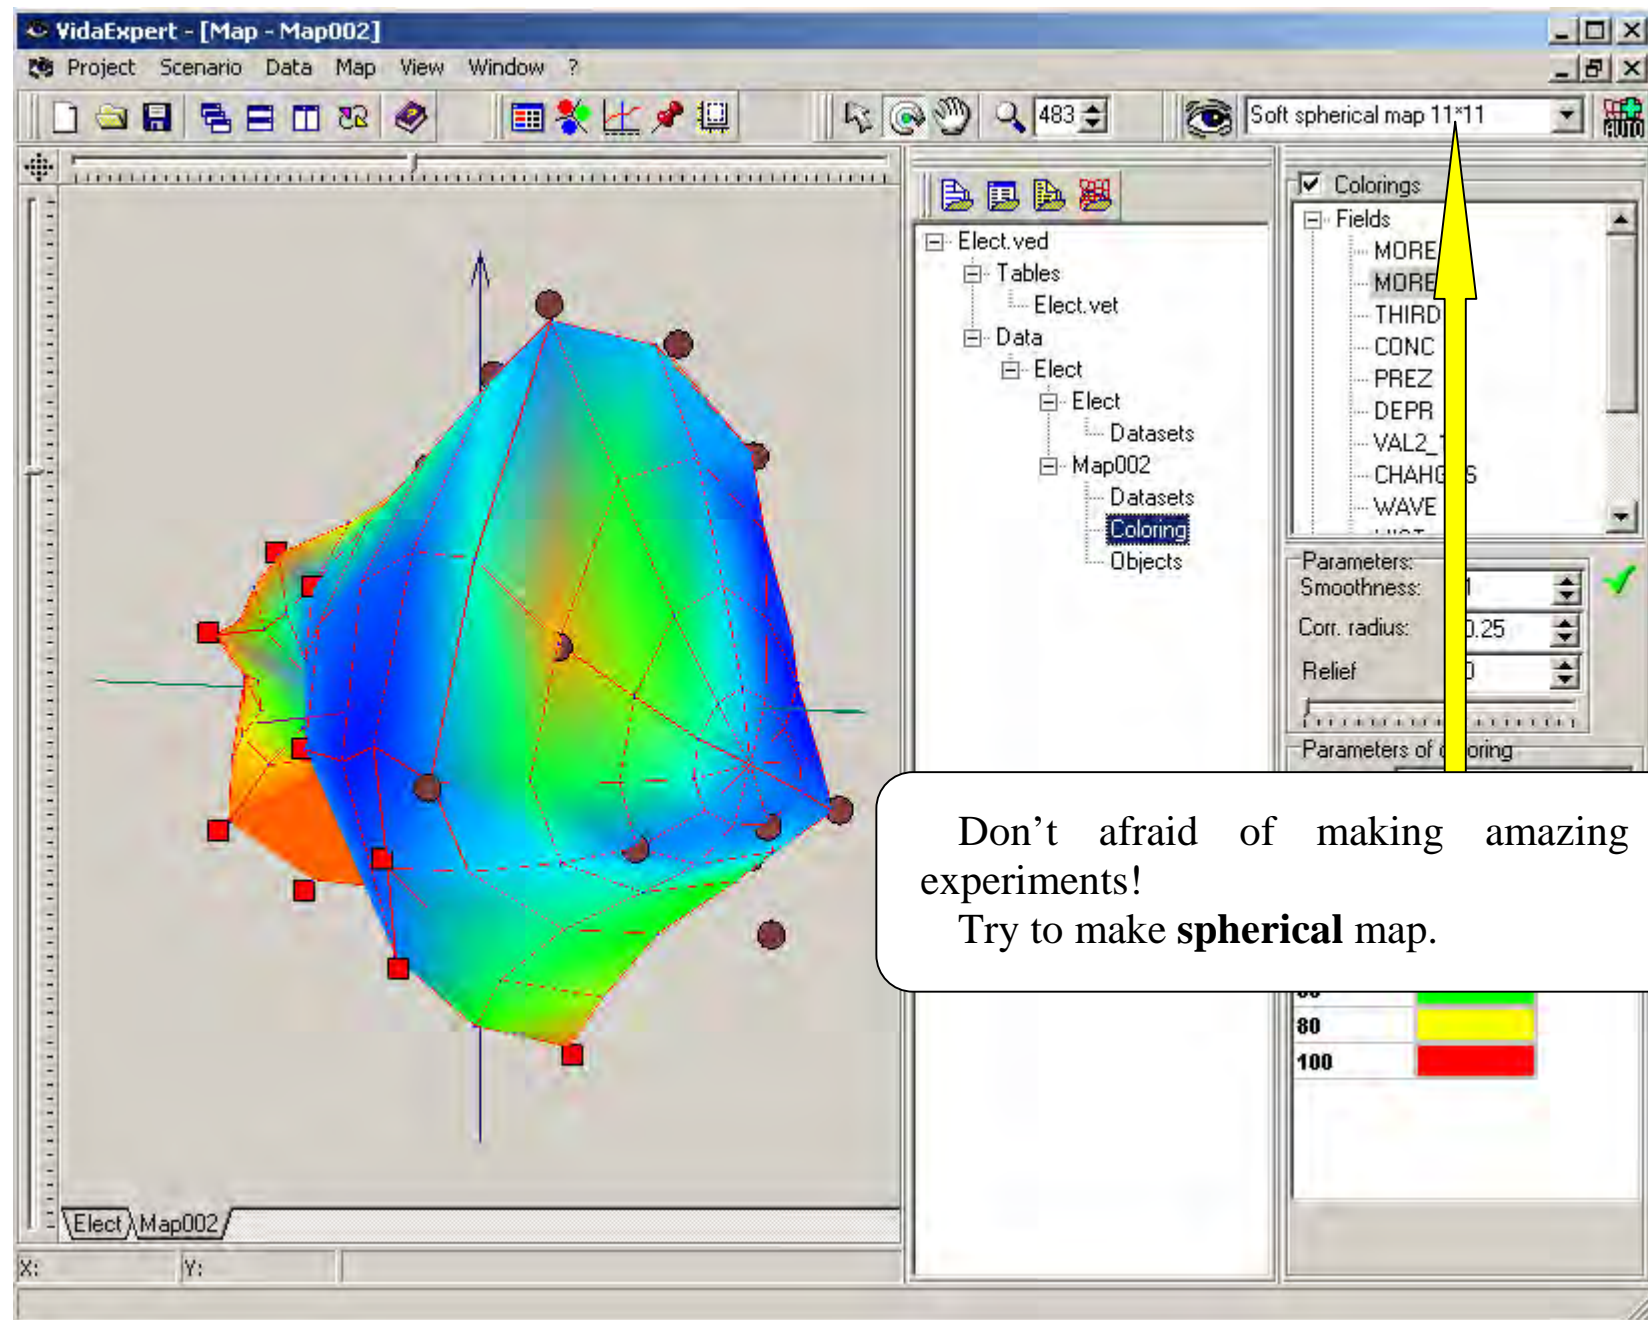



## VIDAEXPERT: DATASET VISUALIZATION

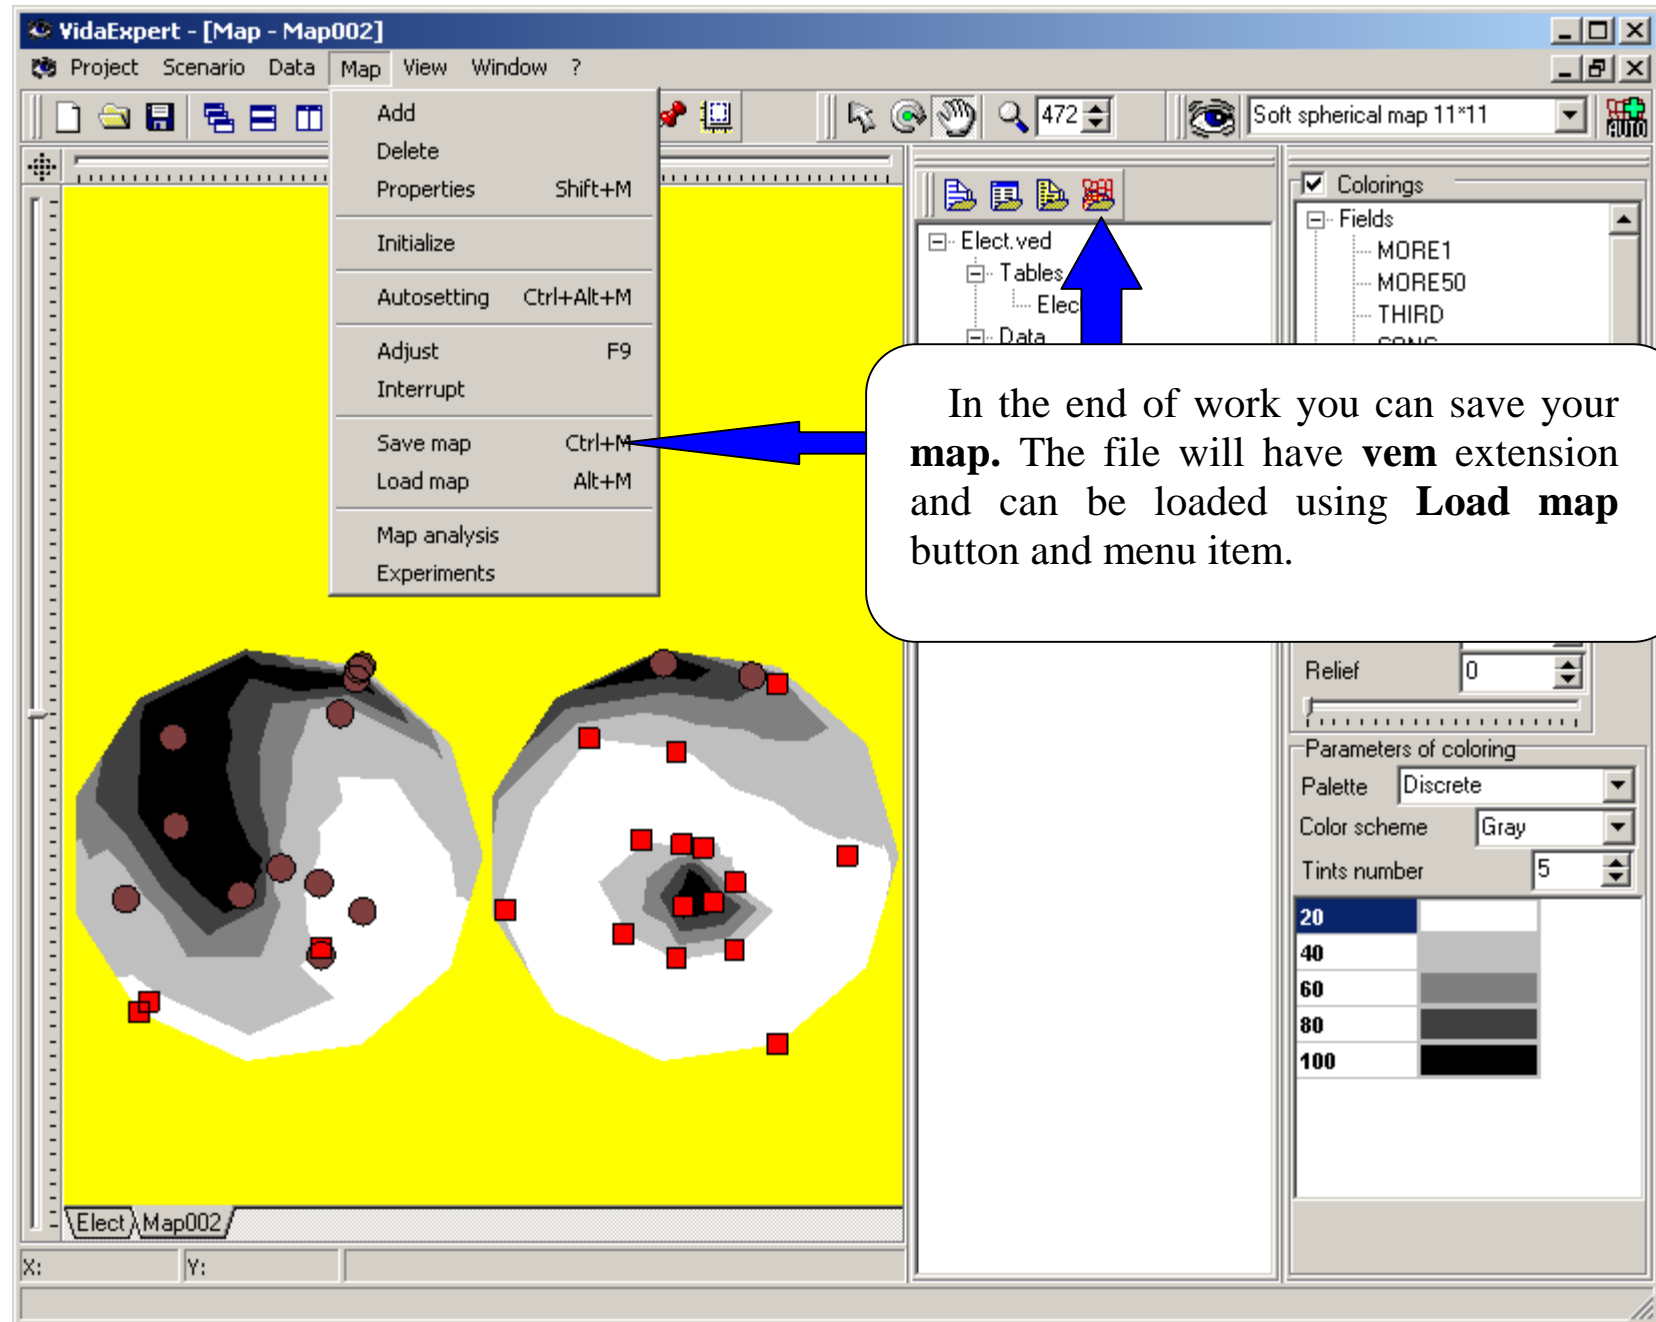

## VIDAEXPERT: DATA ANALYSIS

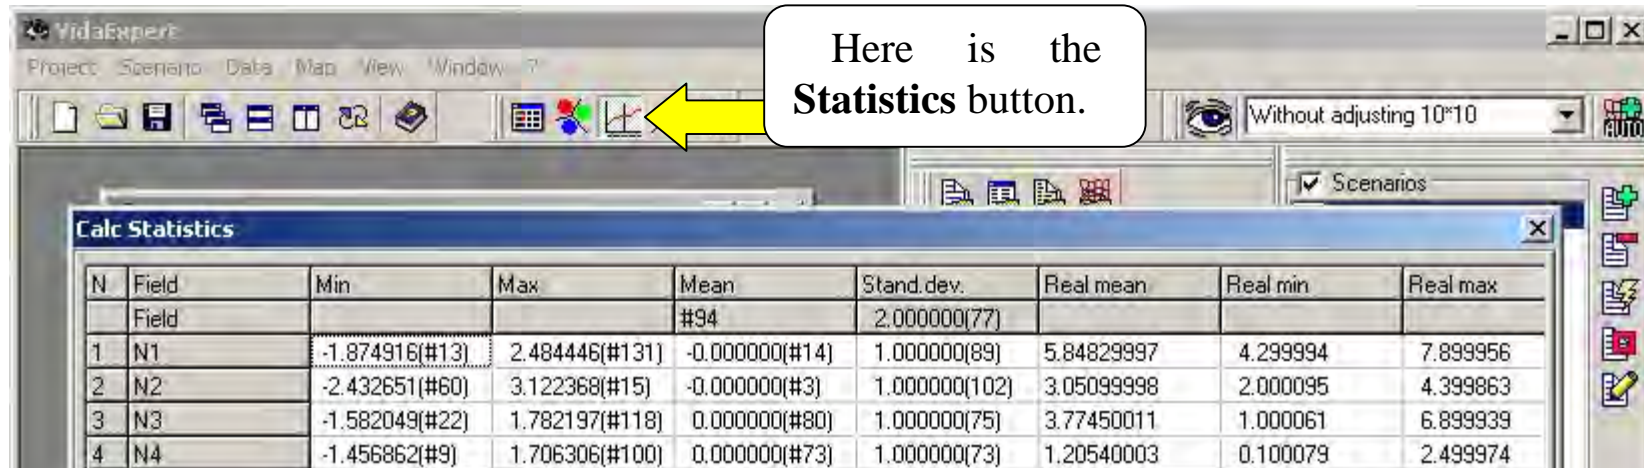

After creating dataset you can analyze it in different ways. First, you can calculate statistics. Open **Statistics** dialog, **Common** tabsheet, click **Calculate**.

**Min, Max:** minimal and maximal field values after **normalization**. The numbers in parentheses with # symbol mean the numbers of the record where the maximum and minimum values were reached.

The same with **Mean**. The number just below the **Mean** word means the number of object closest to the average point.

**Stand.dev.:** standard deviations after **normalization**. The numbers in parentheses indicate how many objects are in the interval  $(m-\sigma, m+\sigma)$ , where  $m$  – average,  $\sigma$  – standard deviation. The number just below the **Stand.dev.** word means overall standard deviation.

**Real min. Real max. Real mean** – Mean. Max. Mean values **before normalization**.

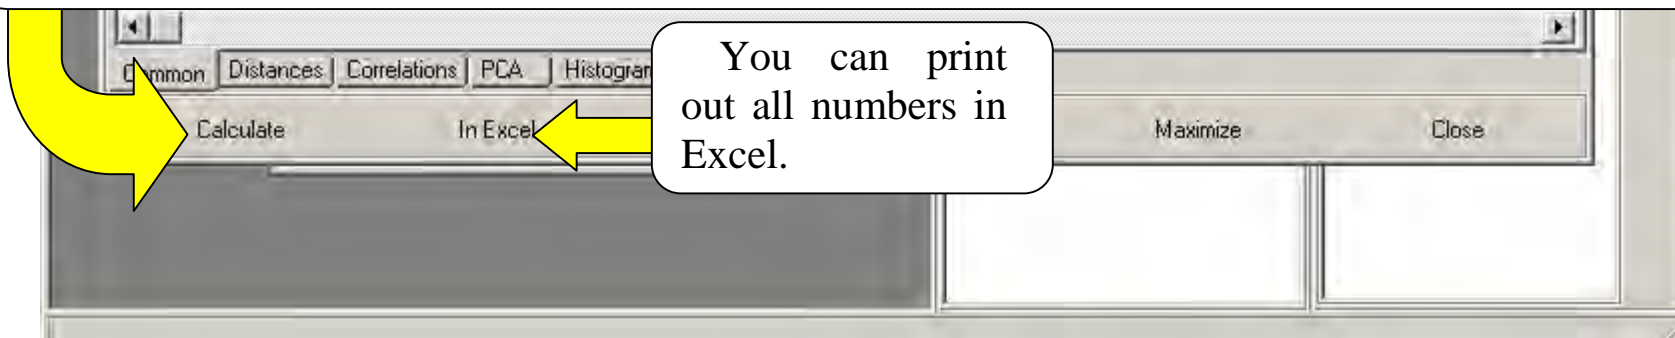

## VIDAEXPERT: DATA ANALYSIS

**Calc Statistics**

|    | 0        | 1        | 2        | 3        | 4        | 5        | 6        | 7        | 8        | 9        |
|----|----------|----------|----------|----------|----------|----------|----------|----------|----------|----------|
| 0  |          |          |          |          |          |          |          |          |          |          |
| 1  | 0.525547 |          |          |          |          |          |          |          |          |          |
| 2  | 0.434508 | 0.285032 |          |          |          |          |          |          |          |          |
| 3  | 1.394024 | 0.996191 | 1.255868 |          |          |          |          |          |          |          |
| 4  | 2.191980 | 1.861481 | 2.109420 | 0.903063 |          |          |          |          |          |          |
| 5  | 1.003253 | 0.499579 | 0.709072 | 0.682849 | 1.524610 |          |          |          |          |          |
| 6  | 0.935462 | 0.599392 | 0.846628 | 0.466417 | 1.287027 | 0.505213 |          |          |          |          |
| 7  | 0.648199 | 0.785738 | 0.525546 | 1.775664 | 2.631052 | 1.189689 | 1.367653 |          |          |          |
| 8  | 0.272389 | 0.377630 | 0.386450 | 1.172442 | 1.991137 | 0.828775 | 0.717074 | 0.775567 |          |          |
| 9  | 1.730588 | 1.439046 | 1.693255 | 0.539854 | 0.544777 | 1.200522 | 0.846627 | 2.213211 | 1.520724 |          |
| 10 | 0.940661 | 0.508153 | 0.737609 | 0.534746 | 1.392823 | 0.298381 | 0.248809 | 1.259745 | 0.719338 | 1.006628 |
| 11 | 0.178982 | 0.499580 | 0.364486 | 1.415862 | 2.247872 | 0.992629 | 0.967704 | 0.552776 | 0.267373 | 1.781462 |
| 12 | 0.757973 | 0.692307 | 0.504915 | 1.641277 | 2.527276 | 1.043021 | 1.282609 | 0.338926 | 0.795918 | 2.113950 |
| 13 | 2.560878 | 2.281719 | 2.545637 | 1.344861 | 0.662541 | 2.017567 | 1.701874 | 3.060955 | 2.360896 | 0.863737 |
| 14 | 3.392872 | 3.043584 | 3.301163 | 2.054250 | 1.218324 | 2.674369 | 2.478978 | 3.821634 | 3.185703 | 1.681235 |
| 15 | 2.186038 | 1.847455 | 2.109420 | 0.888545 | 0.228085 | 1.516056 | 1.287027 | 2.626105 | 1.991137 | 0.544777 |
| 16 | 1.189689 | 0.8587   |          |          |          |          |          | 1.632338 | 0.994266 | 0.605713 |
| 17 | 2.100904 | 1.861    |          |          |          |          |          | 2.619966 | 1.909465 | 0.464675 |
| 18 | 1.872958 | 1.481    |          |          |          |          |          | 2.253570 | 1.659287 | 0.450463 |
| 19 | 1.119387 | 0.992    |          |          |          |          |          | 1.683733 | 0.937618 | 0.703680 |

Common Distances

Calculate

Maximize Close

Euclidean **Distances** matrix (after normalization). Choose Distances tabsheet, click Calculate. (Not very useful if you have thousands of objects. ;))

## VIDAEXPERT: DATA ANALYSIS

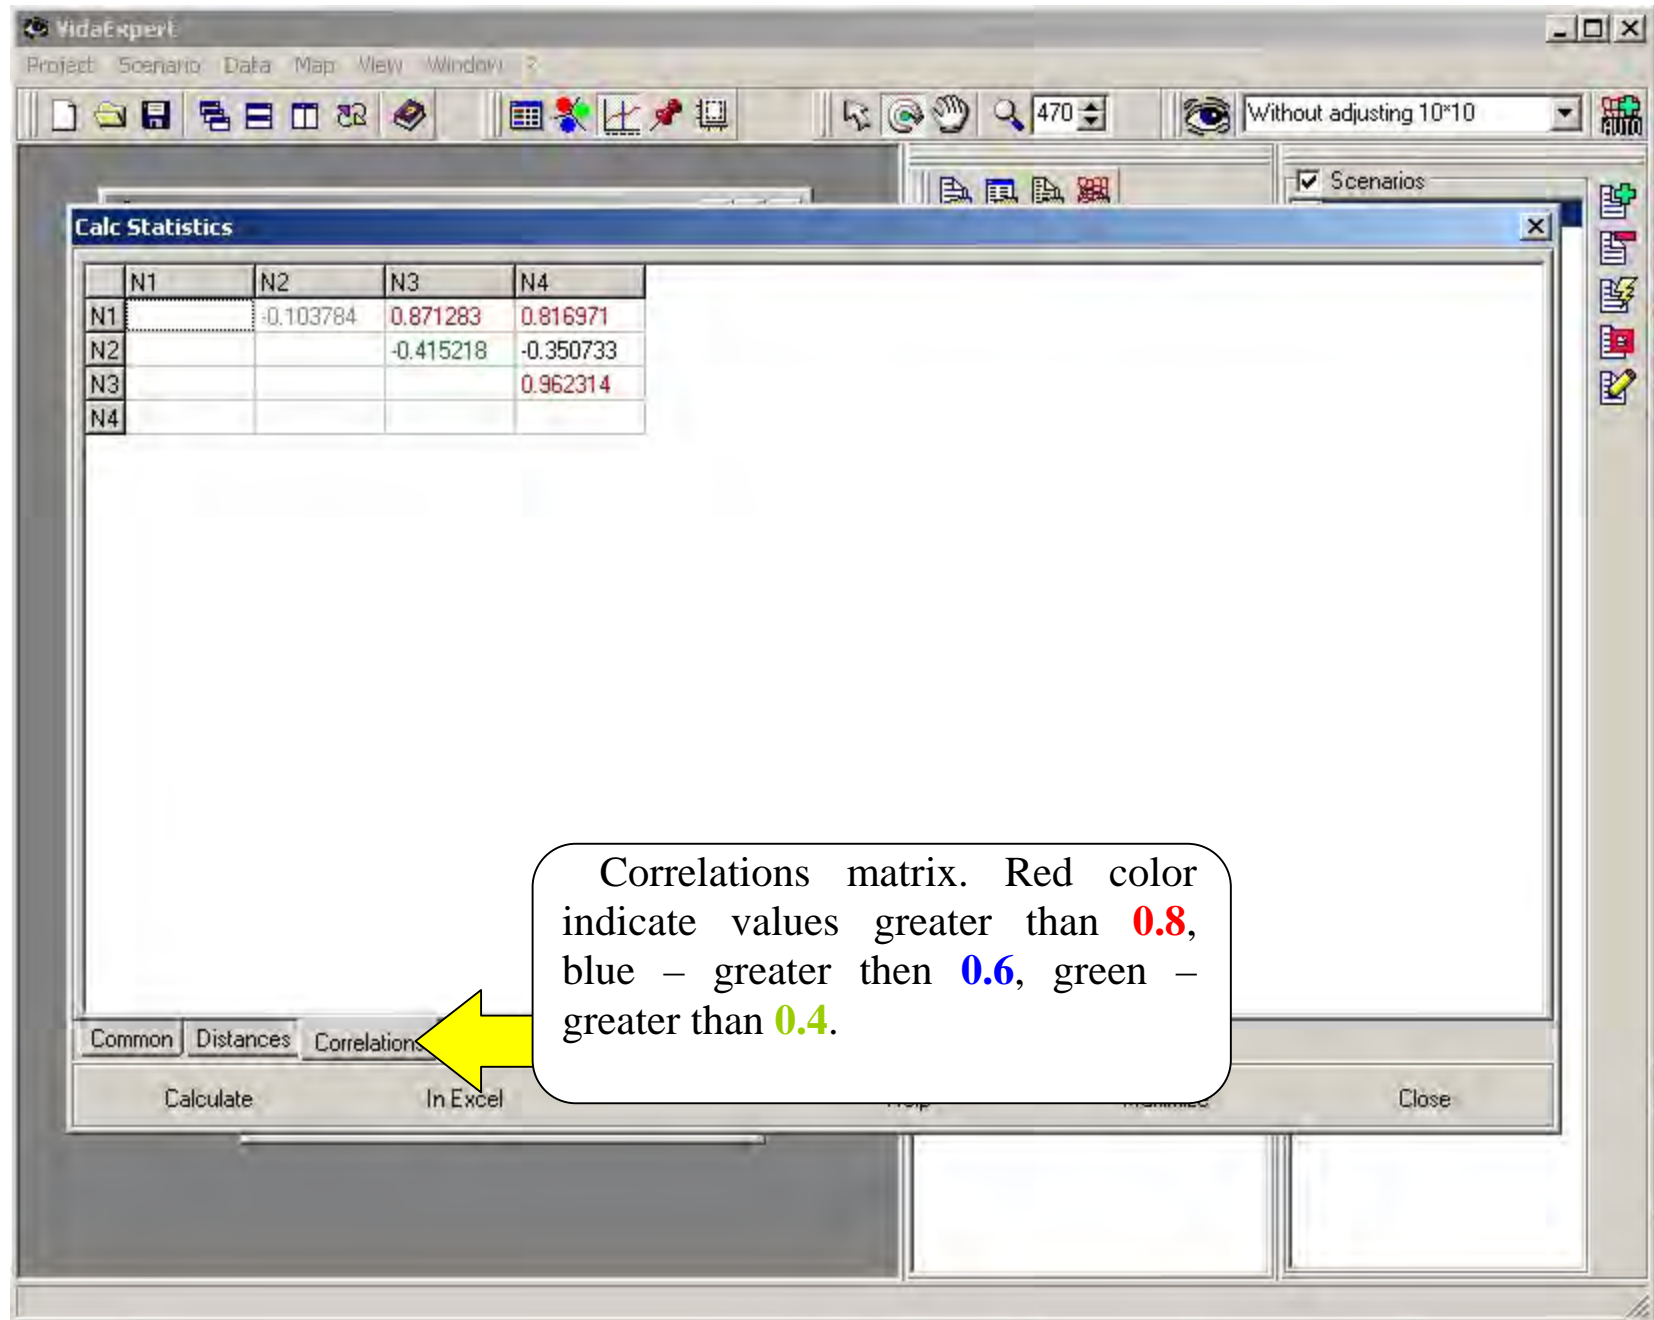



## VIDAEXPERT: DATA ANALYSIS

| Calc Statistics |    |         |           |          |           |           |
|-----------------|----|---------|-----------|----------|-----------|-----------|
| N               | No | Field   | 1         | 2        | 3         | 4         |
|                 |    | Dispers | 0.726151  | 0.231524 | 0.037115  | 0.005210  |
|                 |    | Overall | 0.726151  | 0.957674 | 0.994790  | 1.000000  |
| 1               | 3  | N1      | 0.526813  | 0.363793 | 0.721485  | 0.263784  |
| 2               | 4  | N2      | -0.250294 | 0.929538 | -0.240373 | -0.124630 |
| 3               | 1  | N3      | 0.581995  | 0.013402 | -0.138809 | -0.801146 |
| 4               | 2  | N4      | 0.566659  | 0.058602 | -0.634360 | 0.522542  |

  

|           |           |              |     |            |     |
|-----------|-----------|--------------|-----|------------|-----|
| Common    | Distances | Correlations | PCA | Histograms | Obj |
| Calculate |           | In Excel     |     |            |     |

First line - eigen values of the corresponding vector.

Second line – overall contribution in summary dispersion. From this you can determine **effective linear dimension** of the dataset.

In this example **Iris** dataset is 2D dimensional with accuracy 0.05 and 3D dimensional with accuracy 0.01.

Principal components analysis. Coordinates of principal vectors are shown. Red color indicate the maximum value. Green – several big values.

**Tip:** print the table in Excel to plot different diagrams.

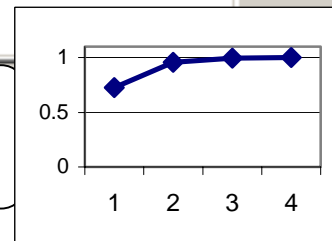

## VIDAEXPERT: DATA ANALYSIS

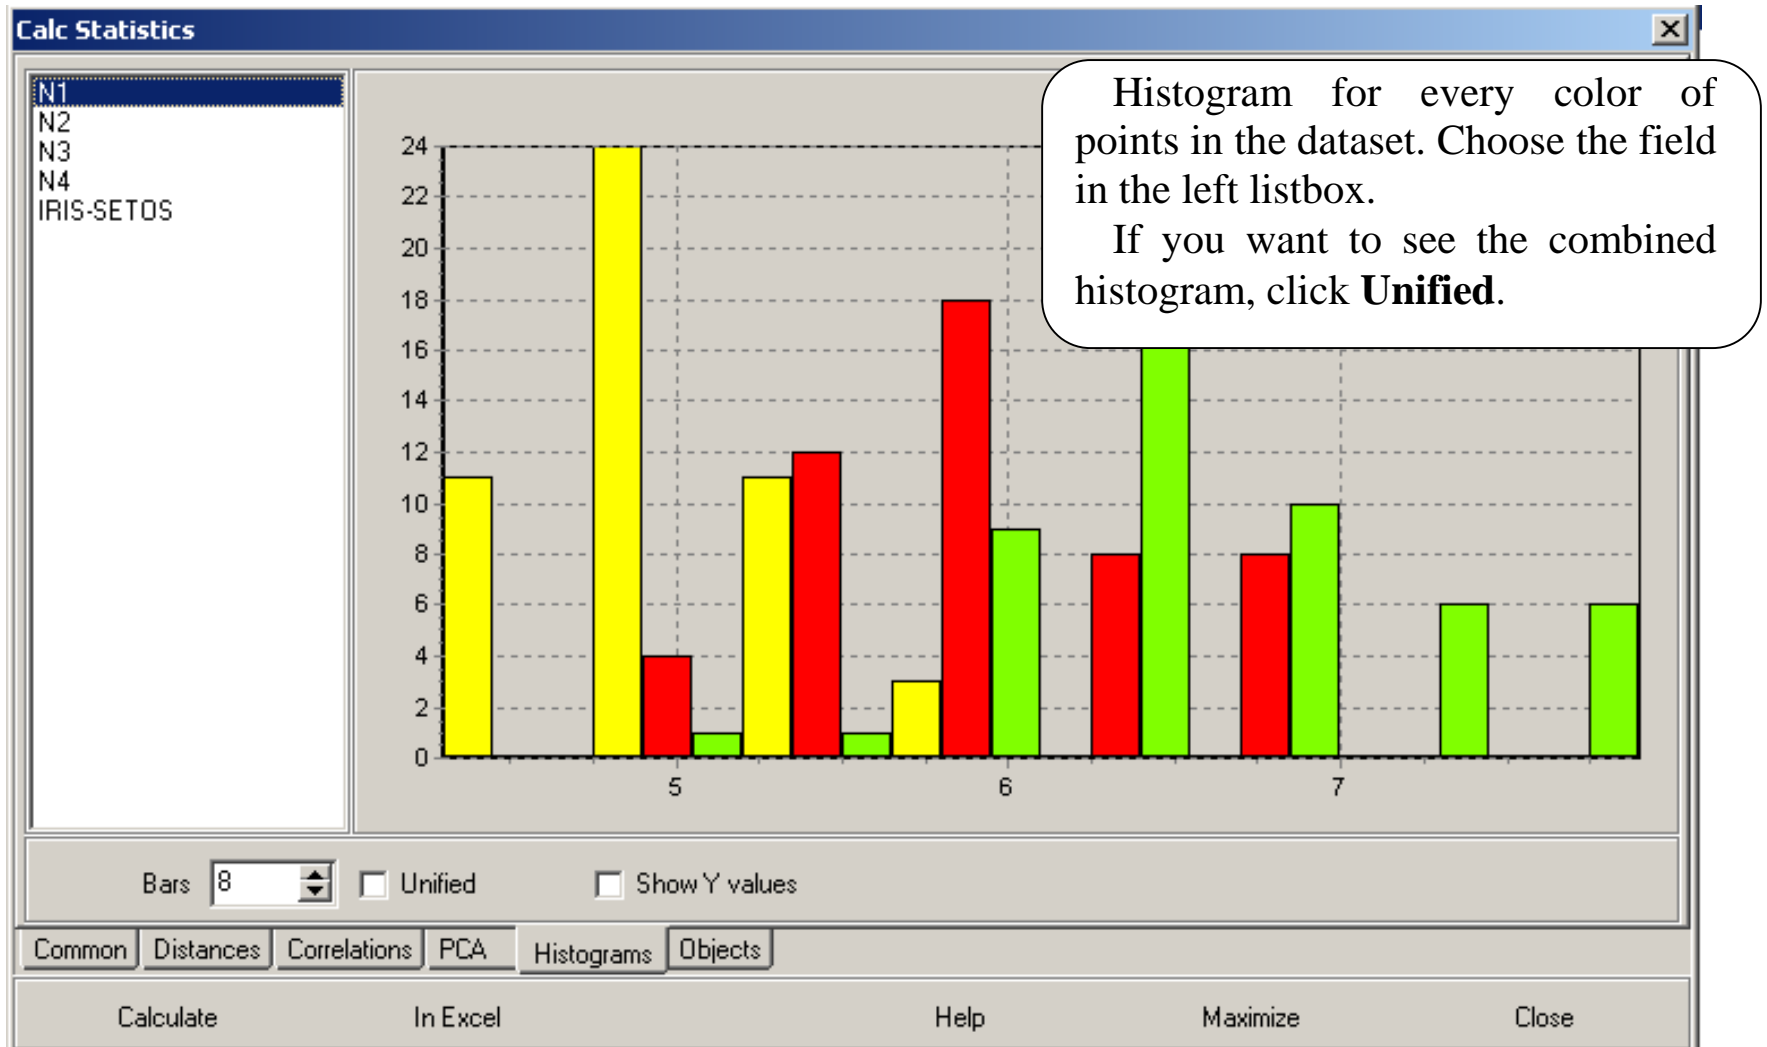

## VIDAEXPERT: DATA ANALYSIS

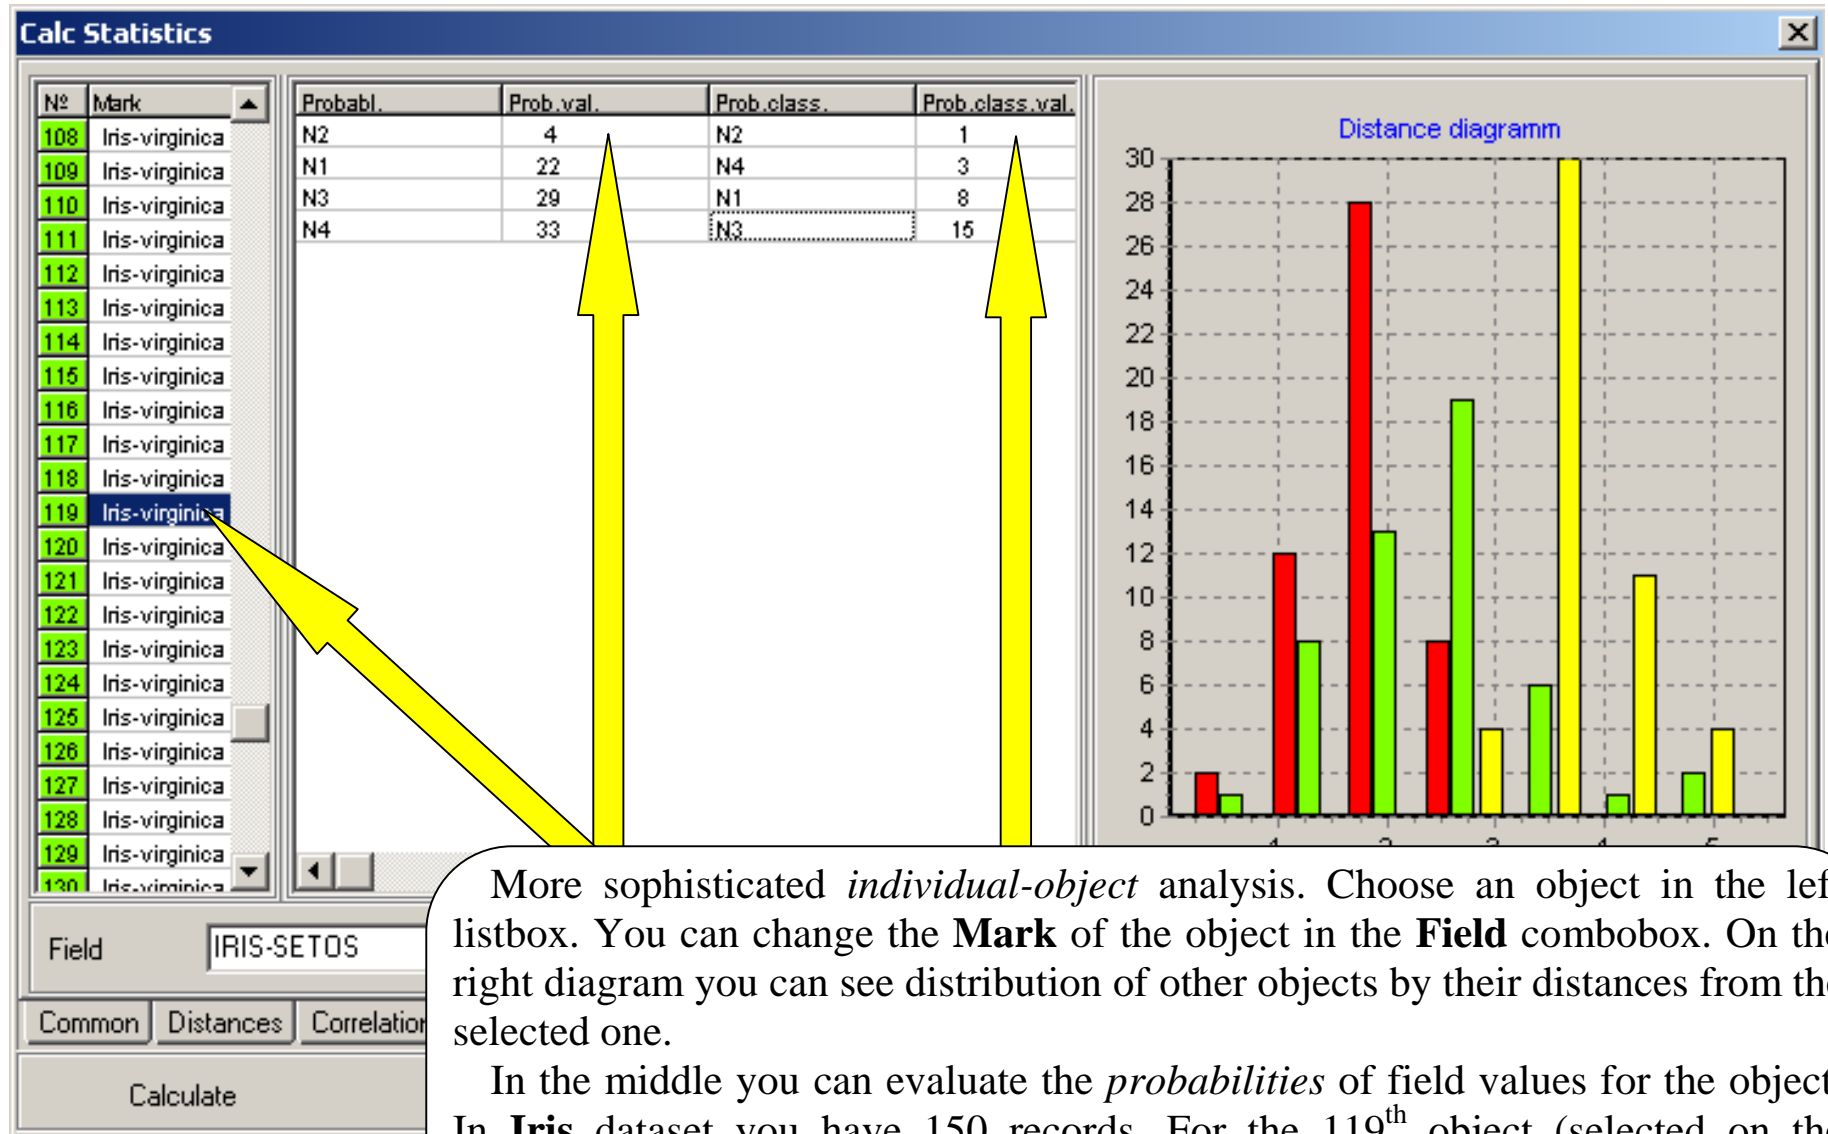

More sophisticated *individual-object* analysis. Choose an object in the left listbox. You can change the **Mark** of the object in the **Field** combobox. On the right diagram you can see distribution of other objects by their distances from the selected one.

In the middle you can evaluate the *probabilities* of field values for the object. In **Iris** dataset you have 150 records. For the 119<sup>th</sup> object (selected on the picture) you have probability of N2 field = 4/150, and probability of N2 in the same class = 1/150. It means that there are only 4 objects (including 119th) in the dataset with value of N2 in the same interval as the 119<sup>th</sup> object has. And only 119<sup>th</sup> object has this value of N2 in it's class (green).

## VIDAEXPERT: DATA ANALYSIS

The screenshot shows the VIDAEXPERT software interface. The main window is titled "VidaExpert - [Map - Map002]". The menu bar includes "Project", "Scenario", "Data", "Map", "View", and "Window". The toolbar contains various icons for file operations and analysis. A yellow arrow points to the "Data analysis" icon in the toolbar, labeled "Data analysis dialog".

The "Data analysis" dialog box is open, showing the "Object analysis" tab. The "Clustering" sub-tab is selected. The "Method" is set to "K-Means" and the "Number of clusters" is set to 3. The "Clusters colors" section shows three clusters with their respective colors and statistics:

| Cluster | Color | Objects | Deviation |
|---------|-------|---------|-----------|
| 1       | Blue  | 52      | 0.91303   |
| 2       | Green | 49      | 0.99429   |
| 3       | Red   | 48      | 1.01319   |

The "Class-class deviation" is 0.973007. The "Analyze" button is highlighted. The "Remember colors" checkbox is checked. The "Numbers in table" and "Distances in table" checkboxes are also checked. The "Close" button is visible.

The "Map" panel shows a scatter plot of data points colored according to the clustering results. The points are grouped into three clusters: blue, green, and red. The map panel also shows the "Colorings" section with checkboxes for "Selections", "Axis X", "Axis Y", and "Axis Z", all of which are checked. The "Not draw all" checkbox is unchecked.

On Clustering tabsheet select method of clustering, number of clusters (not for all methods) and click **Analyze**. You will see the results on the **Map** panel.

Here you see the colors of the clusters, number of objects in every cluster and interclass deviation value (compactness).

**Cancel** will cancel the clustering.  
**Remember colors** will assign for every point it's current color (result of clustering).  
**Numbers in table** will put information about cluster's numbers in the datatable.  
**Distances in table** will put information about distances from the **centroids** in the datatable.



## VIDAEXPERT: DATA ANALYSIS

The screenshot shows the VidaExpert software interface. The main window displays a table of data with columns N1, N2, N3, N4, IRIS-SETOS, and Class. The table is color-coded by cluster number. A yellow arrow points to the 'Numbers in table' button in the 'Object analysis' dialog. The dialog also shows the 'Clustering' tab with 'K-Means' selected and 'Number of clusters' set to 3. The 'Clusters colors' section shows three clusters with their respective colors and statistics.

Click this to switch between **Map** and **Table** panels.

|    | N1  | N2  | N3  | N4  | IRIS-SETOS      | Class |
|----|-----|-----|-----|-----|-----------------|-------|
| 41 | 4.5 | 2.3 | 1.3 | 0.3 | Iris-setosa     | 2     |
| 42 | 4.4 | 3.2 | 1.3 | 0.2 | Iris-setosa     | 2     |
| 43 | 5   | 3.5 | 1.6 | 0.6 | Iris-setosa     | 2     |
| 44 | 5.1 | 3.8 | 1.9 | 0.4 | Iris-setosa     | 2     |
| 45 | 4.8 | 3   | 1.4 | 0.3 | Iris-setosa     | 2     |
| 46 | 5.1 | 3.8 | 1.6 | 0.2 | Iris-setosa     | 2     |
| 47 | 4.6 | 3.2 | 1.4 | 0.2 | Iris-setosa     | 2     |
| 48 | 5.3 | 3.7 | 1.5 | 0.2 | Iris-setosa     | 2     |
| 49 | 5   | 3.3 | 1.4 | 0.2 | Iris-setosa     | 2     |
| 50 | 7   | 3.2 | 4.7 | 1.4 | Iris-versicolor | 3     |
| 51 | 6.4 | 3.2 | 4.5 | 1.5 | Iris-versicolor | 3     |
| 52 | 6.9 | 3.1 | 4.9 | 1.5 | Iris-versicolor | 3     |
| 53 | 5.5 | 2.3 | 4   | 1.3 | Iris-versicolor | 1     |
| 54 | 6.5 | 2.8 | 4.6 | 1.5 | Iris-versicolor | 1     |
| 55 | 5.7 | 2.8 | 4.5 | 1.5 | Iris-versicolor | 1     |
| 56 | 6.3 | 3.3 | 4.7 | 1.5 | Iris-versicolor | 1     |
| 57 | 4.9 | 2.4 | 3.6 | 1   | Iris-versicolor | 1     |
| 58 | 6.6 | 2.9 | 4.4 | 1.4 | Iris-versicolor | 1     |
| 59 | 5.2 | 2.7 | 3.9 | 1.4 | Iris-versicolor | 1     |
| 60 | 5   | 2   | 3.5 | 1   | Iris-versicolor | 1     |
| 61 | 5.9 | 3   | 4.2 | 1.5 | Iris-versicolor | 1     |
| 62 | 6   | 2.2 | 3.5 | 1   | Iris-versicolor | 1     |
| 63 | 6.1 | 2.9 | 4.7 | 1.4 | Iris-versicolor | 1     |
| 64 | 5.6 | 2.9 | 4.3 | 1.4 | Iris-versicolor | 1     |
| 65 | 6.7 | 3.1 | 4.7 | 1.4 | Iris-versicolor | 1     |
| 66 | 5.6 | 3   | 4.5 | 1.5 | Iris-versicolor | 1     |
| 67 | 5.8 | 2.7 | 4.1 | 1   | Iris-versicolor | 1     |
| 68 | 6.2 | 2.2 | 4.5 | 1.5 | Iris-versicolor | 1     |
| 69 | 5.6 | 2.5 | 3.9 | 1.1 | Iris-versicolor | 1     |

You can see records colored accordingly to the cluster number.

If you have clicked the **Numbers in table** button, you will see the numbers of clusters.

**Tip:** right-click on the table and print the table in Excel worksheet or CSV file for the further analysis.

**Object analysis**

Clustering | Values analysis | LDA | LR

Properties

Method: K-Means | Number of clusters: 3

Clusters colors

| Cluster | Color | Statistics |
|---------|-------|------------|
| 1       | Blue  | 52/0.91303 |
| 2       | Green | 49/0.99429 |
| 3       | Red   | 48/1.01319 |

Class-class deviation = 0.973007

Analyze | Cancel

Numbers in table | Distances in table

Remember colors | Close

Colorings

- ☒ Selections
- ☒ Axis X
- ☒ Axis Y
- ☒ Axis Z
- ☐ Not draw all

## VIDAEXPERT: DATA ANALYSIS

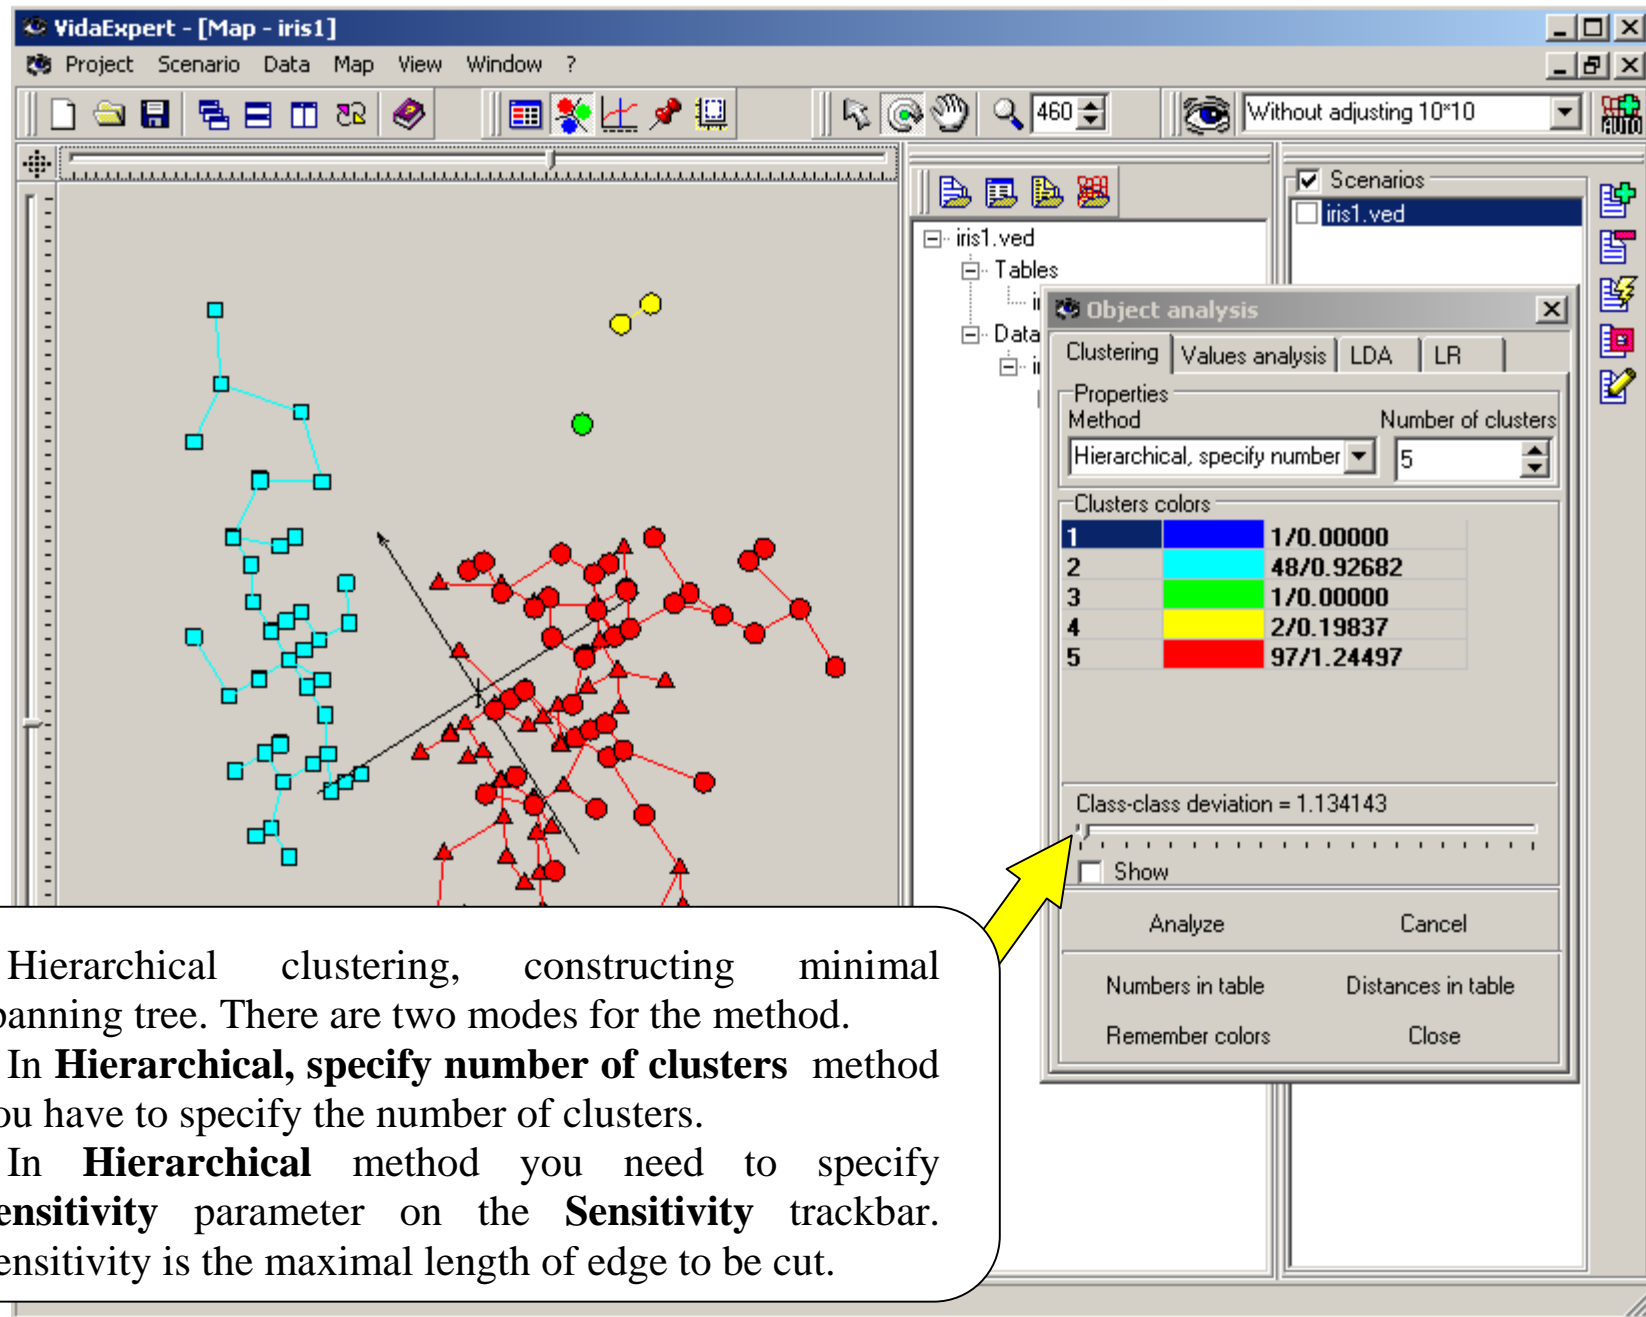

Hierarchical clustering, constructing minimal spanning tree. There are two modes for the method.

In **Hierarchical, specify number of clusters** method you have to specify the number of clusters.

In **Hierarchical** method you need to specify **Sensitivity** parameter on the **Sensitivity** trackbar. Sensitivity is the maximal length of edge to be cut.

## VIDAEXPERT: DATA ANALYSIS

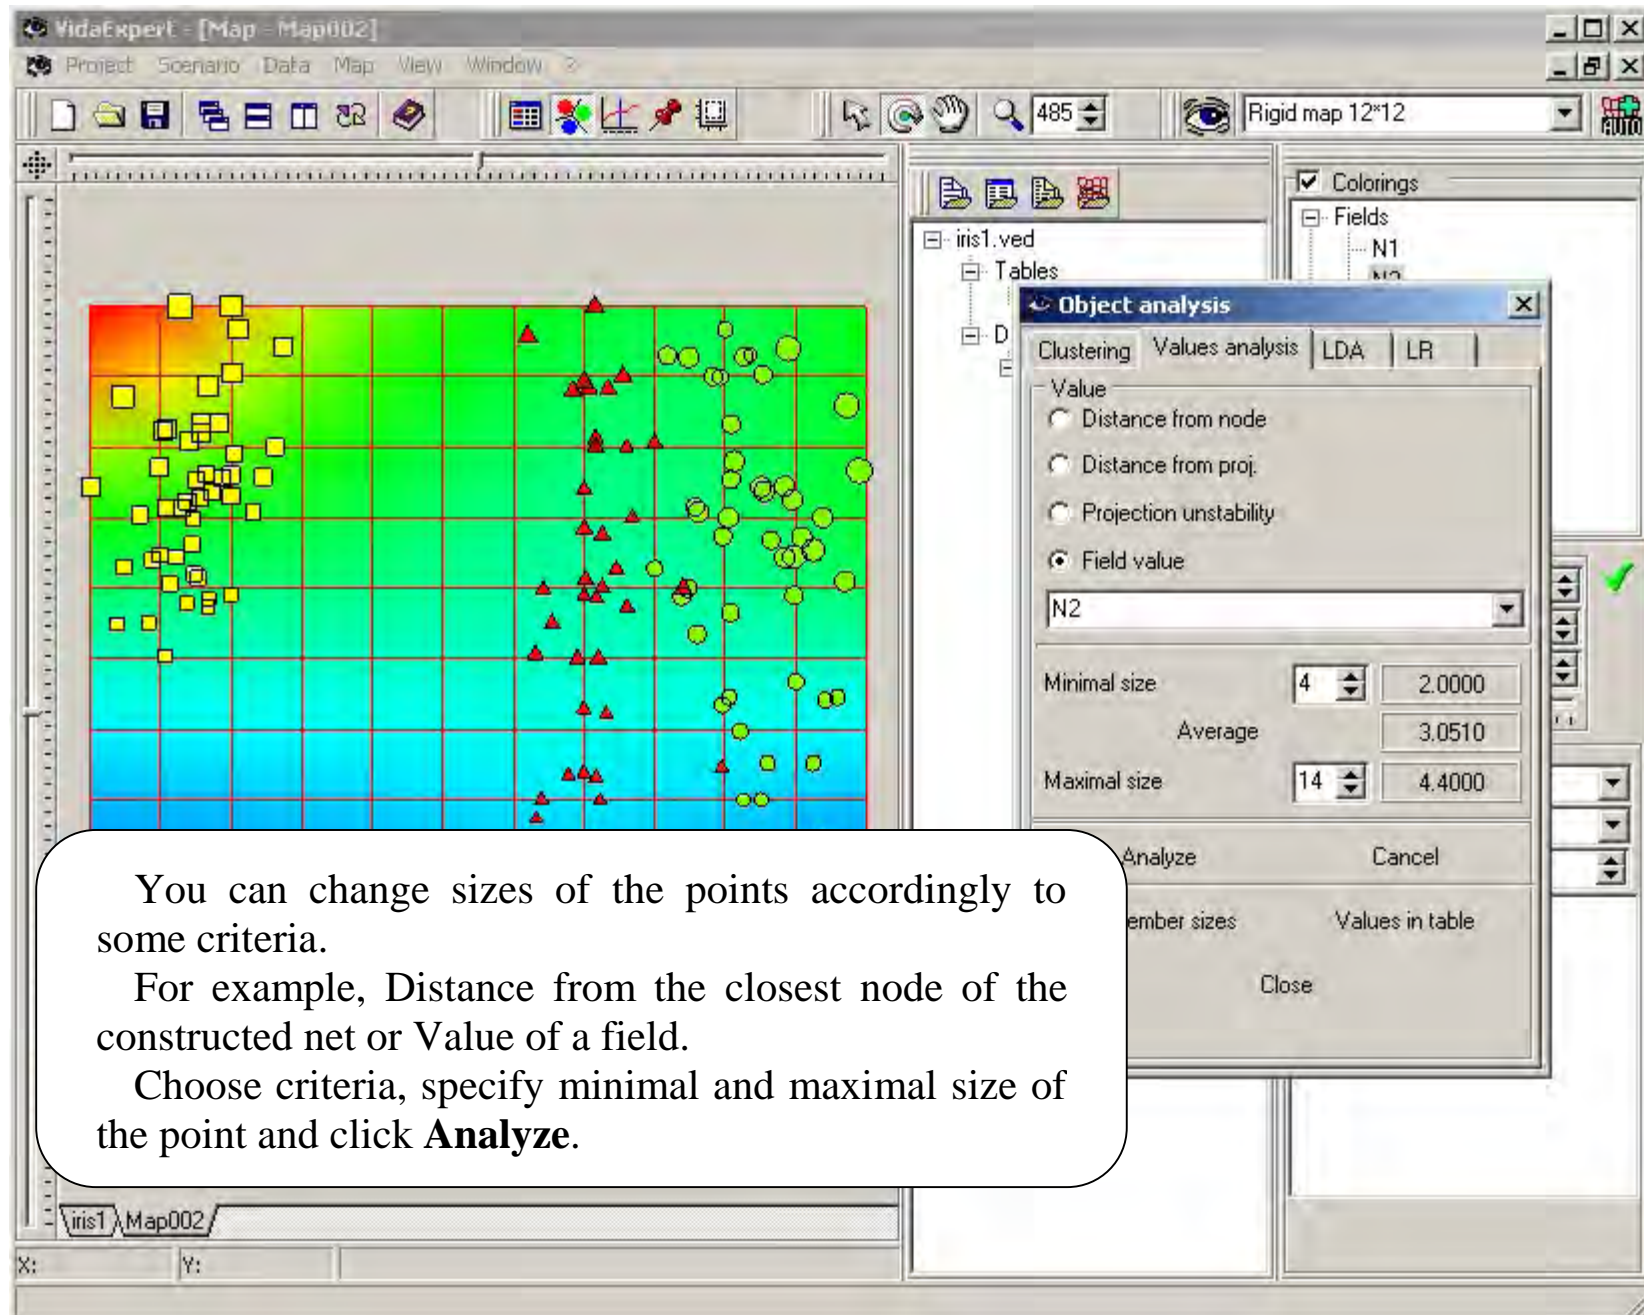

## VIDAEXPERT: DATA ANALYSIS

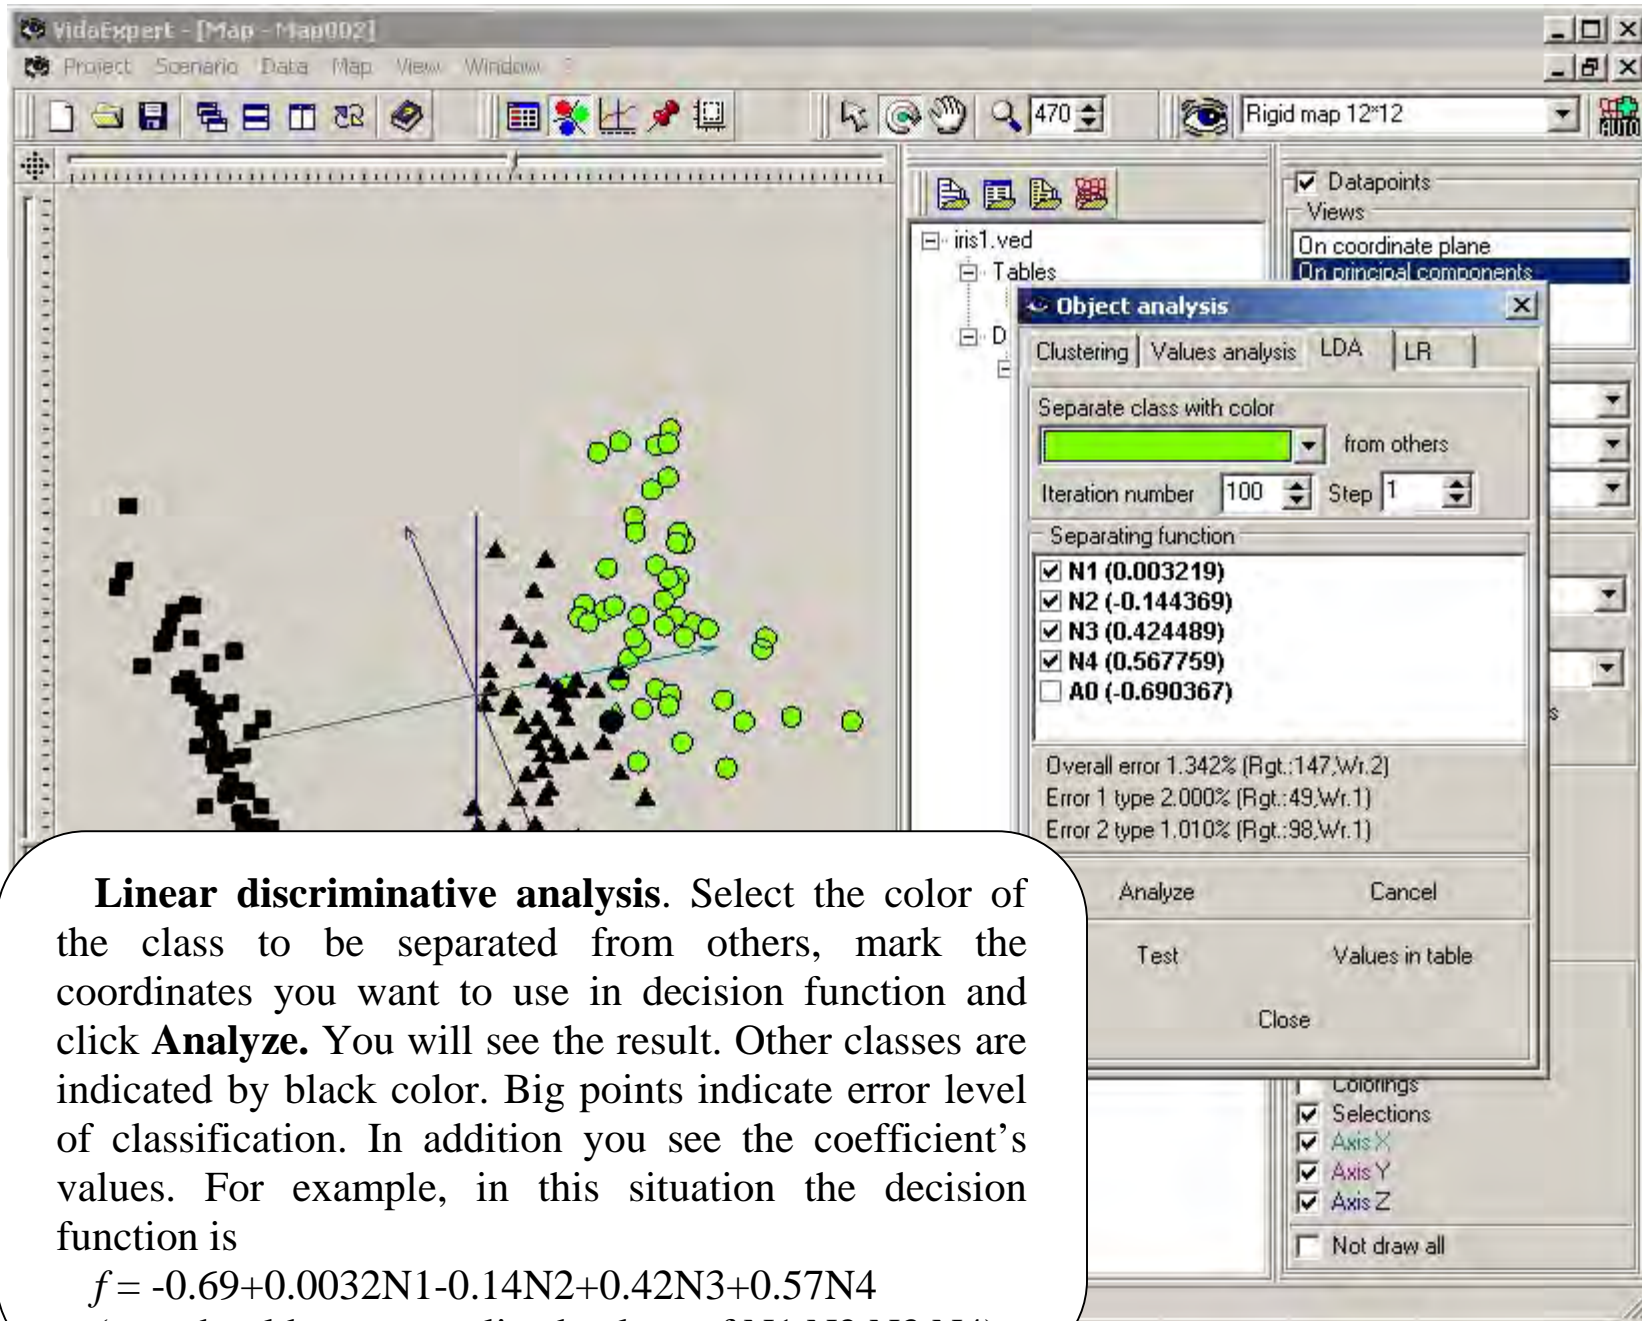



## VIDAEXPERT: DATA ANALYSIS

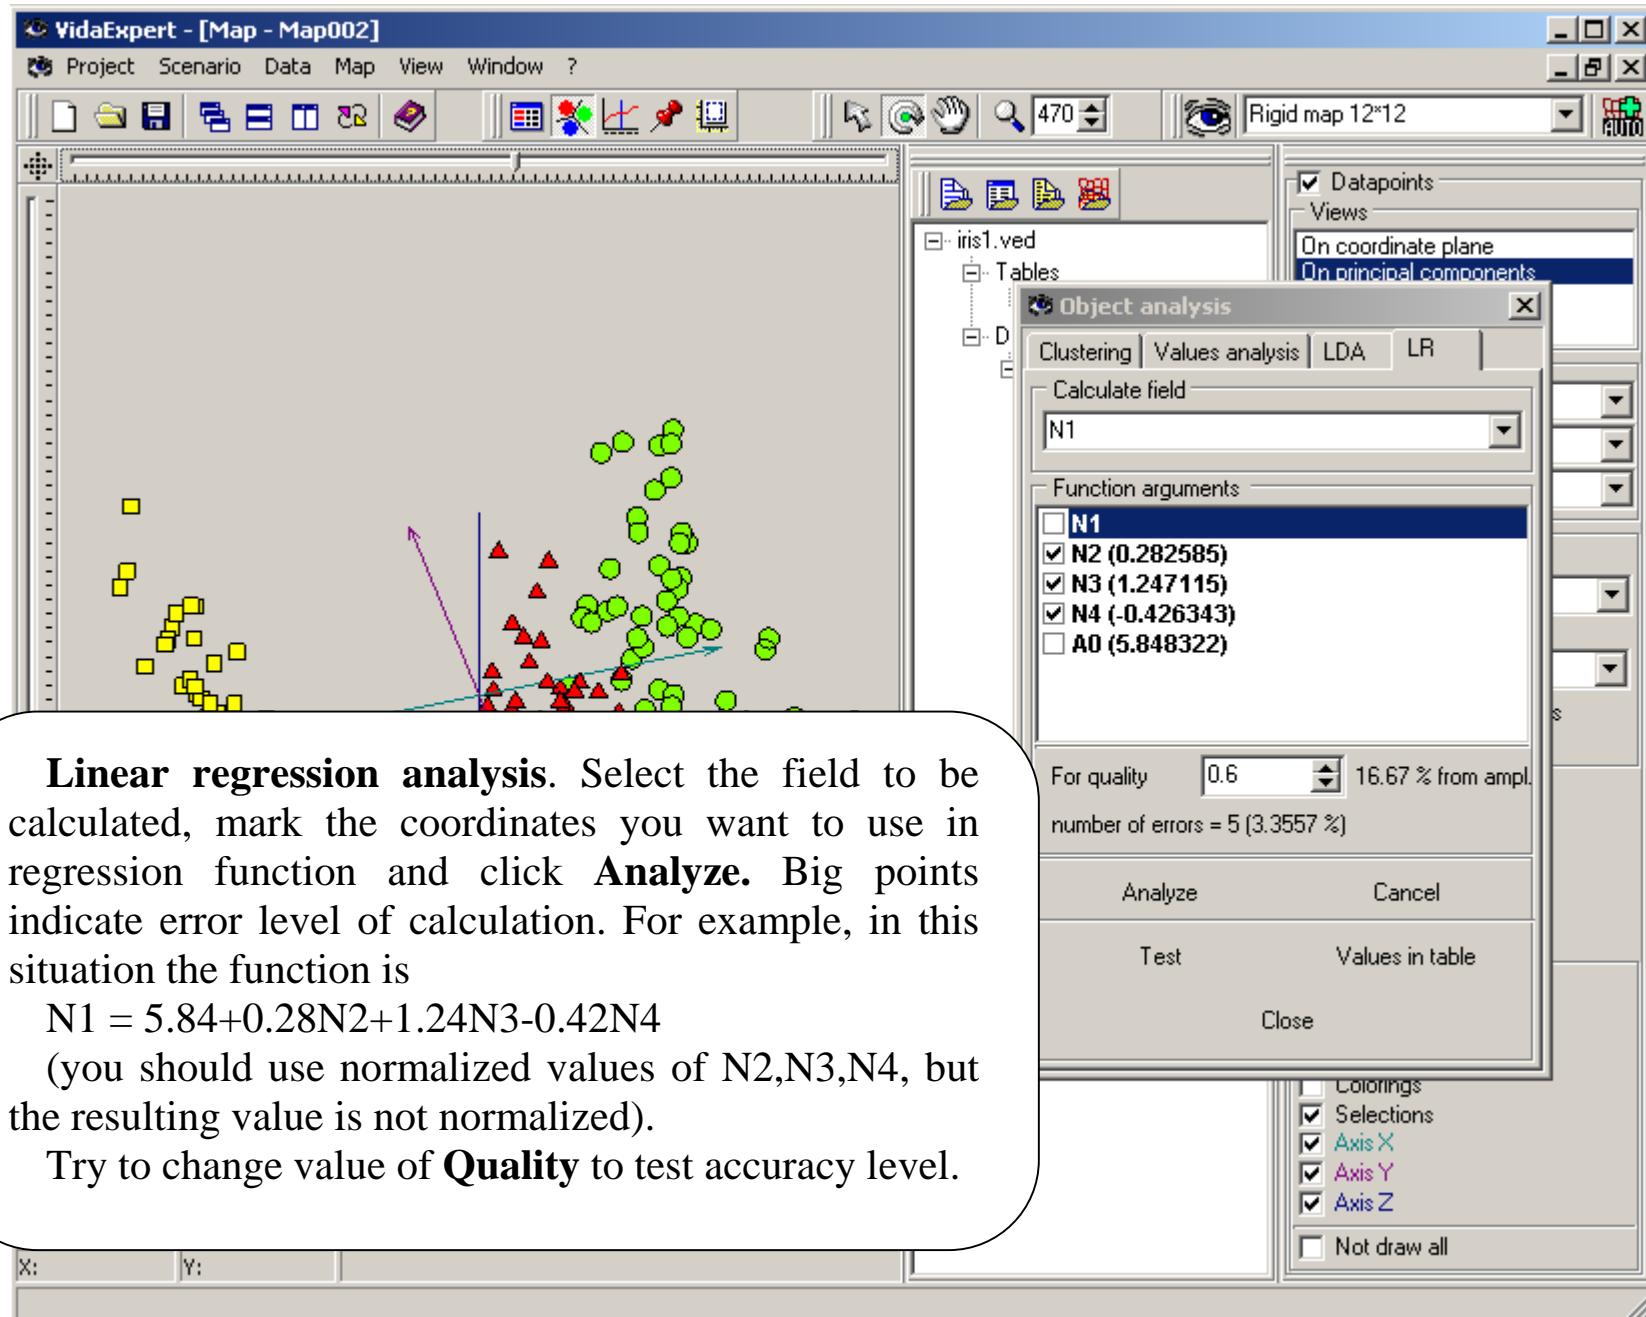

## VIDAEXPERT: DATA ANALYSIS

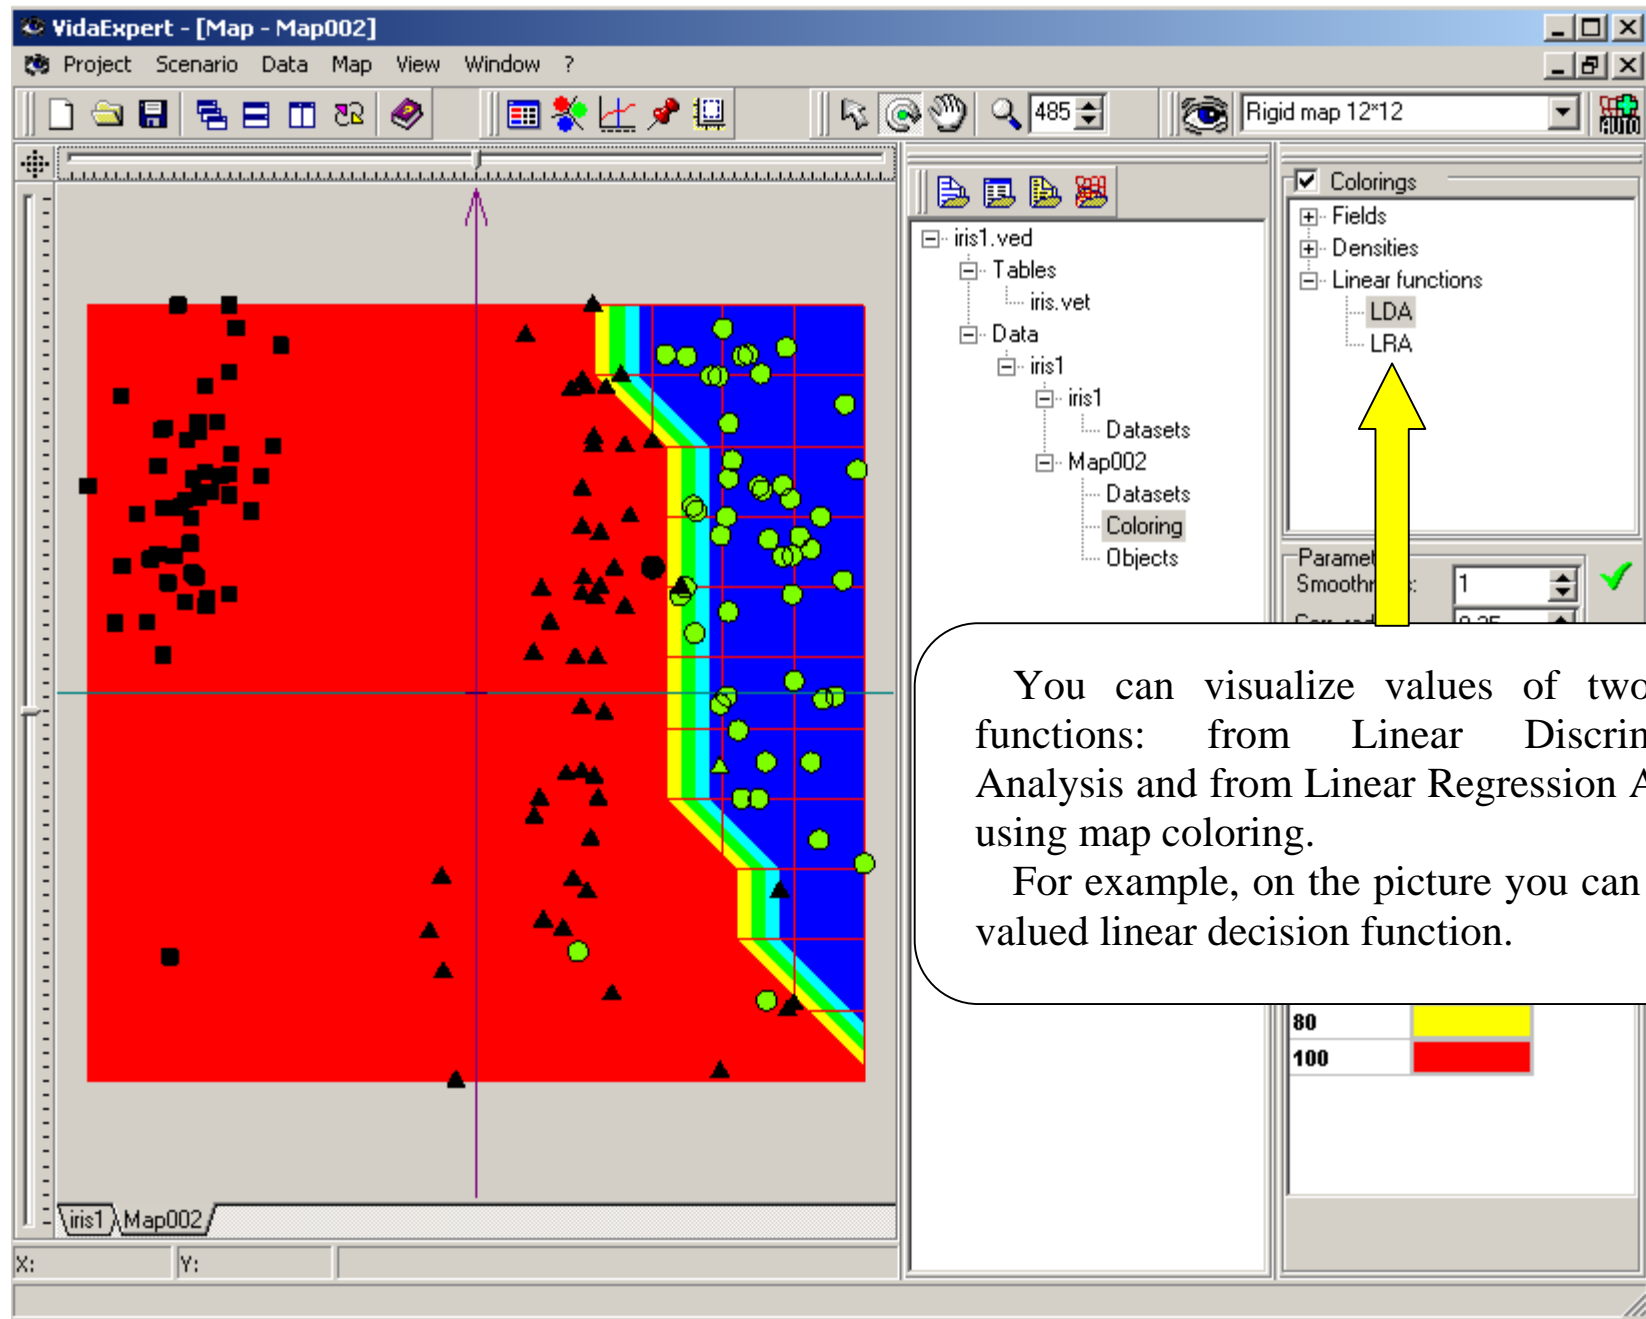

## VIDAEXPERT: DATA ANALYSIS

The screenshot displays the VidaExpert software interface. The main window is titled "VidaExpert - [Map - Map002]". The menu bar includes "Project", "Scenario", "Data", "Map", "View", and "Window". The toolbar contains various icons for file operations, data manipulation, and map navigation. The central map area shows a grid of data points represented by yellow squares, red triangles, and green circles. A dashed black rectangle highlights a specific region of the map. The right sidebar contains a "Selection..." dialog box with a "Marks" section. The "Marks" section lists several options: N1, N2 (checked), N3, N4, and IRIS-SETOS. A yellow arrow points from the "Select" button in the toolbar to the map area, and another yellow arrow points from the "Selection..." dialog box to the "Marks" section. A third yellow arrow points from the dashed black rectangle on the map to the text box below.

Select points by clicking on the **Select** button and dragging the mouse over the map.

You can change properties of displaying of the selected points in the **Selection** dialog.

## VIDAEXPERT: DATA ANALYSIS

VidaExpert - [Таблица - iris.vet]

Project Scenario Data Map View Window ?

Click this to switch between **Map** and **Table** panels.

|    | N1  | N2  | N3  | N4  | IRIS-SETOS      | ED       |
|----|-----|-----|-----|-----|-----------------|----------|
| 46 | 5.1 | 3.8 | 1.6 | 0.2 | Iris-setosa     | 5.356821 |
| 47 | 4.6 | 3.2 | 1.4 | 0.2 | Iris-setosa     | 4.822156 |
| 48 | 5.3 | 3.7 | 1.5 | 0.2 | Iris-setosa     | 5.220302 |
| 49 | 5   | 3.3 | 1.4 | 0.2 | Iris-setosa     | 4.887563 |
| 50 | 7   | 3.2 | 4.7 | 1.4 | Iris-versicolor | 6.494551 |
| 51 | 6.4 | 3.2 | 4.5 | 1.5 | Iris-versicolor | 6.296136 |
| 52 | 6.9 | 3.1 | 4.9 | 1.5 | Iris-versicolor | 6.515177 |
| 53 | 5.5 | 2.3 | 4   | 1.3 | Iris-versicolor | 5.464298 |
| 54 | 6.5 | 2.8 | 4.6 | 1.5 | Iris-versicolor | 6.105620 |
| 55 | 5.7 | 2.8 | 4.5 | 1.3 | Iris-versicolor | 6.146891 |
| 56 | 6.3 | 3.3 | 4.7 | 1.6 | Iris-versicolor | 6.447575 |
| 57 | 4.9 | 2.4 | 3.3 | 1   | Iris-versicolor | 5.200496 |
| 58 | 6.6 | 2.9 | 4.6 | 1.3 | Iris-versicolor | 6.283410 |
| 59 | 5.2 | 2.7 | 3.9 | 1.4 | Iris-versicolor | 5.598621 |
| 60 | 5   | 2   | 3.5 | 1   | Iris-versicolor | 5.081092 |
| 61 | 5.9 | 3   | 4.2 | 1.5 | Iris-versicolor | 5.951986 |
| 62 | 6   | 2.2 | 4   | 1   | Iris-versicolor | 5.567465 |
| 63 | 6.1 | 2.9 | 4.7 | 1.4 | Iris-versicolor | 6.298330 |
| 64 | 5.6 | 2.9 | 3.6 | 1.3 | Iris-versicolor | 5.572291 |
| 65 | 6.7 | 3.1 | 4.4 | 1.4 | Iris-versicolor | 6.215808 |
| 66 | 5.6 | 3   | 4.5 | 1.5 | Iris-versicolor | 6.165322 |
| 67 | 5.8 | 2.7 | 4.1 | 1   | Iris-versicolor | 5.965612 |
| 68 | 6.2 | 2.2 | 4.5 | 1.5 | Iris-versicolor | 5.642067 |
| 69 | 5.6 | 2.5 | 3.9 | 1.1 | Iris-versicolor | 5.636382 |
| 70 | 5.9 | 3.2 | 4.8 | 1.8 | Iris-versicolor | 6.340897 |
| 71 | 6.1 | 2.8 | 4   | 1.3 | Iris-versicolor | 5.791332 |
| 72 | 6.3 | 2.5 | 4.9 | 1.5 | Iris-versicolor | 6.122736 |
| 73 | 6.1 | 2.8 | 4.7 | 1.2 | Iris-versicolor | 6.345306 |
| 74 | 6.4 | 2.9 | 4.3 | 1.3 | Iris-versicolor | 6.070074 |

iris.vet

Selection...

Marks

- ☐ N1
- ☒ N2
- ☐ N3
- ☐ N4
- ☐ IRIS-SETOS

Here you can see the selected points as records in the datatable.

iris1.ved

- Tables
  - iris.vet
- Data
  - iris1
    - iris1
      - Datasets
        - Map002



## VIDAEXPERT: DATA ANALYSIS

The screenshot displays the VidaExpert software interface. The main window is titled "VidaExpert - [Map - Map002]". The menu bar includes "Project", "Scenario", "Data", "Map", "View", and "Window". The toolbar contains various icons for file operations and data analysis. A yellow arrow points to the "Annotation" icon in the toolbar, which is labeled "Annotation dialog".

The "Annotation" dialog box is open, showing the following options:

- Points:**
  - ☐ Randomly selected (with a value of 50 and a percentage sign)
  - ☐ By color
  - ☒ Selected
- Parameters:**
  - Field names:**
    - ☐ N1
    - ☐ N2
    - ☐ N3
    - ☒ N4
    - ☒ IRIS-SETOS
  - ☒ All fields
  - ☐ Max values
  - ☐ Min values
  - ☐ Unexpected features
  - ☐ Unexpected in class
- Depth:** 1
- Font size:** 9
- Max length:** 50

- Buttons:** Apply, Clear, To table, Close

The main map area shows a grid with various data points (yellow squares, red triangles, green circles). Several points are labeled with text boxes containing descriptions such as "1.1/Iris-versicolor", "1.3/Iris-versicolor", "1.7/Iris-virginica", and "1.3/Iris-versicolor".

**You can assign for some points labels with their short description.**  
**In **Annotation** dialog choose which points do you need to label, content of the labels and click **Apply**.**
